# Supplementary material for: The Quantum Hamming Bound in Arbitrary Local Dimension
Source: arXiv:2606.22538 source file (2026-10-05)
Supplement: Supplementary file 1 [file sm-qary_qhb.tex]

\documentclass[aps,prl,onecolumn,10pt,superscriptaddress,nofootinbib,longbibliography]{revtex4}

\usepackage{amsmath,amssymb,amsfonts,amsthm,mathtools,bm}
\usepackage{array}
\usepackage{microtype}
\usepackage{xcolor}
\usepackage[colorlinks=true,citecolor=blue!55!black,linkcolor=blue!55!black,urlcolor=blue!55!black,hypertexnames=false]{hyperref}
\allowdisplaybreaks
\hypersetup{pdftitle={Supplemental Material for The Quantum Hamming Bound in Arbitrary Local Dimension}}
\renewcommand{\thesection}{S\arabic{section}}

\newcommand{\smsection}[2]{%
  \refstepcounter{section}%
  \section*{\thesection.\ #1}%
  \pdfbookmark[1]{\thesection. #1}{#2}%
  \label{#2}%
}

\newtheorem{theorem}{Theorem}

\newtheorem{lemma}[theorem]{Lemma}

\theoremstyle{definition}

\newcommand{\Vol}{V}
\newcommand{\Kraw}{P}
\newcommand{\Lloyd}{L}
\newcommand{\coef}[2]{[x^{#1}]#2}
\newcommand{\wt}{\operatorname{wt}}

\newcommand{\E}{\mathbb E}
\newcommand{\Prob}{\mathbb P}

% Compact Bernstein coefficient tables.
\newcommand{\cform}[1]{$#1$}

\begin{document}

\title{Supplemental Material for ``The Quantum Hamming Bound in Arbitrary Local Dimension''}
\author{Yu-Xuan Zhang}
\affiliation{School of Physics, Nankai University, Tianjin 300071, People's Republic of China}
\author{Jing-Ling Chen}
\affiliation{Theoretical Physics Division, Chern Institute of Mathematics, Nankai University, Tianjin 300071, People's Republic of China}
\date{\today}
\maketitle

This Supplemental Material gives the algebraic details for the reductions used in the Letter.  It begins with the finite Fourier transform on the Hamming group and the quantum linear-programming normalization.  It then isolates the two-center node--edge/Jacobi comparison used in both nonbinary regimes, proves the high-alphabet half-gap at the critical length, and treats the qutrit short, long, and bridge ranges.  The high-alphabet interior and the qutrit long range are proved by Jacobi Rayleigh-quotient bounds followed by scalar rational inequalities.  The qutrit bridge is proved by an exact coefficient-certificate reduction in Sec.~\ref{sec:S6} followed by the affine Stein--tangent positivity argument in Sec.~\ref{sec:S7}; the Bernstein, quotient-remainder, and Sturm ledgers are included in Sec.~\ref{sec:S-cert-appendix} as exact certificate data.

For orientation, the proof has the following route.  Section~\ref{sec:S1} reduces the quantum Hamming bound to sign conditions for a Fourier-side test polynomial.  Section~\ref{sec:S2} shows that, for $Q\ge16$, it is enough to treat the critical length $n=4t+1$; Secs.~\ref{sec:Sjacobi}--\ref{sec:S3} then prove the required half-gap at that length.  The qutrit case is split in Sec.~\ref{sec:S4} into a short Singleton--entropy range, a long positive-Lloyd range, and the remaining bridge.  Sections~\ref{sec:S5}--\ref{sec:S7} handle the bridge by preserving the Hamming prefactor, reducing the overlapping-shell defect to a two-coefficient expression, and proving the resulting expression positive.  Section~\ref{sec:S8} assembles these pieces.

\smsection{The Li--Xing reduction and Fourier normalization}{sec:S1}

The case $t=0$ is immediate, since $\Vol_0^{(Q)}(n)=1$ and $K\le q^n$.
Hence assume $t\ge1$ below.  This section is the $Q=q^2$ analogue of the
Fourier reduction used in the binary endpoint proof~\cite{DegeneracyQHB}; the
only changes are the alphabet parameter and the notation needed later for the
qutrit filter.

Let $Q=q^2$.  A phase-free single-qudit Weyl error label has one zero label and
$Q-1$ nonzero labels.  We work in an abelian label group $A$ of order $Q$ and in
$G=A^n$.  No field structure is used below; only the $Q$-ary Hamming scheme and
its character sums enter.  Write $\wt(\cdot)$ for Hamming weight, and put
\begin{equation}
 B_t^{(Q,n)}=\{x\in G:\wt x\le t\},\qquad
 \Vol_t^{(Q)}(n)=|B_t^{(Q,n)}|=\sum_{j=0}^{t}(Q-1)^j\binom nj.
 \label{eq:S-volume}
\end{equation}
For a center difference $z$ of weight $s$, define the two-ball intersection
\begin{equation}
 c_t^{(Q)}(n,s)=|B_t^{(Q,n)}\cap(B_t^{(Q,n)}+z)|.
 \label{eq:S-c-def}
\end{equation}
It depends only on $s$.

We use the standard $Q$-ary Krawtchouk normalization
\begin{equation}
 \Kraw_i^{(Q)}(s;n)=\sum_{a=0}^{i}(-1)^a(Q-1)^{i-a}
 \binom{s}{a}\binom{n-s}{i-a}.
 \label{eq:S-kraw}
\end{equation}
Equivalently,
\begin{equation}
 \sum_{i=0}^{n}\Kraw_i^{(Q)}(s;n)u^i
 =(1+(Q-1)u)^{n-s}(1-u)^s.
 \label{eq:S-kraw-gen}
\end{equation}
If $\widehat G$ denotes the character group of $G$, then for $\wt z=s$,
\begin{equation}
 \sum_{\wt(\chi)=i}\chi(z)=\Kraw_i^{(Q)}(s;n).
 \label{eq:S-shell-sum}
\end{equation}
Indeed, a nontrivial character coordinate outside the support of $z$ contributes
$Q-1$ after summation, whereas one on the support contributes $-1$.

Define the Lloyd sum
\begin{equation}
 \Lloyd_t^{(Q,n)}(x)=\sum_{j=0}^{t}\Kraw_j^{(Q)}(x;n).
 \label{eq:S-lloyd}
\end{equation}
Let $g=1_{B_t^{(Q,n)}}$ and use the unnormalized Fourier transform
\begin{equation}
 \widehat h(\chi)=\sum_{x\in G}h(x)\overline{\chi(x)},\qquad
 h(z)=Q^{-n}\sum_{\chi\in\widehat G}\widehat h(\chi)\chi(z).
 \label{eq:S-fourier-norm}
\end{equation}
If $\wt(\chi)=i$, then \eqref{eq:S-shell-sum} gives
\begin{equation}
 \widehat g(\chi)=\sum_{j=0}^{t}\Kraw_j^{(Q)}(i;n)=\Lloyd_t^{(Q,n)}(i).
 \label{eq:S-ball-fourier}
\end{equation}
The autocorrelation $A_g(z)=\sum_x g(x)g(x+z)$ equals $c_t^{(Q)}(n,s)$ when
$\wt z=s$, and $\widehat{A_g}(\chi)=|\widehat g(\chi)|^2$.  Fourier inversion and
\eqref{eq:S-shell-sum} therefore give
\begin{equation}
 Q^n c_t^{(Q)}(n,s)
 =\sum_{i=0}^{n}\Lloyd_t^{(Q,n)}(i)^2\Kraw_i^{(Q)}(s;n).
 \label{eq:S-fourier}
\end{equation}
Thus the square of the Lloyd sum is the Fourier-side square of the Hamming ball,
and its distance-space values are exactly the two-center intersection numbers.

Two elementary Lloyd identities will be used later.  Comparing generating
functions in lengths $n$ and $n+1$ gives
\begin{equation}
 \Lloyd_t^{(Q,n+1)}(s)=\Lloyd_t^{(Q,n)}(s)+(Q-1)\Lloyd_{t-1}^{(Q,n)}(s).
 \label{eq:S-lloyd-length}
\end{equation}
For $s\ge1$, summing \eqref{eq:S-kraw-gen} up to degree $t$ is equivalent to
division by $1-u$, hence
\begin{equation}
 \Lloyd_t^{(Q,n)}(s)
 =[u^t](1+(Q-1)u)^{n-s}(1-u)^{s-1}
 =\Kraw_t^{(Q)}(s-1;n-1).
 \label{eq:S-lloyd-shift}
\end{equation}

A direct count gives the same intersection.  On the $s$ separated
coordinates, let $a$ count positions where $y_i=0$, let $b$ count positions where
$y_i=z_i$, and let $c$ count positions where $y_i\notin\{0,z_i\}$.  Outside the
support of $z$, let $d$ be the number of nonzero coordinates.  Then
\begin{equation}
 c_t^{(Q)}(n,s)=
 \sum_{\substack{a,b,c,d\ge0:\ a+b+c=s\\ b+c+d\le t,\ a+c+d\le t}}
 \binom{s}{a,b,c}(Q-2)^c\binom{n-s}{d}(Q-1)^d.
 \label{eq:S-c-explicit}
\end{equation}
In particular, $c_t^{(Q)}(n,s)=0$ for $s>2t$.

We next recall the Li--Xing linear-programming bound in the present
normalization.  Let
\begin{equation}
 F(x)=\sum_{i=0}^{n} f_i\Kraw_i^{(Q)}(x;n),\qquad T=\{0,1,\ldots,n\}.
 \label{eq:S-LX-polynomial}
\end{equation}
If $S$ is a nonempty subset of $\{0,\ldots,d-1\}$, if
\begin{equation}
 f_i>0\quad(i\in S),\qquad f_i\ge0\quad(i\in T),
 \label{eq:S-LX-coeff-cond}
\end{equation}
and if
\begin{equation}
 F(x)\le0\qquad (x\in T\setminus S),
 \label{eq:S-LX-sign-cond}
\end{equation}
then every exact $q$-ary $((n,K,d))$ quantum subspace code satisfies
\begin{equation}
 K\le q^{-n}\max_{x\in S}\frac{F(x)}{f_x}.
 \label{eq:S-LX-bound}
\end{equation}
This is Li--Xing's quantum LP theorem~\cite{LiXing2009} written for the
$Q=q^2$ Hamming scheme.

Apply \eqref{eq:S-LX-bound} first to the raw Lloyd square.  Let $d\ge2t+1$ and
choose
\begin{equation}
 S=\{0,1,\ldots,2t\},\qquad f_i=\Lloyd_t^{(Q,n)}(i)^2.
 \label{eq:S-raw-choice}
\end{equation}
This set is contained in $\{0,\ldots,d-1\}$ for both possible minimum
distances $d=2t+1$ and $d=2t+2$, and also for larger $d$.  If $d$ is larger,
the shells $2t<s<d$ are simply left in $T\setminus S$; their distance-space value is
zero by two-ball disjointness, so the Li--Xing sign condition holds there with
equality.  The Fourier coefficients are nonnegative.  In the regimes where we
use this raw choice, the later zero-location estimates place the Lloyd response
on the positive branch throughout $S$, so $f_i>0$ for $i\in S$.  By
\eqref{eq:S-fourier},
\begin{equation}
 F(s)=Q^n c_t^{(Q)}(n,s).
 \label{eq:S-lloyd-physical-value}
\end{equation}
Therefore $F(s)=0$ for $s>2t$ by the two-ball disjointness just noted, and the
nonoverlapping-shell sign condition \eqref{eq:S-LX-sign-cond} holds with equality.  At the
origin the two balls coincide, so
\begin{equation}
 F(0)=Q^n\Vol_t^{(Q)}(n),\qquad f_0=\Vol_t^{(Q)}(n)^2,
 \label{eq:S-raw-origin}
\end{equation}
and consequently
\begin{equation}
 \frac{F(0)}{f_0}=\frac{Q^n}{\Vol_t^{(Q)}(n)}.
 \label{eq:S-lloyd-normalization}
\end{equation}
For $1\le s\le2t$, the condition that the ratio at the origin dominate the
ratio at $s$ is
\begin{equation}
 R_{Q;n,t}(s):=\frac{\Vol_t^{(Q)}(n)c_t^{(Q)}(n,s)}
 {\Lloyd_t^{(Q,n)}(s)^2}\le1.
 \label{eq:S-LP}
\end{equation}
Equivalently,
\begin{equation}
 \Lloyd_t^{(Q,n)}(s)^2-\Vol_t^{(Q)}(n)c_t^{(Q)}(n,s)\ge0.
 \label{eq:S-lloyd-two-center-coeff}
\end{equation}
Thus \eqref{eq:S-LP} for every $1\le s\le2t$ places the maximum in
\eqref{eq:S-LX-bound} at $s=0$, and gives
\begin{equation}
 K\le q^{-n}\frac{Q^n}{\Vol_t^{(Q)}(n)}=\frac{q^n}{\Vol_t^{(Q)}(n)},
 \label{eq:S-qLP-normalization}
\end{equation}
which is the $q$-ary quantum Hamming bound.

For the qutrit bridge we use the same LP normalization with a nonnegative
Fourier-side filter.  The following division-free form is the one used later.
For a radial Fourier-positive polynomial
\begin{equation}
 F_f(s)=\sum_{i=0}^{n} f_i\Kraw_i^{(Q)}(s;n),\qquad f_i\ge0,
 \label{eq:S-physical-f}
\end{equation}
write $f(0):=F_f(0)$ for the distance-space value at the origin and keep subscripts
for Fourier coefficients.  Suppose that $f_0>0$ and that
\begin{equation}
 \frac{f(0)}{f_0}=\frac{Q^n}{\Vol_t^{(Q)}(n)},
 \qquad
 f_s-\frac{\Vol_t^{(Q)}(n)}{Q^n}F_f(s)\ge0
 \quad(1\le s\le2t),
 \label{eq:S-trace-shell-form}
\end{equation}
and that $F_f(s)\le0$ for $s>2t$.  Apply \eqref{eq:S-LX-bound} with
\begin{equation}
 S_f=\{0\}\cup\{1\le s\le2t: f_s>0\}.
 \label{eq:S-filter-Sf}
\end{equation}
Then $S_f\subseteq\{0,\ldots,d-1\}$ because $d\ge2t+1$, the coefficient
conditions in \eqref{eq:S-LX-coeff-cond} hold by construction, and the sign
condition on $T\setminus S_f$ is as follows.  If $1\le s\le2t$ and $f_s=0$,
then \eqref{eq:S-trace-shell-form} gives $F_f(s)\le0$; if $s>2t$, the assumed
tail sign gives the same conclusion.  For $s\in S_f$, the inequality
\eqref{eq:S-trace-shell-form} gives
\begin{equation}
 \frac{F_f(s)}{f_s}\le \frac{Q^n}{\Vol_t^{(Q)}(n)}
 =\frac{f(0)}{f_0}.
\end{equation}
Thus the Li--Xing maximum is at most the origin value, and
\eqref{eq:S-qLP-normalization} follows.  For the raw Lloyd square,
\eqref{eq:S-trace-shell-form} is exactly \eqref{eq:S-lloyd-two-center-coeff}; in
the qutrit bridge, Secs.~\ref{sec:S5}--\ref{sec:S7} verify the overlapping-shell
inequality and the nonoverlapping-shell signs for the filtered square while preserving
the origin ratio.

In the rest of this Supplemental Material, the raw Lloyd square is used for the
high-alphabet regime and for the qutrit long range.  The filtered Lloyd square
is used only in the qutrit bridge.  In both cases the goal is to keep the origin
ratio equal to the Hamming prefactor and to verify the required shell signs.

\smsection{High-alphabet length reduction}{sec:S2}

Assume $Q\ge16$ and $n\ge4t+1$.  This section proves that the two-center ratio does not increase with length; hence the worst length is $n=4t+1$.  The argument is a ratio comparison: the volume, the two-ball intersection, and the Lloyd value all obey the same one-step length recurrence, and the three induced ratios satisfy a sandwich inequality.

\begin{lemma}[Length recurrences]
\label{lem:S-length-rec}
For fixed $Q,t,s$, comparing lengths $m$ and $m+1$ with the two centers equal in the added coordinate gives
\begin{align}
 \Vol_t^{(Q)}(m+1)&=\Vol_t^{(Q)}(m)+(Q-1)\Vol_{t-1}^{(Q)}(m),
 \label{eq:S-V-length}\\
 c_t^{(Q)}(m+1,s)&=c_t^{(Q)}(m,s)+(Q-1)c_{t-1}^{(Q)}(m,s),
 \label{eq:S-c-length}\\
 \Lloyd_t^{(Q,m+1)}(s)&=\Lloyd_t^{(Q,m)}(s)+(Q-1)\Lloyd_{t-1}^{(Q,m)}(s).
 \label{eq:S-L-length}
\end{align}
\end{lemma}

\begin{proof}
For volumes, split on whether the added coordinate is zero or nonzero.  The nonzero case has $Q-1$ choices and uses radius $t-1$ in the first $m$ coordinates.  The intersection recurrence is the same because the two centers agree in the added coordinate.  The Lloyd recurrence is \eqref{eq:S-lloyd-length}.
\end{proof}

Set
\begin{equation}
 x=\frac{\Vol_{t-1}^{(Q)}(m)}{\Vol_t^{(Q)}(m)},\quad
 y=\frac{c_{t-1}^{(Q)}(m,s)}{c_t^{(Q)}(m,s)},\quad
 z=\frac{\Lloyd_{t-1}^{(Q,m)}(s)}{\Lloyd_t^{(Q,m)}(s)}.
 \label{eq:S-xyz}
\end{equation}
For $1\le s\le2t$ the intersection $B_t(0)\cap B_t(z)$ is nonempty, so $c_t^{(Q)}(m,s)>0$ and $y$ is well defined; if $c_{t-1}^{(Q)}(m,s)=0$ then $y=0$.
Substituting \eqref{eq:S-V-length}--\eqref{eq:S-L-length} into $R$ gives the exact factorization
\begin{equation}
 \frac{R_{Q;m+1,t}(s)}{R_{Q;m,t}(s)}
 =\frac{(1+(Q-1)x)(1+(Q-1)y)}{(1+(Q-1)z)^2}.
 \label{eq:S-length-factor}
\end{equation}
Thus $R_{Q;m+1,t}(s)\le R_{Q;m,t}(s)$ follows from the ratio sandwich
\begin{equation}
 0\le y\le x\le z.
 \label{eq:S-sandwich}
\end{equation}

The shell estimate used below is elementary.  For
\begin{equation}
 w_j^{(Q)}(N)=(Q-1)^j\binom Nj,
\end{equation}
we have
\begin{equation}
 \frac{w_{\ell-1}^{(Q)}(N)}{w_\ell^{(Q)}(N)}
 =\frac{\ell}{(Q-1)(N-\ell+1)}.
 \label{eq:S-shell-ratio}
\end{equation}
Since this ratio is increasing in $\ell$, if
\begin{equation}
 \eta=\frac{j}{(Q-1)(N-j+1)}<1,
\end{equation}
then $w_{\ell-1}^{(Q)}(N)\le\eta w_{\ell}^{(Q)}(N)$ for $1\le\ell\le j$.  Summing the shifted inequalities gives the explicit domination
\begin{equation}
 \Vol_{j-1}^{(Q)}(N)=\sum_{\ell=0}^{j-1}w_{\ell}^{(Q)}(N)
 \le \eta\sum_{\ell=1}^{j}w_{\ell}^{(Q)}(N)
 \le \eta\Vol_j^{(Q)}(N),
\end{equation}
so
\begin{equation}
 \frac{\Vol_{j-1}^{(Q)}(N)}{\Vol_j^{(Q)}(N)}\le\eta.
 \label{eq:S-shell-tail}
\end{equation}

To prove $y\le x$, decompose $c_t(m,s)$ by the local type \eqref{eq:S-c-explicit}.  For fixed $(a,b,c)$ on the separated support, the larger of the two local distances is
\begin{equation}
 h=c+\max(a,b)=s-\min(a,b).
\end{equation}
The remaining $m-s$ coordinates contribute $\Vol_{t-h}^{(Q)}(m-s)$ with a nonnegative coefficient independent of $t$.  It is therefore enough to compare the ball ratios term by term.  Put $r=t-h$ and $N=m-s$.  For each $0\le p<r$,
\begin{equation}
 \frac{w_{r-p-1}^{(Q)}(N)}{w_{r-p}^{(Q)}(N)}
 \le
 \frac{w_{t-p-1}^{(Q)}(m)}{w_{t-p}^{(Q)}(m)}
 \label{eq:S-adjacent-dom}
\end{equation}
if and only if
\begin{equation}
 h(m-t+p+1)\ge (t-p)(s-h).
\end{equation}
Here $h\ge s-h$ because $h=s-\min(a,b)$, and $m\ge4t+1$ implies $m-t+p+1\ge t-p$.  Hence \eqref{eq:S-adjacent-dom} holds.  Multiplying the adjacent inequalities gives
\begin{equation}
 \frac{w_{r-k}^{(Q)}(N)}{w_r^{(Q)}(N)}
 \le
 \frac{w_{t-k}^{(Q)}(m)}{w_t^{(Q)}(m)},
 \qquad 1\le k\le r.
\end{equation}
Therefore
\begin{equation}
 A_N:=\frac{\Vol_{r-1}^{(Q)}(N)}{w_r^{(Q)}(N)}
 \le
 A_m:=\frac{\Vol_{t-1}^{(Q)}(m)}{w_t^{(Q)}(m)}.
\end{equation}
Since the map $A\mapsto A/(1+A)$ is increasing on $[0,\infty)$,
\begin{equation}
 \frac{\Vol_{r-1}^{(Q)}(N)}{\Vol_r^{(Q)}(N)}
 =\frac{A_N}{1+A_N}
 \le
 \frac{A_m}{1+A_m}
 =\frac{\Vol_{t-1}^{(Q)}(m)}{\Vol_t^{(Q)}(m)}.
\end{equation}
Terms with $r=0$ contribute zero to the numerator.  Summing the nonnegative local-type weights therefore yields
\begin{equation}
 \frac{c_{t-1}^{(Q)}(m,s)}{c_t^{(Q)}(m,s)}
 \le
 \frac{\Vol_{t-1}^{(Q)}(m)}{\Vol_t^{(Q)}(m)},
 \label{eq:S-y-le-x}
\end{equation}
so $y\le x$.

For the volume ratio $x$, the shell-tail estimate gives
\begin{equation}
 x\le \frac{t}{(Q-1)(m-t+1)}.
 \label{eq:S-x-upper}
\end{equation}
By the Lloyd shift identity,
\begin{equation}
 z=\frac{\Kraw_{t-1}^{(Q)}(s-1;m-1)}{\Kraw_t^{(Q)}(s-1;m-1)}.
 \label{eq:S-z-kraw}
\end{equation}
Let $N=m-1$.  The symmetric Jacobi matrix for monic $Q$-ary Krawtchouk polynomials has diagonal and off-diagonal entries
\begin{equation}
 b_i=\frac{(Q-1)N-(Q-2)i}{Q},
 \qquad
 a_i=\frac{\sqrt{(Q-1)(i+1)(N-i)}}{Q}.
 \label{eq:S-jacobi}
\end{equation}
The three-term recurrence for the orthonormal Krawtchouk system is represented by this real symmetric Jacobi matrix, with the spectral variable equal to the Hamming distance $x$.  Therefore the zeros of $\Kraw_t^{(Q)}(x;N)$ are the eigenvalues of its $t\times t$ leading truncation.  The elementary Weyl bound for the smallest eigenvalue, applied to the displayed diagonal and off-diagonal entries, gives
\begin{equation}
 \xi_1\ge
 \frac{(Q-1)N-(Q-2)(t-1)-2\sqrt{(Q-1)(t-1)(N-t+2)}}{Q}.
 \label{eq:S-zero-lower}
\end{equation}
For $N\ge4t$ and $Q\ge16$, the right hand side is $>2t-1$.  The displayed lower bound is increasing in $N$ on this range, since its derivative is $Q^{-1}((Q-1)-\sqrt{(Q-1)(t-1)/(N-t+2)})>0$.  It is therefore enough to check $N=4t$.  There the quantity $A=(Q-1)N-(Q-2)(t-1)-Q(2t-1)$ is positive, so the desired inequality may be squared.  After squaring, the difference between the two sides is
\begin{equation}
 (Q^2-16Q+16)t^2+4(Q-1)^2t+4(Q-1)(Q+1)>0.
 \label{eq:S-zero-square}
\end{equation}
Thus $0\le s-1\le2t-1$ lies to the left of the first zero.  The standard partial-fraction expansion for consecutive orthogonal polynomials, equivalently the spectral-measure representation of the Jacobi matrix, gives positive residues:
\begin{equation}
\frac{\Kraw_{t-1}^{(Q)}(x;N)}{\Kraw_t^{(Q)}(x;N)}=\sum_j\frac{\alpha_j}{\xi_j-x},\qquad \alpha_j>0.
\label{eq:S-partial-fraction}
\end{equation}
where the $\xi_j$ are the zeros of $\Kraw_t^{(Q)}(\cdot;N)$.  Hence, to the left of the first zero, the ratio is positive and increasing as $x$ increases toward the zero, since
\begin{equation}
 \frac{d}{dx}\sum_j\frac{\alpha_j}{\xi_j-x}
 =\sum_j\frac{\alpha_j}{(\xi_j-x)^2}>0.
\label{eq:S-partial-fraction-monotone}
\end{equation}
Using $\Kraw_j^{(Q)}(0;N)=(Q-1)^j\binom Nj$ gives
\begin{equation}
 z\ge \frac{\Kraw_{t-1}^{(Q)}(0;m-1)}{\Kraw_t^{(Q)}(0;m-1)}
 =\frac{t}{(Q-1)(m-t)}.
 \label{eq:S-z-lower}
\end{equation}
Combining \eqref{eq:S-x-upper} and \eqref{eq:S-z-lower} gives $x\le z$, hence the sandwich \eqref{eq:S-sandwich}.  The same first-zero bound also gives $\Lloyd_t^{(Q,m)}(s)>0$ throughout $1\le s\le2t$, since $\Kraw_t^{(Q)}(0;m-1)>0$ and no zero is crossed before $s-1$.  By \eqref{eq:S-length-factor},
\begin{equation}
 R_{Q;m+1,t}(s)\le R_{Q;m,t}(s)
 \qquad(Q\ge16,\ m\ge4t+1,\ 1\le s\le2t).
 \label{eq:S-length-monotone}
\end{equation}
Repeated application reduces all $n\ge4t+1$ to $n=4t+1$.
Therefore, for $Q\ge16$, it is enough to prove the raw Lloyd-square comparison
and Lloyd positivity at the critical length $n=4t+1$.  This is the input used in
Secs.~\ref{sec:Sjacobi}--\ref{sec:S3}.

\smsection{Two-center Jacobi comparison}{sec:Sjacobi}

The common Jacobi structure used later in the high-alphabet
critical comparison and in the qutrit long range is as follows.  The purpose of this section
is only to turn a two-center intersection ratio into the largest eigenvalue of
a nonnegative tridiagonal matrix; the two applications insert their own node and
edge weights below.  The setup is the two-ball intersection in the $Q$-ary
Hamming scheme.

Let the separated coordinate count be fixed.  In the two-ball intersection,
write the boundary layers of the two balls as a parity chain of node types
\(c\), with positive node weights \(D_c\), and odd imbalance edge types \(e\)
with positive weights \(B_e\).  The relevant shell increment is
\(I_s=C_s-C_{s+1}\).  In the applications below the quantities
\(D_c,B_e,\alpha_c,\beta_e,\gamma_e\) are defined explicitly from the
coordinate types of the two-center intersection; the present paragraph fixes
only the algebraic consequence of such a decomposition.  The node--edge
classification has the form
\begin{align}
 I_s&=\sum_{c}D_c,\label{eq:S-jacobi-template-I}\\
 C_s&=\sum_c\alpha_cD_c+\sum_e\beta_eB_e,\label{eq:S-jacobi-template-C}
\end{align}
with \(\alpha_c,\beta_e\ge0\).  When an edge \(e\) joins the neighboring nodes
\(e-1\) and \(e+1\), its weight satisfies
\begin{equation}
 \frac{B_e^2}{D_{e-1}D_{e+1}}=\gamma_e.
 \label{eq:S-jacobi-template-gamma}
\end{equation}
There may also be one one-sided edge at the left boundary of an odd chain.  If
that edge has weight \(B_0\), coefficient \(\beta_0\), and is attached to the
first node \(c_0\), its contribution is included as the diagonal update
\begin{equation}
 J_{c_0,c_0}\leftarrow J_{c_0,c_0}+\frac{\beta_0B_0}{D_{c_0}},
 \label{eq:S-jacobi-one-sided-update}
\end{equation}
since \((\beta_0B_0/D_{c_0})v_{c_0}^2=\beta_0B_0\).  With
\(v_c=\sqrt{D_c}\), define the remaining entries of the symmetric tridiagonal
matrix \(J\) by
\begin{equation}
 J_{c,c}=\alpha_c,
 \qquad
 J_{e-1,e+1}=J_{e+1,e-1}=\frac{1}{2}\beta_e\sqrt{\gamma_e}.
 \label{eq:S-jacobi-template-J}
\end{equation}
For an ordinary edge \(e\), the corresponding off-diagonal terms contribute
\begin{equation}
 2J_{e-1,e+1}v_{e-1}v_{e+1}
 =\beta_e\sqrt{\gamma_e D_{e-1}D_{e+1}}
 =\beta_eB_e.
 \label{eq:S-jacobi-edge-recovery}
\end{equation}
Together with \eqref{eq:S-jacobi-one-sided-update}, this gives
\begin{equation}
 C_s=v^{\mathsf T}Jv,
 \qquad
 I_s=v^{\mathsf T}v,
 \qquad
 \frac{C_s}{I_s}\le\lambda_{\max}(J).
 \label{eq:S-jacobi-template-Rayleigh}
\end{equation}
Thus a two-center ratio comparison is reduced to a spectral bound for a
nonnegative tridiagonal matrix.

The spectral majorants used below are two universal parity Jacobi models.  Let
\(\mathsf K_0\) and \(\mathsf K_1\) be the half-line Jacobi matrices with zero
diagonal and off-diagonal entries
\begin{equation}
 b_j^{(0)}=\sqrt\frac{2j+2}{2j+1},
 \qquad
 b_j^{(1)}=\sqrt\frac{2j+3}{2j+2}.
 \label{eq:S-jacobi-model-b}
\end{equation}
For the even model put
\begin{equation}
 \phi_j=(2j+1)\sqrt{\binom{2j}{j}}\,2^{-3j/2}.
 \label{eq:S-jacobi-even-ground}
\end{equation}
Then
\begin{equation}
 b_{j-1}^{(0)}\phi_{j-1}+b_j^{(0)}\phi_{j+1}
 =\frac{3}{\sqrt2}\phi_j,
 \label{eq:S-jacobi-ground-eigen}
\end{equation}
with the first term omitted at \(j=0\).  Hence, for every finitely supported
sequence \(x_j=\phi_jy_j\),
\begin{equation}
 \frac{3}{\sqrt2}\sum_jx_j^2
 -2\sum_jb_j^{(0)}x_jx_{j+1}
 =\sum_jb_j^{(0)}\phi_j\phi_{j+1}(y_j-y_{j+1})^2\ge0.
 \label{eq:S-jacobi-ground-state}
\end{equation}
Every finite truncation of \(\mathsf K_0\) therefore has norm at most
\(3/\sqrt2\).

The shifted odd chain has the same bound with an explicit boundary reserve.  Put
\begin{equation}
 \psi_j=(j+1)\sqrt{\frac{2^j}{(2j+1)\binom{2j}{j}}},
 \qquad j\ge0.
 \label{eq:S-jacobi-odd-ground}
\end{equation}
Equivalently,
\begin{equation}
 \frac{\psi_{j+1}}{\psi_j}
 =\frac{j+2}{\sqrt{(j+1)(2j+3)}}.
 \label{eq:S-jacobi-odd-ratio}
\end{equation}
Using \eqref{eq:S-jacobi-model-b}, this ratio gives the boundary identity
\begin{equation}
 b_0^{(1)}\psi_1+\frac{1}{\sqrt2}\psi_0=\frac{3}{\sqrt2}\psi_0
 \label{eq:S-jacobi-odd-boundary-eigen}
\end{equation}
and, for every \(j\ge1\),
\begin{equation}
 b_{j-1}^{(1)}\psi_{j-1}+b_j^{(1)}\psi_{j+1}
 =\frac{3}{\sqrt2}\psi_j.
 \label{eq:S-jacobi-odd-eigen}
\end{equation}
Indeed, \eqref{eq:S-jacobi-odd-ratio} gives
\begin{equation}
 \frac{b_j^{(1)}\psi_{j+1}}{\psi_j}=\frac{j+2}{\sqrt2(j+1)},
 \qquad
 \frac{b_{j-1}^{(1)}\psi_{j-1}}{\psi_j}=\frac{2j+1}{\sqrt2(j+1)},
 \label{eq:S-jacobi-odd-eigen-check}
\end{equation}
and the two displayed fractions add to \(3/\sqrt2\).  Hence, for every
finitely supported sequence \(x_j=\psi_jy_j\),
\begin{equation}
 \frac{3}{\sqrt2}\sum_jx_j^2
 -2\sum_jb_j^{(1)}x_jx_{j+1}
 -\frac{1}{\sqrt2}x_0^2
 =\sum_jb_j^{(1)}\psi_j\psi_{j+1}(y_j-y_{j+1})^2\ge0.
 \label{eq:S-jacobi-odd-ground-state}
\end{equation}
This is the boundary-improved form
\begin{equation}
 \mathsf K_1+\frac{1}{\sqrt2}P_0\preceq \frac{3}{\sqrt2}I,
 \label{eq:S-jacobi-odd-boundary}
\end{equation}
where \(P_0\) is the rank-one projection onto the first node.  In particular,
the ordinary odd truncations also have norm at most \(3/\sqrt2\), and any
additional left boundary load bounded by \(c/\sqrt2\) can be absorbed into an
off-diagonal model coefficient \(c\).

The way this template is used is as follows.  If the concrete two-center
coefficients satisfy
\begin{equation}
 \alpha_c\le A,
 \qquad
 \beta_e\sqrt{\gamma_e}\le B\sqrt{q}\,b_j^{(\epsilon)},
 \label{eq:S-jacobi-template-domination}
\end{equation}
for the appropriate parity model, and the possible one-sided boundary load is
absorbed by \eqref{eq:S-jacobi-odd-boundary}, then the concrete finite matrix is
entrywise dominated by the corresponding finite model.  Since both matrices are
symmetric with nonnegative entries, Perron--Frobenius monotonicity gives the
same ordering of largest eigenvalues; combining this with
\eqref{eq:S-jacobi-ground-state} and \eqref{eq:S-jacobi-odd-ground-state} gives
\begin{equation}
 \lambda_{\max}(J)\le A+\frac{3}{2\sqrt2}B\sqrt q,
 \label{eq:S-jacobi-template-bound}
\end{equation}
with the extra boundary term included as stated in the concrete
qutrit estimate.  The remaining work in Secs.~\ref{sec:S3} and~\ref{sec:S4}
is therefore to compute \(D,B,\alpha,\beta,\gamma\), establish the entrywise
majorants, and compare the resulting scalar bound with the required target.

\smsection{High-alphabet half-gap at critical length}{sec:S3}

After Sec.~\ref{sec:S2}, all high-alphabet cases have been reduced to
\(n=4t+1\).  We now instantiate the common two-center Jacobi template of
Sec.~\ref{sec:Sjacobi}.  The proof makes the node weights, edge weights,
entrywise parity-model domination, and final scalar gap explicit, so the
critical comparison is an explicit Jacobi estimate followed by a
one-variable rational inequality.  Put
\begin{equation}
 C_s=c_t^{(Q)}(4t+1,s),\qquad I_s=C_s-C_{s+1}.
 \label{eq:S-CsIs-critical}
\end{equation}
For \(2\le s\le 2t-1\), set
\begin{equation}
 x=s-1,\qquad
 L_s=\Kraw_t^{(Q)}(x;4t),\qquad
 M_s=\Kraw_{t-1}^{(Q)}(x;4t-1).
 \label{eq:S-LsMs-critical}
\end{equation}
The first-difference identity
\begin{equation}
 \Kraw_t^{(Q)}(x+1;N)-\Kraw_t^{(Q)}(x;N)
 =-Q\Kraw_{t-1}^{(Q)}(x;N-1)
 \label{eq:S-kraw-first-diff-critical}
\end{equation}
comes directly from the generating function by replacing one factor
\((1+(Q-1)u)\) with \((1-u)\).  With \(N=4t\) and \(x=s-1\), this gives
\begin{equation}
 L_{s+1}=L_s-QM_s.
 \label{eq:S-L-difference-critical}
\end{equation}
We shall use the following contiguous ratio bound for this same positive
branch:
\begin{equation}
 0<\frac{M_s}{L_s}\le \frac{t}{D_Q(t,s)},
 \qquad
 D_Q(t,s)=4(Q-1)t-\frac{9Q}{8}(s-1).
 \label{eq:S-L-ratio-critical}
\end{equation}
Equivalently, with \(x=s-1\), this is the cleared inequality
\begin{equation}
 t\Kraw_t^{(Q)}(x;4t)-D_Q(t,x+1)\Kraw_{t-1}^{(Q)}(x;4t-1)\ge0,
 \qquad 1\le x\le2t-2.
 \label{eq:S-contiguous-ratio-cleared}
\end{equation}
The small cases \(t=1,2\) are checked directly in the small-\(t\)
boundary table below; the propagation proof below is used only for \(t\ge3\).
For \(t\ge3\), the first-zero bound for \(\Kraw_t^{(Q)}(\cdot;4t)\),
obtained from the same degree Jacobi matrix, places the first zero to the right
of \(2t-1\).  Hence
\(L_s=\Kraw_t^{(Q)}(x;4t)>0\) throughout \(1\le x\le2t-2\), and the ratio
\(M_s/L_s\) has a fixed sign.  The remaining comparison is made before any
sign-sensitive division: \eqref{eq:S-L-ratio-critical} is exactly the cleared
inequality \eqref{eq:S-contiguous-ratio-cleared}, together with \(L_s>0\) and
\(D_Q(t,s)>0\).

We now prove \eqref{eq:S-contiguous-ratio-cleared} by writing out the
continued-fraction comparison.  Put
\begin{equation}
 P_j=\Kraw_j^{(Q)}(x;4t-1),\qquad r_j=\frac{P_{j-1}}{P_j}\quad (1\le j\le t).
 \label{eq:S-critical-Pj-rj}
\end{equation}
The length recursion gives
\begin{equation}
 L_s=P_t+(Q-1)P_{t-1},\qquad M_s=P_{t-1},
 \qquad
 \frac{M_s}{L_s}=\frac{r_t}{1+(Q-1)r_t}.
 \label{eq:S-critical-M-over-L-r}
\end{equation}
The fixed-length degree recurrence for the \(Q\)-ary Krawtchouk polynomials is
\begin{equation}
 jP_j=A_jP_{j-1}-B_jP_{j-2},
 \quad
 A_j=(Q-1)(4t-j)+j-1-Qx,
 \quad
 B_j=(Q-1)(4t-j+1).
 \label{eq:S-critical-degree-recurrence}
\end{equation}
Thus, whenever the previous ratios are positive,
\begin{equation}
 r_j=\frac{j}{A_j-B_jr_{j-1}}.
 \label{eq:S-critical-rj-recurrence}
\end{equation}
Set
\begin{equation}
 E_j=(Q-1)(4t-j)-Qx\left(1+\frac{j}{8t}\right),
 \qquad 1\le j\le t.
 \label{eq:S-critical-Ej}
\end{equation}
For \(Q\ge16\), \(t\ge3\), and \(1\le x\le2t-2\), these denominators are
positive, since \(E_j\) is minimized at \(j=t\), \(x=2t-2\), where
\begin{equation}
 E_t\ge \left(\frac{3Q}{4}-3\right)t+\frac{9Q}{4}>0.
 \label{eq:S-critical-Ej-positive}
\end{equation}
We claim that
\begin{equation}
 0<r_j\le\frac{j}{E_j}
 \qquad (1\le j\le t).
 \label{eq:S-critical-rj-barrier}
\end{equation}
For \(j=1\), this follows from \(r_1=1/A_1\) and \(A_1>E_1>0\).  Suppose it
has been proved up to \(j-1\).  Then the denominator in
\eqref{eq:S-critical-rj-recurrence} is at least
\(A_j-B_j(j-1)/E_{j-1}\).  Hence it is enough to check
\begin{equation}
 A_j-\frac{B_j(j-1)}{E_{j-1}}\ge E_j.
 \label{eq:S-critical-barrier-step}
\end{equation}
After multiplying by the positive number \(E_{j-1}\), the left side minus the
right side equals
\begin{equation}
 \frac{Qx}{64t^2}\,H_j(x),
 \label{eq:S-critical-barrier-residual}
\end{equation}
where
\begin{align}
 H_j(x)=&-8Qj^2t-Qj^2x+32Qjt^2-8Qjtx+8Qjt+Qjx
        \notag\\
       &{}-96jt^2+8jt+64t^2-8t.
 \label{eq:S-critical-Hj}
\end{align}
This polynomial is decreasing in \(x\).  At \(x=2t-2\), the quantity
\(H_j(2t-2)/2\), as a polynomial in \(j\), is concave on \([2,t]\).  Therefore
its minimum on the integer interval \(2\le j\le t\) occurs at an endpoint, and
those endpoint values are
\begin{align}
 \frac{H_2(2t-2)}{2}
   &=2\{8Qt^2+3Qt+Q-32t^2+2t\}>0,\notag\\
 \frac{H_t(2t-2)}{2}
   &=t\{(3Q-48)t^2+(14Q+36)t-(Q+4)\}>0.
 \label{eq:S-critical-H-endpoints}
\end{align}
Here the inequalities use \(Q\ge16\) and \(t\ge3\).  Thus
\eqref{eq:S-critical-barrier-step} holds, so the induction proves
\eqref{eq:S-critical-rj-barrier}.  Taking \(j=t\) gives
\begin{equation}
 r_t\le \frac{t}{3(Q-1)t-\frac{9Q}{8}x}.
 \label{eq:S-critical-rt-bound}
\end{equation}
Since \(r\mapsto r/(1+(Q-1)r)\) is increasing for \(r\ge0\),
\eqref{eq:S-critical-M-over-L-r} and \eqref{eq:S-critical-rt-bound} give
\begin{equation}
 \frac{M_s}{L_s}
 \le
 \frac{t}{3(Q-1)t-\frac{9Q}{8}x+(Q-1)t}
 =\frac{t}{D_Q(t,x+1)}.
 \label{eq:S-critical-ratio-from-barrier}
\end{equation}
Together with positivity, this proves \eqref{eq:S-L-ratio-critical}.  Moreover
\begin{equation}
 \frac{D_Q(t,s)}{t}
 \ge 4(Q-1)-\frac{9Q}{8}\frac{2t-2}{t}
 >Q,
 \label{eq:S-DQ-positive-critical}
\end{equation}
so \(0<Qt/D_Q(t,s)<1\).
Therefore, writing \(u_s=M_s/L_s\),
\begin{equation}
 \frac{R_{Q;4t+1,t}(s+1)}{R_{Q;4t+1,t}(s)}
 =\frac{1-I_s/C_s}{(1-Qu_s)^2}.
 \label{eq:S-R-step-factor-critical}
\end{equation}
Since \(0<Qu_s<1\), it is enough to prove
\begin{equation}
 \frac{C_s}{I_s}\le T_Q(t,s),
 \qquad
 T_Q(t,s)=\frac{D_Q(t,s)^2}{Qt\{2D_Q(t,s)-Qt\}}.
 \label{eq:S-target-critical}
\end{equation}
Indeed \eqref{eq:S-target-critical} is equivalent to
\begin{equation}
 \frac{I_s}{C_s}\ge \frac{Qt}{D_Q(t,s)}
 \left(2-\frac{Qt}{D_Q(t,s)}\right).
 \label{eq:S-target-IoverC-critical}
\end{equation}
The right hand side is positive by \eqref{eq:S-DQ-positive-critical}; since
\(u_s\le t/D_Q(t,s)\) and the function \(v\mapsto Qv(2-Qv)\) is increasing on
\(0\le v\le t/D_Q(t,s)<1/Q\), \eqref{eq:S-target-IoverC-critical} implies
\(I_s/C_s\ge Qu_s(2-Qu_s)\), which is exactly
\eqref{eq:S-R-step-factor-critical}\(\le1\).
For \(Q=16\), with \(r=2t-s\),
\begin{equation}
 T_{16}(t,s)=\frac{9(4t+3r+3)^2}{16t(8t+9r+9)}.
 \label{eq:S-T16-critical}
\end{equation}

We now give the exact two-center Jacobi decomposition.  Put
\begin{equation}
 r=2t-s,
 \qquad
 N=4t-s.
 \label{eq:S-rN-critical}
\end{equation}
The node and ordinary-edge sets are
\begin{align}
 \mathcal C_s&=\{c:0\le c\le\min(s,r),\ c\equiv s\pmod2\},
 \label{eq:S-Cset-critical}\\
 \mathcal E_s&=\{e:1\le e\le\min(s,r-1),\ e\not\equiv s\pmod2\}.
 \label{eq:S-Eset-critical}
\end{align}
For \(c\in\mathcal C_s\), let \(m_c=s-c\) and
\(\ell_c=(r-c)/2\), and define
\begin{equation}
 D_c^{(Q)}=
 \binom{s}{c}(Q-2)^c
 \binom{s-c}{(s-c)/2}
 w_{\ell_c}^{(Q)}(N).
 \label{eq:S-Dc-critical}
\end{equation}
For \(e\in\mathcal E_s\), put \(\rho_e=(r-e-1)/2\) and
\begin{equation}
 B_e^{(Q)}=
 \binom{s}{e}(Q-2)^e
 \binom{s-e}{(s-e-1)/2}
 w_{\rho_e}^{(Q)}(N).
 \label{eq:S-Be-critical}
\end{equation}
The imbalance sums are
\begin{align}
 \alpha_c^{(Q)}={}&
 \sum_{j=0}^{\min(m_c/2,\ell_c)}
 (2-\delta_{j0})
 \frac{\binom{m_c}{m_c/2-j}}
      {\binom{m_c}{m_c/2}}
 \frac{\Vol_{\ell_c-j}^{(Q)}(N+1)}
      {w_{\ell_c}^{(Q)}(N)},
 \label{eq:S-alpha-critical}\\
 \beta_e^{(Q)}={}&
 2\sum_{j=0}^{\min((s-e-1)/2,\rho_e)}
 \frac{\binom{s-e}{(s-e-1)/2-j}}
      {\binom{s-e}{(s-e-1)/2}}
 \frac{\Vol_{\rho_e-j}^{(Q)}(N+1)}
      {w_{\rho_e}^{(Q)}(N)}.
 \label{eq:S-beta-critical}
\end{align}
When \(s\) is odd, the one-sided edge uses the same formula with
\(e=0\), namely \(\rho_0=(r-1)/2\); we denote the resulting coefficient by
\(\beta_0^{(Q)}\), and set
\begin{equation}
 B_0^{(Q)}=\frac{2D_1^{(Q)}}{(Q-2)(s+1)}.
 \label{eq:S-B0-critical}
\end{equation}
The local-type derivation is as follows.  On the \(s\) separated coordinates,
a point in \(B_t(0)\cap B_t(z)\) may use equal nonzero symbols at some of the
separated positions, and the remaining separated positions are split between
the two centers.  The parity of the unmatched separated positions determines
whether the two residual radii are equal or differ by one.  In the difference
\(I_s=C_s-C_{s+1}\), the only surviving boundary terms are the equal-residual
classes; choosing \(c\) equal nonzero separated positions gives the
multinomial and central-binomial factors in \eqref{eq:S-Dc-critical}, and the
outside coordinates must lie on the top shell \(\ell_c\), giving
\(D_c^{(Q)}\).  The full intersection \(C_s\) also contains the two
neighbouring imbalance classes.  These sit between the adjacent equal-residual
nodes \(e-1\) and \(e+1\); summing the lower outside shells produces the
coefficients \(\beta_e^{(Q)}\), while the top-shell geometric mean is
\(B_e^{(Q)}\).  If \(s\) is odd, the leftmost imbalance has no node on one
side of the chain; its contribution is therefore the one-sided edge
\(B_0^{(Q)}\) attached to the first node \(c=1\), not an omitted ordinary
edge.  This gives the exact identities
\begin{align}
 I_s&=\sum_{c\in\mathcal C_s}D_c^{(Q)},
 \label{eq:S-Is-node-critical}\\
 C_s&=\sum_{c\in\mathcal C_s}\alpha_c^{(Q)}D_c^{(Q)}
 +\sum_{e\in\mathcal E_s}\beta_e^{(Q)}B_e^{(Q)}
 +\mathbf 1_{\{s\ {\rm odd}\}}\beta_0^{(Q)}B_0^{(Q)}.
 \label{eq:S-Cs-edge-critical}
\end{align}
Here \(D_c^{(Q)}\) is the double-boundary contribution with equal
remaining radius at the two centers, while \(B_e^{(Q)}\) is the odd
imbalance contribution sitting between the neighbouring nodes \(e-1\)
and \(e+1\).  The cancellation in the geometric mean is completely local:
with \(\rho_e=(r-e-1)/2\),
\begin{align}
 \frac{\binom{s}{e}^2}{\binom{s}{e-1}\binom{s}{e+1}}
 &=\frac{(e+1)(s-e+1)}{e(s-e)},\nonumber\\
 \frac{\binom{s-e}{(s-e-1)/2}^2}
 {\binom{s-e+1}{(s-e+1)/2}\binom{s-e-1}{(s-e-1)/2}}
 &=\frac{s-e}{s-e+1},\nonumber\\
 \frac{w_{\rho_e}^{(Q)}(N)^2}{w_{\rho_e}^{(Q)}(N)w_{\rho_e+1}^{(Q)}(N)}
 &=\frac{\rho_e+1}{(Q-1)(N-\rho_e)}.
 \label{eq:S-gamma-cancel-factors}
\end{align}
Multiplying these three displayed factors gives
\begin{equation}
 \frac{(B_e^{(Q)})^2}{D_{e-1}^{(Q)}D_{e+1}^{(Q)}}
 =\frac{(e+1)(\rho_e+1)}{(Q-1)e(N-\rho_e)}
 =:\gamma_e^{(Q)}.
 \label{eq:S-gamma-critical}
\end{equation}
Let \(v_c=\sqrt{D_c^{(Q)}}\).  Define the symmetric tridiagonal matrix
\(J_{Q;t,s}\) on \(\mathcal C_s\) by
\begin{align}
 (J_{Q;t,s})_{c,c}&=\alpha_c^{(Q)},
 \label{eq:S-J-diag-critical}\\
 (J_{Q;t,s})_{e-1,e+1}&=(J_{Q;t,s})_{e+1,e-1}
 =\frac12\beta_e^{(Q)}\sqrt{\gamma_e^{(Q)}}
 \qquad(e\in\mathcal E_s),
 \label{eq:S-J-edge-critical}
\end{align}
and, when \(s\) is odd, add
\begin{equation}
 \frac{2\beta_0^{(Q)}}{(Q-2)(s+1)}
 \label{eq:S-J-special-critical}
\end{equation}
to the diagonal entry indexed by \(c=1\).  Then
\begin{equation}
 C_s=v^{\mathsf T}J_{Q;t,s}v,
 \qquad
 I_s=v^{\mathsf T}v.
 \label{eq:S-Rayleigh-critical}
\end{equation}
Thus \eqref{eq:S-target-critical} follows once
\begin{equation}
 \lambda_{\max}(J_{Q;t,s})\le T_Q(t,s).
 \label{eq:S-J-target-critical}
\end{equation}

The alphabet reduction follows term by term from the displayed formulae.  Every term in
\eqref{eq:S-alpha-critical} and \eqref{eq:S-beta-critical} is a positive
linear combination of powers \((Q-1)^{p-\ell}\) with \(p\le\ell\).  Indeed,
each quotient \(\Vol_a^{(Q)}(N+1)/w_b^{(Q)}(N)\) expands as a finite sum
of binomial factors times \((Q-1)^{j-b}\), with \(j\le a\le b\).  Hence
these diagonal and edge coefficients are nonincreasing in \(Q\).  The
factor \(\gamma_e^{(Q)}\) and the exceptional factor \((Q-2)^{-1}\) are
also decreasing.  Therefore
\begin{equation}
 J_{Q;t,s}\le J_{16;t,s}\quad\hbox{entrywise for }Q\ge16.
 \label{eq:S-J-monotone-critical}
\end{equation}
Since the matrices are nonnegative and symmetric, Perron--Frobenius gives
\(\lambda_{\max}(J_{Q;t,s})\le\lambda_{\max}(J_{16;t,s})\).
On the target side, write
\begin{equation}
 z_Q=\frac{D_Q(t,s)}{Qt}=4-\frac4Q-\frac98\frac{s-1}{t}.
 \label{eq:S-zQ-critical}
\end{equation}
Then \(z_Q\) is increasing in \(Q\), and \(z_{16}>1\) for
\(2\le s\le2t-1\).  Since \(g(z)=z^2/(2z-1)\) is increasing for
\(z>1\),
\begin{equation}
 T_Q(t,s)=g(z_Q)\ge g(z_{16})=T_{16}(t,s).
 \label{eq:S-target-monotone-critical}
\end{equation}
Consequently the whole high-alphabet critical comparison reduces first to the
smallest high alphabet.  We now close that comparison by an explicit spectral
comparison.
Set
\begin{equation}
 \zeta_*=\frac{r}{15(4t+r+2)},
 \qquad
 A(\zeta)=\frac{(1+15\zeta)(1+\zeta)}{(1-\zeta)^2},
 \qquad
 B(\zeta)=\frac{2(1+15\zeta)}{(1-\zeta)^2}.
 \label{eq:S-AB-zeta-critical}
\end{equation}
The shell-tail estimate \eqref{eq:S-shell-tail}, applied inside the node
and edge sums \eqref{eq:S-alpha-critical}--\eqref{eq:S-beta-critical}, bounds each lower ball by a geometric tail over the top shell.  Summing the resulting central-binomial weights gives the elementary majorants \(A\) and \(B\); explicitly, for every node and ordinary edge
\begin{equation}
 \alpha_c^{(16)}\le A(\zeta_*),
 \qquad
 \beta_e^{(16)}\le B(\zeta_*).
 \label{eq:S-alpha-beta-AB-critical}
\end{equation}
Indeed, for a node put
\begin{equation}
 \zeta_c=\frac{\ell_c}{15(N-\ell_c+1)}.
 \label{eq:S-zeta-c-critical}
\end{equation}
The shell-tail estimate gives, for every \(j\ge0\),
\begin{equation}
 \frac{\Vol_{\ell_c-j}^{(16)}(N+1)}{w_{\ell_c}^{(16)}(N)}
 \le (1+15\zeta_c)\frac{\zeta_c^j}{1-\zeta_c}.
 \label{eq:S-node-tail-to-zeta}
\end{equation}
The central-binomial ratios in \eqref{eq:S-alpha-critical} have total
geometric envelope \(\sum_{j\ge0}(j+1)\zeta_c^j=(1-\zeta_c)^{-2}\);
the factor \(2-\delta_{j0}\) is absorbed by the harmless multiplier
\(1+\zeta_c\).  Therefore
\begin{equation}
 \alpha_c^{(16)}
 \le (1+15\zeta_c)(1+\zeta_c)\sum_{j\ge0}(j+1)\zeta_c^j
 =A(\zeta_c).
 \label{eq:S-alpha-sum-to-A}
\end{equation}
Since \(\zeta_c\le\zeta_*\), and \(A\) is increasing on
\(0\le\zeta\le1/45\), this gives the first bound.  For an ordinary edge,
with \(\zeta_e=(\rho_e+1)/(15(N-\rho_e))\le\zeta_*\), the same
shell-tail bound and the central-binomial envelope give
\begin{equation}
 \beta_e^{(16)}
 \le 2(1+15\zeta_e)\sum_{j\ge0}(j+1)\zeta_e^j
 =B(\zeta_e)\le B(\zeta_*).
 \label{eq:S-beta-sum-to-B}
\end{equation}
For the ordinary edge between the neighbouring nodes \(c\) and \(c+2\),
that is \(e=c+1\), \eqref{eq:S-gamma-critical} becomes
\begin{equation}
 \gamma_{c+1}^{(16)}
 =\frac{c+2}{c+1}\,
 \frac{\ell_c}{15(N-\ell_c+1)}
 =\frac{c+2}{c+1}\zeta_c
 \le \frac{c+2}{c+1}\zeta_*.
 \label{eq:S-gamma-model-critical}
\end{equation}
After ordering the nodes by parity, the ordinary part of
\(J_{16;t,s}\) is therefore entrywise dominated by the finite truncation of
one of the two universal parity models:
\begin{equation}
 J_{16;t,s}^{\rm ord}
 \le_{\rm ent}
 A(\zeta_*)I+\frac{1}{2}B(\zeta_*)\sqrt{\zeta_*}\,
 \mathsf K_{\epsilon(s)}.
 \label{eq:S-entrywise-model-critical}
\end{equation}
Here \(\epsilon(s)=0\) or \(1\) according to the parity of the node chain,
and \(\mathsf K_0,\mathsf K_1\) have off-diagonal entries
\begin{equation}
 b_j^{(0)}=\sqrt\frac{2j+2}{2j+1},
 \qquad
 b_j^{(1)}=\sqrt\frac{2j+3}{2j+2}.
 \label{eq:S-model-b-critical}
\end{equation}
Both sides of \eqref{eq:S-entrywise-model-critical} are symmetric and
entrywise nonnegative, hence Perron--Frobenius monotonicity gives the same
inequality for their spectral radii.

The spectral estimates for the two universal parity models were proved in
Sec.~\ref{sec:Sjacobi}.  In particular, every finite truncation of the even
model \(\mathsf K_0\) has norm at most \(3/\sqrt2\), and the odd model has the
boundary reserve
\begin{equation}
 \mathsf K_1+\frac{1}{\sqrt2}P_0\preceq \frac{3}{\sqrt2}I.
 \label{eq:S-critical-odd-reserve-ref}
\end{equation}
These are the ground-state square identities
\eqref{eq:S-jacobi-ground-state} and
\eqref{eq:S-jacobi-odd-ground-state}, applied to the finite truncations
appearing here.

For even \(s\), \eqref{eq:S-entrywise-model-critical} and
\eqref{eq:S-jacobi-ground-state} give immediately
\begin{equation}
 \lambda_{\max}(J_{16;t,s})
 \le A(\zeta_*)+\frac{3}{2\sqrt2}B(\zeta_*)\sqrt{\zeta_*}.
 \label{eq:S-perron-even-critical}
\end{equation}
For odd \(s\) and \(r\ge3\), the special edge contributes at most
\begin{equation}
 d_*=\frac{B(\zeta_*)}{7(s+1)}
 \label{eq:S-special-d-critical}
\end{equation}
to the first diagonal entry, while the coefficient multiplying
\(\mathsf K_1\) is
\begin{equation}
 c_*=\frac{1}{2}B(\zeta_*)\sqrt{\zeta_*}.
 \label{eq:S-special-c-critical}
\end{equation}
Since \(t=(r+s)/2\),
\begin{equation}
 \zeta_*=\frac{r}{15(3r+2s+2)}.
 \label{eq:S-zeta-rs-critical}
\end{equation}
For odd \(r,s\ge3\),
\begin{equation}
 49r(s+1)^2-120(3r+2s+2)
 \ge147(s+1)^2-240(s+1)-1080>0,
 \label{eq:S-special-absorb-poly}
\end{equation}
and hence
\begin{equation}
 \frac{d_*}{c_*}
 =\frac{2}{7(s+1)\sqrt{\zeta_*}}
 \le \frac{1}{\sqrt2}.
 \label{eq:S-special-absorb-critical}
\end{equation}
The rank-one boundary term is therefore absorbed by
\eqref{eq:S-critical-odd-reserve-ref}, and the same bound
\eqref{eq:S-perron-even-critical} holds for every nonterminal odd chain.
The terminal odd case \(r=1\) is one-dimensional; since then \(s=2t-1\),
\begin{equation}
 \frac{C_s}{I_s}=1+\frac{1}{7t},
 \qquad
 T_{16}(t,2t-1)-\left(1+\frac{1}{7t}\right)
 =\frac{28t^2+220t+495}{56t(4t+9)}>0.
 \label{eq:S-terminal-r1-critical}
\end{equation}

It remains only to compare the scalar upper bound in
\eqref{eq:S-perron-even-critical} with the target.  Put
\begin{equation}
 u=\frac{r}{t},
 \qquad
 \bar\zeta=\frac{u}{15(4+u)}.
 \label{eq:S-zeta-bar-critical}
\end{equation}
Then \(0\le\zeta_*\le\bar\zeta\le1/45\), and the functions
\(A,B\) are increasing on this interval.  Moreover, at fixed \(u\),
\begin{equation}
 T_{16}(t,s)
 \ge \Theta(\bar\zeta),
 \qquad
 \Theta(\zeta)=
 \frac{9(1+30\zeta)^2}{(1-15\zeta)(8+420\zeta)}.
 \label{eq:S-Theta-critical}
\end{equation}
For \(0\le\zeta\le1/45\),
\begin{equation}
 \Theta(\zeta)
 \ge A(\zeta)+\frac{3}{2\sqrt2}B(\zeta)\sqrt\zeta.
 \label{eq:S-scalar-critical}
\end{equation}
Indeed,
\begin{equation}
 \frac{3}{2\sqrt2}\sqrt\zeta
 \le \frac{15}{2}\zeta+\frac{3}{80},
 \qquad
 \frac{15}{2}\zeta+\frac{3}{80}-\frac{3}{2\sqrt2}\sqrt\zeta
 =\frac{3}{80}(10\sqrt{2\zeta}-1)^2,
 \label{eq:S-root-linear-critical}
\end{equation}
and direct reduction gives
\begin{align}
&\Theta(\zeta)-A(\zeta)
 -B(\zeta)\left(\frac{15}{2}\zeta+\frac{3}{80}\right)\notag\\
&\qquad=
 \frac{15201000\zeta^4+1147275\zeta^3+22440\zeta^2-575\zeta+4}{40(1-\zeta)^2(1-15\zeta)(105\zeta+2)}.
 \label{eq:S-scalar-rational-critical}
\end{align}
The denominator is positive on \([0,1/45]\).  The numerator equals
\begin{equation}
 \zeta^3(15201000\zeta+1147275)+(22440\zeta^2-575\zeta+4),
 \label{eq:S-scalar-numerator-critical}
\end{equation}
and the final quadratic has discriminant
\begin{equation}
 575^2-4\cdot22440\cdot4=-28415<0.
 \label{eq:S-scalar-discriminant-critical}
\end{equation}
Equations \eqref{eq:S-perron-even-critical}--\eqref{eq:S-scalar-discriminant-critical}
prove
\begin{equation}
 \lambda_{\max}(J_{16;t,s})\le T_{16}(t,s),
 \qquad 2\le s\le2t-1.
 \label{eq:S-Q16-certificate-closed}
\end{equation}
Combining this with \eqref{eq:S-J-target-critical} closes the critical
separation propagation at \(Q=16\), and the monotonicity
\eqref{eq:S-J-monotone-critical}--\eqref{eq:S-target-monotone-critical}
lifts it to all \(Q\ge16\).

The initial separations are independent of the interior Jacobi comparison.  By
the Lloyd shift identity, at \(n=4t+1\),
\begin{equation}
 \Lloyd_t^{(Q,4t+1)}(s)=\Kraw_t^{(Q)}(s-1;4t).
 \label{eq:S-critical-L-shift}
\end{equation}
Hence
\begin{equation}
 \Lloyd_t^{(Q,4t+1)}(1)=(Q-1)^t\binom{4t}{t},
 \label{eq:S-L-s1}
\end{equation}
and
\begin{align}
 \Lloyd_t^{(Q,4t+1)}(2)
 &=(Q-1)^t\binom{4t-1}{t}-(Q-1)^{t-1}\binom{4t-1}{t-1}\nonumber\\
 &=(Q-1)^{t-1}\binom{4t-1}{t}\frac{3Q-4}{4}.
 \label{eq:S-L-s2}
\end{align}
The corresponding two-center intersections are
\begin{align}
 c_t^{(Q)}(4t+1,1)&=Q\Vol_{t-1}^{(Q)}(4t),
 \label{eq:S-c-s1}\\
 c_t^{(Q)}(4t+1,2)&=2\Vol_{t-1}^{(Q)}(4t-1)
 +(Q^2-2)\Vol_{t-2}^{(Q)}(4t-1).
 \label{eq:S-c-s2}
\end{align}
Using the shell-tail estimate \eqref{eq:S-shell-tail} to compare the
balls to the top shell of \(\Vol_t^{(Q)}(4t+1)\), one obtains
\begin{align}
 R_{Q;4t+1,t}(1)&\le \frac{4Q(Q-1)}{(3Q-4)^2},
 \label{eq:S-end1}\\
 R_{Q;4t+1,t}(2)&\le
 \frac{16(Q-1)^2(Q^2+6Q-8)}{(3Q-4)^4}.
 \label{eq:S-end2}
\end{align}
The endpoint estimates reduce to the following exact algebraic checks:
\begin{equation}
 \frac12-\frac{4Q(Q-1)}{(3Q-4)^2}
 =\frac{Q^2-16Q+16}{2(3Q-4)^2}\ge0,
 \label{eq:S-end1-check}
\end{equation}
and
\begin{equation}
 \frac12-
 \frac{16(Q-1)^2(Q^2+6Q-8)}{(3Q-4)^4}
 =\frac{(7Q-8)(7Q^3-72Q^2+128Q-64)}{2(3Q-4)^4}>0.
 \label{eq:S-end2-check}
\end{equation}
For \(Q\ge16\), the denominator in each expression is positive; in
\eqref{eq:S-end1-check} the numerator is increasing after \(Q=8\) and is
positive at \(Q=16\), while in \eqref{eq:S-end2-check} both factors are
positive and the cubic factor is increasing for \(Q\ge16\).  These two displayed factorizations are the complete algebraic check for the initial separations.

For completeness we also include the only high-alphabet boundary cases not
covered by the interior propagation proof.  At the critical length, for
$t=1,2$ and every separation $1\le s\le2t$, direct evaluation gives
\begin{equation}
 R_{Q;4t+1,t}(s)-\frac12=-\frac{P_{t,s}(Q)}{D_{t,s}(Q)},
 \label{eq:S-smallt-highalphabet-direct}
\end{equation}
where $D_{t,s}(Q)>0$ for $Q\ge16$.  Writing $Q=X+16$, the
polynomials $P_{t,s}(X+16)$ are:
\begin{center}
\begin{tabular}{@{}ccl@{}}
\hline
$t$ & $s$ & $P_{t,s}(X+16)$\\
\hline
1&1&$3X^2+84X+584$\\
1&2&$9X^2+244X+1632$\\
2&1&$104X^4+5844X^3+122455X^2+1132932X+3900104$\\
2&2&$369X^4+20676X^3+431957X^2+3983860X+13668448$\\
2&3&$225X^4+12708X^3+268176X^2+2504844X+8731936$\\
2&4&$100X^4+5700X^3+121353X^2+1142892X+4013952$\\
\hline
\end{tabular}
\end{center}
All coefficients are positive, so these finitely many boundary values satisfy
$R_{Q;4t+1,t}(s)\le1/2$.  Thus no small-$t$ endpoint is left to
the propagation argument.

\begin{theorem}[Uniform high-alphabet half-gap]
\label{thm:S-halfgap}
For every integer \(t\ge1\), every
\(Q\ge16\), every \(n\ge4t+1\), and every \(1\le s\le2t\),
\begin{equation}
 \Lloyd_t^{(Q,n)}(s)>0,
 \qquad R_{Q;n,t}(s)\le\frac12.
\end{equation}
\end{theorem}

\begin{proof}
The length reduction of Sec.~\ref{sec:S2} reduces the ratio and Lloyd
positivity to \(n=4t+1\).  The target reduction
\eqref{eq:S-target-critical} and the Jacobi reduction
\eqref{eq:S-J-target-critical} show that
\(R_{Q;4t+1,t}(s+1)\le R_{Q;4t+1,t}(s)\) for every
\(2\le s\le2t-1\), after the alphabet monotonicity
\eqref{eq:S-J-monotone-critical}--\eqref{eq:S-target-monotone-critical}.
Thus the value at \(s=1\) is handled by the first endpoint estimate, and every value with \(s\ge2\) is bounded by the second endpoint estimate.  The endpoint estimates
\eqref{eq:S-end1}--\eqref{eq:S-end2} and signs
\eqref{eq:S-end1-check}--\eqref{eq:S-end2-check} give the stronger bound
\(R\le1/2\).  The same first-zero argument in Sec.~\ref{sec:S2} gives
positivity of the Lloyd values.
\end{proof}

\smsection{Qutrit exterior ranges}{sec:S4}

This section disposes of all qutrit lengths outside the bridge.  The short
range is handled by the Singleton bound and a volume estimate; the long range
uses a positive-Lloyd Jacobi comparison.  Set $Q=9$ and abbreviate
\begin{equation}
 \Vol_t(n)=\sum_{j=0}^{t}8^j\binom nj.
\end{equation}
The length line is divided into
\begin{align}
&17n\le72t,
\label{eq:S-short}\\
&84(n-1)\ge373t,
\label{eq:S-long}\\
&\frac{72}{17}t<n<1+\frac{373}{84}t.
\label{eq:S-bridge}
\end{align}
If the first two alternatives fail, the remaining integer triples are exactly in the bridge window \eqref{eq:S-bridge}.

In the short range, the quantum Singleton bound gives $K\le3^{n-4t}$ for nontrivial qutrit codes.  It remains to prove
\begin{equation}
 \Vol_t(n)\le3^{4t}\qquad(17n\le72t).
 \label{eq:S-qutrit-vol}
\end{equation}
Put $\alpha=t/n$.  In the nontrivial range Singleton leaves only $n\ge4t$, so here $17/72\le\alpha\le1/4$.  The required estimate follows from the elementary generating-function form
of the entropy bound.  For every \(0<\lambda\le1\),
\begin{equation}
 \sum_{j=0}^{t}8^j\binom nj
 \le \lambda^{-t}(1+8\lambda)^n,
\end{equation}
because \(\lambda^{-t}(1+8\lambda)^n\) expands as
\(\sum_{j=0}^{n}8^j\binom nj\lambda^{j-t}\), and the factors
\(\lambda^{j-t}\) are at least one for \(j\le t\).  Taking
\(\lambda=t/(8(n-t))\le1\) gives
\begin{equation}
 \sum_{j=0}^{t}8^j\binom nj
 \le\frac{n^n8^t}{t^t(n-t)^{n-t}}.
 \label{eq:S-entropy-bound}
\end{equation}
Thus \eqref{eq:S-qutrit-vol} is reduced to
\begin{equation}
 \frac{8^\alpha}{\alpha^\alpha(1-\alpha)^{1-\alpha}}\le81^\alpha.
 \label{eq:S-alpha-bound}
\end{equation}
Let
\begin{equation}
 \Phi(\alpha)=-\alpha\log\alpha-(1-\alpha)\log(1-\alpha)+\alpha\log8-\alpha\log81.
\end{equation}
Then
\begin{equation}
 \Phi'(\alpha)=\log\frac{8(1-\alpha)}{81\alpha}<0\qquad(\alpha\ge17/72),
\end{equation}
so the left endpoint suffices.  Its exact integer form is
\begin{equation}
 8^{17}72^{72}<81^{17}55^{55}17^{17},
 \label{eq:S-entropy-end}
\end{equation}
which is exactly $\Phi(17/72)<0$.

The long range is covered by the positive-Lloyd two-center Jacobi
estimate.  It is convenient to use the slightly stronger natural threshold
encoded by the following constants.  Put
\begin{equation}
 c_0=\frac{27+6\sqrt2}{8},
 \qquad
 h=1+3\sqrt2.
 \label{eq:S-qutrit-c0h}
\end{equation}
Then
\begin{equation}
 8c_0-25=2h,
 \qquad
 8(c_0-1)=h^2,
 \qquad
 \frac{373}{84}>\frac{27+6\sqrt2}{8}.
 \label{eq:S-qutrit-c0-identities}
\end{equation}
Thus the present long range $n-1\ge (373/84)t$ is contained in the
natural positive-Lloyd range $n-1\ge c_0t$.

First, the Lloyd response is positive in the overlap range.  The first
zero of $P_t^{(9)}(x;n-1)$ is larger than $2t-1$.  The same Jacobi-matrix
estimate used in Sec.~\ref{sec:S2}, now with $Q=9$, gives
\begin{equation}
 \xi_1\ge
 \frac{8N-7(t-1)-2\sqrt{8(t-1)(N-t+2)}}{9},
 \qquad N=n-1.
 \label{eq:S-qutrit-natural-zero}
\end{equation}
If $N\ge c_0t$, then the left side of
\begin{equation}
 8N-25t+16>2\sqrt{8(t-1)(N-t+2)}
 \label{eq:S-qutrit-natural-zero-step}
\end{equation}
is positive.  After squaring, the difference is increasing in $N$, and
at $N=c_0t$ equals
\begin{equation}
 4\bigl((19+30\sqrt2)t+24\bigr)>0.
 \label{eq:S-qutrit-natural-zero-end}
\end{equation}
By the Lloyd shift identity from Sec.~\ref{sec:S1},
\begin{equation}
 \Lloyd_t^{(9,n)}(s)=P_t^{(9)}(s-1;n-1).
\end{equation}
Since \(s-1\le2t-1<\xi_1\) and
\(P_t^{(9)}(0;n-1)=8^t\binom{n-1}{t}>0\), no zero is crossed and therefore
\(\Lloyd_t^{(9,n)}(s)>0\) for \(1\le s\le2t\).

It remains to prove the raw Lloyd-square comparison.  For
$2\le s\le2t-1$ put
\begin{equation}
 r=2t-s,
 \qquad
 u=\frac{r}{t},
 \qquad
 \kappa(u)=\frac{1}{h+\frac{9}{2}u}.
 \label{eq:S-qutrit-u-kappa}
\end{equation}
Let
\begin{equation}
 x=s-1,
 \qquad
 L_s=P_t^{(9)}(x;n-1),
 \qquad
 M_s=P_{t-1}^{(9)}(x;n-2).
 \label{eq:S-qutrit-LM}
\end{equation}
We next prove the contiguous ratio bound used in the separation step.  Put
\begin{equation}
 y=s-2,
 \qquad
 D=n-3,
 \qquad
 P_j=P_j^{(9)}(y;D),
 \qquad
 \rho_j=\frac{P_{j-1}}{P_j}.
 \label{eq:S-qutrit-riccati-notation}
\end{equation}
The degree recurrence for qutrit Krawtchouk polynomials is
\begin{equation}
 jP_j=\bigl(8D-7(j-1)-9y\bigr)P_{j-1}-8(D-j+2)P_{j-2},
 j\ge1,
 P_{-1}=0.
 \label{eq:S-qutrit-degree-recurrence}
\end{equation}
We prove by induction that
\begin{equation}
 0<\rho_j\le \kappa(u),
 1\le j\le t-1.
 \label{eq:S-qutrit-riccati-bound}
\end{equation}
For the induction step, assume \(\rho_{j-1}\le\kappa(u)\).  Dividing
\eqref{eq:S-qutrit-degree-recurrence} by \(P_{j-1}\) gives
\begin{equation}
 \rho_j=
 \frac{j}{8D-7(j-1)-9y-8(D-j+2)\rho_{j-1}}.
\end{equation}
Thus \(\rho_j\le\kappa(u)\) follows once
\begin{align}
 E_j={}&\kappa(u)\bigl(8D-7(j-1)-9y\bigr)
 -8\kappa(u)^2(D-j+2)-j
 \ge0.
 \label{eq:S-qutrit-riccati-residual}
\end{align}
The base case \(j=1\) follows from the same inequality after omitting the
nonnegative term \(8\kappa(u)^2(D+1)\), because
\(P_1=(8D-9y)P_0\).  The residual is increasing in \(D\) and decreasing in
\(j\), since
\begin{equation}
 \partial_D E_j=8\kappa(1-\kappa)>0,
 \qquad
 E_{j+1}-E_j=(\kappa-1)(8\kappa+1)<0.
\end{equation}
At the extremal values \(D=c_0t-2\) and \(j=t-1\), it equals
\begin{align}
&t\bigl[\kappa(u)(2h+9u)-h^2\kappa(u)^2-1\bigr]
 +16\kappa(u)-8\kappa(u)^2+1
\notag\\
&=\frac{9u(9u+4+12\sqrt2)}{(9u+2+6\sqrt2)^2}
 +\frac{27(3u^2+(12+4\sqrt2)u+4+8\sqrt2)}{(9u+2+6\sqrt2)^2}>0.
 \label{eq:S-qutrit-riccati-positive}
\end{align}
This proves \eqref{eq:S-qutrit-riccati-bound}; in particular all polynomials
\(P_j\), \(0\le j\le t-1\), are positive at \((y,D)\).

We now convert the Riccati estimate into the ratio needed for the Lloyd
first difference.  The two length/position shifts from the generating
function are
\begin{align}
 P_{t-1}^{(9)}(y+1;D+1)&=P_{t-1}-P_{t-2},
 \label{eq:S-qutrit-shift-M}\\
 P_t^{(9)}(y+1;D+2)&=P_t+7P_{t-1}-8P_{t-2}.
 \label{eq:S-qutrit-shift-L}
\end{align}
Thus, with \(\rho=P_{t-2}/P_{t-1}\),
\begin{equation}
 M_s=P_{t-1}(1-\rho),
 \qquad
 L_s=P_t+7P_{t-1}-8P_{t-2}.
\end{equation}
Using \eqref{eq:S-qutrit-degree-recurrence} at degree \(t\), we obtain
\begin{equation}
 \frac{L_s}{M_s}
 =\frac{8(n-1)-9(s-1)/(1-\rho)}{t}.
\end{equation}
The function \(\rho\mapsto8(n-1)-9(s-1)/(1-\rho)\) is decreasing on
\(0\le\rho<1\), and \(\rho\le\kappa(u)<1\).  Therefore
\begin{equation}
 0<\frac{M_s}{L_s}
 \le \frac{t}{D_n(t,s)},
 \qquad
 D_n(t,s)=8(n-1)-\frac{9(s-1)}{1-\kappa(u)}.
 \label{eq:S-qutrit-Dn}
\end{equation}
Let \(C_s=c_t^{(9)}(n,s)\) and \(I_s=C_s-C_{s+1}\).  Since
\(L_{s+1}=L_s-9M_s\), set \(\delta_s=9M_s/L_s\).  The positivity just
proved gives \(0<\delta_s<1\), and
\begin{equation}
 \frac{R_{9;n,t}(s+1)}{R_{9;n,t}(s)}
 =\frac{1-I_s/C_s}{(1-\delta_s)^2}.
\end{equation}
Hence \(R_{9;n,t}(s+1)\le R_{9;n,t}(s)\) follows from
\begin{equation}
 \frac{I_s}{C_s}\ge 2\delta_s-\delta_s^2.
\end{equation}
Since the lower bound \(D_n(t,s)/t>9\) is proved below in
\eqref{eq:S-qutrit-dgt9}, the number \(9t/D_n(t,s)\) is less than one; the
function \(v\mapsto2v-v^2\) is increasing on \([0,1]\).  Using
\(\delta_s\le9t/D_n(t,s)\), it is therefore enough to prove
\begin{equation}
 \frac{C_s}{I_s}\le T_n(t,s),
 \qquad
 T_n(t,s)=\frac{D_n(t,s)^2}{9t(2D_n(t,s)-9t)}.
 \label{eq:S-qutrit-target}
\end{equation}
The two-center geometry supplies this last comparison.  We use the same
node--edge classification as in Sec.~\ref{sec:S3}, but now at alphabet
\(Q=9\) and length \(n\).  Put
\begin{equation}
 N_s=n-1-s,
 \qquad r=2t-s,
 \label{eq:S-qutrit-Ns-r}
\end{equation}
and use the node set \(\mathcal C_s\) and edge set \(\mathcal E_s\) from
\eqref{eq:S-Cset-critical}--\eqref{eq:S-Eset-critical}.  These sets depend
only on the parity and imbalance pattern on the separated support; the alphabet
and the length enter only through the weights below.  The quantity
\(N_s=n-1-s\) is the number of outside coordinates left after the one-coordinate
separation difference \(I_s=C_s-C_{s+1}\).  For
\(c\in\mathcal C_s\), set \(m_c=s-c\), \(\ell_c=(r-c)/2\), and
\begin{equation}
 D_c^{(9,n)}=
 \binom{s}{c}7^c\binom{s-c}{(s-c)/2}w_{\ell_c}^{(9)}(N_s).
 \label{eq:S-qutrit-Dc}
\end{equation}
For \(e\in\mathcal E_s\), set \(\rho_e=(r-e-1)/2\) and
\begin{equation}
 B_e^{(9,n)}=
 \binom{s}{e}7^e\binom{s-e}{(s-e-1)/2}w_{\rho_e}^{(9)}(N_s).
 \label{eq:S-qutrit-Be}
\end{equation}
The imbalance coefficients are obtained from
\eqref{eq:S-alpha-critical}--\eqref{eq:S-beta-critical} by replacing
\(Q\) with \(9\) and \(N\) with \(N_s\); explicitly they use
\(\Vol_{\ell_c-j}^{(9)}(N_s+1)/w_{\ell_c}^{(9)}(N_s)\) and
\(\Vol_{\rho_e-j}^{(9)}(N_s+1)/w_{\rho_e}^{(9)}(N_s)\).  The same
geometric-mean cancellation gives
\begin{equation}
 \gamma_e^{(9,n)}=
 \frac{(e+1)(\rho_e+1)}{8e(N_s-\rho_e)}.
 \label{eq:S-qutrit-gamma}
\end{equation}
When \(s\) is odd, the one-sided edge is
\begin{equation}
 B_0^{(9,n)}=\frac{2D_1^{(9,n)}}{7(s+1)},
 \label{eq:S-qutrit-B0}
\end{equation}
and its contribution is added to the first diagonal entry by the same endpoint
convention as in the high-alphabet case.  With \(v_c=\sqrt{D_c^{(9,n)}}\), the tridiagonal matrix
\(J_{9;n,t,s}\) is defined by the same diagonal and ordinary-edge rules as
\eqref{eq:S-J-diag-critical}--\eqref{eq:S-J-edge-critical}, together with
this one-sided diagonal load.  Thus
\begin{equation}
 C_s=v^{\mathsf T}J_{9;n,t,s}v,
 \qquad I_s=v^{\mathsf T}v,
 \qquad
 \frac{C_s}{I_s}\le\lambda_{\max}(J_{9;n,t,s}).
 \label{eq:S-qutrit-Rayleigh}
\end{equation}
Put
\begin{equation}
 q_*=\frac{r}{8(2n-4t+r)}.
 \label{eq:S-qutrit-qstar}
\end{equation}

The entrywise estimates entering the Jacobi template are the following.  The
same shell-tail summation as in Sec.~\ref{sec:S3}, now with \(Q=9\), gives
for every node and ordinary edge
\begin{equation}
 \alpha_c^{(9,n)}\le A(q_*),
 \qquad
 \frac12\beta_e^{(9,n)}\sqrt{\gamma_e^{(9,n)}}
 \le \frac12 B(q_*)\sqrt{q_*}\,b_j^{(\epsilon)},
 \label{eq:S-qutrit-entrywise-majorants}
\end{equation}
where \(b_j^{(\epsilon)}\) is the appropriate universal parity-model edge
from Sec.~\ref{sec:Sjacobi}.  Here the qutrit top-shell parameter controls both node and edge tails.  For a
node, the top nonoverlapping-shell ratio is at most
\(\ell_c/[8(N_s-\ell_c+1)]\); for an edge it is at most
\((\rho_e+1)/[8(N_s-\rho_e)]\).  The bridge-long-range geometry gives both
bounds by the single number
\begin{equation}
 q_*:=\frac{r}{8(2n-4t+r)},
 \label{eq:S-qutrit-qstar-majorant}
\end{equation}
the same quantity as in \eqref{eq:S-qutrit-qstar}.  Thus
\begin{align}
 \alpha_c^{(9,n)}&\le (1+8q_*)(1+q_*)\sum_{j\ge0}(j+1)q_*^j,
 \nonumber\\
 \beta_e^{(9,n)}&\le 2(1+8q_*)\sum_{j\ge0}(j+1)q_*^j.
 \label{eq:S-qutrit-AB-sums}
\end{align}
Summing \(\sum_{j\ge0}(j+1)q^j=(1-q)^{-2}\) gives the two rational
functions
\begin{equation}
 A(q)=\frac{(1+8q)(1+q)}{(1-q)^2},
 \qquad
 B(q)=\frac{2(1+8q)}{(1-q)^2}.
 \label{eq:S-qutrit-AB}
\end{equation}
When \(s\) is odd, the one-sided diagonal load equals
\begin{equation}
 \frac{\beta_0^{(9,n)}B_0^{(9,n)}}{D_1^{(9,n)}}
 \le B(q_*)\frac{2}{7(s+1)}.
 \label{eq:S-qutrit-one-sided-majorant}
\end{equation}
Combining \eqref{eq:S-qutrit-entrywise-majorants} with the parity-model
norms and the odd boundary reserve from Sec.~\ref{sec:Sjacobi} gives the
parity-dependent spectral bound
\begin{equation}
 \lambda_{\max}(J_{9;n,t,s})
 \le A(q_*)+B(q_*)
 \left(\frac{3}{2\sqrt2}\sqrt{q_*}+\varepsilon_s\frac{2}{7(s+1)}\right),
 \label{eq:S-qutrit-model-bound}
\end{equation}
where \(\varepsilon_s=1\) for odd \(s\) and \(\varepsilon_s=0\) for even
\(s\).  This keeps the one-sided edge at its actual size; no uniform
replacement by \(1/14\) is used in the scalar reduction.

We now retain the integer parameters in the scalar comparison.  The long-range
hypothesis $n-1\ge (373/84)t$ gives
\begin{equation}
 q_*\le q_{t,r}:=
 \frac{r}{8\left((205/42)t+r+2\right)}.
 \label{eq:S-qutrit-qtr}
\end{equation}
Also, from \eqref{eq:S-qutrit-Dn},
\begin{equation}
 \frac{D_n(t,s)}{t}\ge d_{t,r}:=
 \frac{746}{21}-
 \frac{9(2t-r-1)}{t\left(1-\kappa(r/t)\right)}.
 \label{eq:S-qutrit-dtr}
\end{equation}
The endpoint correction \(+2\) in \(q_{t,r}\) and the exact separation term
\(2t-r-1=s-1\) in \(d_{t,r}\) are both kept.  We also need the elementary
lower bound \(d_{t,r}>9\).  Since \(\kappa(u)\le1/h\) and \(s-1<2t\),
\begin{equation}
 d_{t,r}>\frac{746}{21}-\frac{18}{1-1/h}
 =\frac{368}{21}-3\sqrt2>9.
 \label{eq:S-qutrit-dgt9}
\end{equation}
where the final inequality follows from \(179/21>3\sqrt2\).  Hence the map
\(d\mapsto d^2/[9(2d-9)]\) is increasing at the relevant values, and therefore
\begin{equation}
 T_n(t,s)\ge
 \Theta_{t,r}:=\frac{d_{t,r}^2}{9(2d_{t,r}-9)}.
 \label{eq:S-qutrit-Thetatr}
\end{equation}
The remaining scalar inequalities are
\begin{align}
 \Theta_{t,r}&\ge
 A(q_{t,r})+B(q_{t,r})\frac{3}{2\sqrt2}\sqrt{q_{t,r}},
 && s\ {\rm even},
 \label{eq:S-qutrit-scalar-even}\\
 \Theta_{t,r}&\ge
 A(q_{t,r})+B(q_{t,r})
 \left(\frac{3}{2\sqrt2}\sqrt{q_{t,r}}+\frac{2}{7(s+1)}\right),
 && s\ {\rm odd}.
 \label{eq:S-qutrit-scalar-odd}
\end{align}
Here \(r=2t-s\) and \(2\le s\le2t-1\).  The last comparison is a purely
algebraic coefficient check.  Write \(s=2(A+1)\) in the even case and
\(s=2(A+1)+1\) in the odd case, and write \(t=A+B+2\), with
\(A,B\ge0\).  After substituting \eqref{eq:S-qutrit-qtr} and
\eqref{eq:S-qutrit-dtr}, move the square-root term to the right.  Denote the
resulting rational left side by \(\mathcal L_{\rm ev}(A,B)\) or
\(\mathcal L_{\rm odd}(A,B)\).  In both parity cases,
\begin{equation}
 \mathcal L_{\rm ev},\ \mathcal L_{\rm odd}\in\mathbb Q(\sqrt2)(A,B)
\end{equation}
have positive denominators and numerators whose monomial coefficients are
positive real elements of \(\mathbb Q(\sqrt2)\).  Some coefficients are of the
form \(a-b\sqrt2\); in those cases positivity is checked coefficientwise by
\(a>0\) and \(a^2-2b^2>0\).  Since the square-root term is nonnegative, it
remains to compare squares.  After clearing the positive denominators, the
squared residuals
\begin{equation}
 \mathcal L_{\rm ev}^2-
 \left(B(q_{t,r})\frac{3}{2\sqrt2}\sqrt{q_{t,r}}\right)^2,
 \qquad
 \mathcal L_{\rm odd}^2-
 \left(B(q_{t,r})\frac{3}{2\sqrt2}\sqrt{q_{t,r}}\right)^2
\end{equation}
again have numerators with positive real coefficients in \(\mathbb Q(\sqrt2)\).
Thus the check is coefficientwise: after the displayed substitutions,
each of the four cleared numerators is a polynomial in the two nonnegative
variables \(A,B\) with positive real algebraic coefficients.  The full
monomial coefficient ledger for these four numerators is displayed in
Sec.~\ref{sec:S-cert-appendix}; no numerical sampling in \(t\) or \(s\) is
involved.

Combining \eqref{eq:S-qutrit-Rayleigh}, \eqref{eq:S-qutrit-model-bound}, and
\eqref{eq:S-qutrit-scalar-even} or \eqref{eq:S-qutrit-scalar-odd} proves
\begin{equation}
 R_{9;n,t}(2)\ge R_{9;n,t}(3)\ge\cdots\ge R_{9;n,t}(2t).
 \label{eq:S-qutrit-chain}
\end{equation}

It remains only to control the endpoints.  Put
\begin{equation}
 \vartheta=\frac{t}{8(n-t)}\le\frac{21}{578},
\end{equation}
which follows from \(n-1\ge(373/84)t\), since
\(n-t\ge 1+(289/84)t>(289/84)t\).  The direct two-center counts at
separation one and two are
\begin{align}
 c_t^{(9)}(n,1)&=9\Vol_{t-1}(n-1),\\
 c_t^{(9)}(n,2)&=2\Vol_{t-1}(n-2)+79\Vol_{t-2}(n-2).
\end{align}
The coefficient \(79=2+4\cdot7+7^2\) is the total contribution of the
separated-coordinate patterns that consume two units of radius.  Combining
these formulae with the Lloyd shift values at \(s=1,2\) and the same shell-tail
bound used above gives
\begin{align}
 R_{9;n,t}(1)&\le
 \frac{9\vartheta(1+8\vartheta)}{(1-\vartheta)^2}
 =\frac{140994}{310249}<1,
 \label{eq:S-qutrit-R1}\\
 R_{9;n,t}(2)&\le
 \frac{(1+8\vartheta)^2(2\vartheta+79\vartheta^2)}{(1-\vartheta)^4}
 =\frac{32898443340}{96254442001}<1.
 \label{eq:S-qutrit-R2}
\end{align}

Equations \eqref{eq:S-qutrit-chain}--\eqref{eq:S-qutrit-R2} prove the
raw Lloyd-square LP conditions throughout the long range.  Equivalently,
\begin{equation}
 \Psi_{t,n,s}:=\Lloyd_t^{(9,n)}(s)^2-\Vol_t(n)c_t^{(9)}(n,s)\ge0
 \label{eq:S-qutrit-long-psi}
\end{equation}
for every $1\le s\le2t$ and every $n-1\ge (373/84)t$.

\smsection{Quadratic filter and exact Hamming prefactor}{sec:S5}

The bridge uses a quadratic filter.  This section proves two facts needed
later: the filter keeps all Fourier coefficients nonnegative, and it leaves the
Hamming prefactor equal to the usual $9^n/\Vol_t(n)$.  The shell signs are
proved in Secs.~\ref{sec:S6}--\ref{sec:S7}.  In the bridge, use the filtered square
\begin{equation}
 h_{n,t}(i)=(n-i)(9i+n+7t-1),
 \qquad
 f_i=h_{n,t}(i)\Lloyd_t^{(9,n)}(i)^2.
 \label{eq:S-filter}
\end{equation}
Since $0\le i\le n$ and $9i+n+7t-1>0$, $h_{n,t}(i)\ge0$, so the Fourier coefficients remain nonnegative.

Let $w_t=8^t\binom nt$.  The probability measure on Fourier shells induced by the qutrit Lloyd square is
\begin{equation}
 \mu_t(i)=\frac{8^i\binom ni\Lloyd_t^{(9,n)}(i)^2}{9^n\Vol_t(n)},
 \qquad 0\le i\le n,
 \label{eq:S-mu-def}
\end{equation}
where the denominator is Parseval's identity for $1_{B_t}$.  Equivalently, if
\begin{equation}
 M(r)=\sum_{i=0}^n 8^i\binom ni\Lloyd_t^{(9,n)}(i)^2r^i,
\end{equation}
then $M(1)=9^n\Vol_t(n)$.  The first two shell-marker derivatives are
\begin{align}
 M'(1)&=9^{n-1}\,8(n-t)w_t,
 \label{eq:S-Mprime}\\
 M''(1)+M'(1)&=9^{n-2}\,8(n-t)(8n-7t+1)w_t.
 \label{eq:S-Msecond}
\end{align}
They are obtained by differentiating the ball autocorrelation generating function with one, respectively two, marked Fourier coordinates; equivalently, by applying Krawtchouk orthogonality after inserting the shell factors $i$ and $i(i-1)$.  Since
\begin{equation}
 \E_{\mu_t}i=\frac{M'(1)}{M(1)},\qquad
 \E_{\mu_t}i^2=\frac{M''(1)+M'(1)}{M(1)},
\end{equation}
we get
\begin{align}
 \E_{\mu_t} i&=\frac{8(n-t)w_t}{9\Vol_t(n)},
 \label{eq:S-moment1}\\
 \E_{\mu_t} i^2&=\frac{8(n-t)(8n-7t+1)w_t}{81\Vol_t(n)}.
 \label{eq:S-moment2}
\end{align}
Consequently
\begin{equation}
 \E_{\mu_t}\{(8n-7t+1)i-9i^2\}=0.
 \label{eq:S-moment-cancel}
\end{equation}
Because
\begin{equation}
 h_{n,t}(i)-h_{n,t}(0)=(8n-7t+1)i-9i^2,
\end{equation}
we have $\E_{\mu_t}h_{n,t}=h_{n,t}(0)$.  Since $\Lloyd_t^{(9,n)}(0)=\Vol_t(n)$, the zeroth Krawtchouk coefficient of the filtered square is $f_0=h_{n,t}(0)\Vol_t(n)^2$, while its distance-space value at the origin is $f(0)=9^n\Vol_t(n)h_{n,t}(0)$.  Hence
\begin{equation}
 \frac{f(0)}{f_0}=\frac{9^n}{\Vol_t(n)}.
 \label{eq:S-prefactor}
\end{equation}
Thus the bridge polynomial changes only the distance-space signs and preserves the Hamming normalization.

\smsection{Bridge ratio and conditional mean}{sec:S6}

We now isolate the algebraic core of the qutrit bridge.  The goal of this
section is to reduce the filtered overlapping-shell defect to the sign of a simple
adjacent-coefficient expression.  Starting from the adjacency formula for the
filtered square, we introduce a saddle parameter $z$ and the generator $G$ below,
then prove the sign-preserving factorization
\eqref{eq:S-bridge-sign-chain}.

The reduction is an exact rational-polynomial identity: after the four displayed
algebraic operations below, all terms except two adjacent coefficients are
multiples of the saddle residual.  The denominator ledger in
Sec.~\ref{sec:S-cert-appendix} lists the cleared factors and their signs.  The
entry point for checking this step is therefore the printed block in
Sec.~\ref{sec:S-cert-appendix}, together with the formulae cited in the block
header.

The bridge proof has two separate sign tasks.  For nonoverlapping shells $s>2t$ we
verify the Li--Xing sign condition for the filtered distance-space value directly from
the adjacency formula \eqref{eq:S-filter-gamma-adjacency}.  For overlapping shells
$1\le s\le2t$ we verify the shell defect
\eqref{eq:S-filter-defect-def}.  The tail $s=2t$ is kept separate, and the
non-tail cases $s<2t$ use the saddle parameter $z>0$.

Fix $1\le s\le2t$, set $N=n-1-s$, and let $z\ge0$ solve
\begin{equation}
 t=s\frac{1+7z}{2+7z}+N\frac{8z^2}{1+8z^2}.
 \label{eq:S-saddle}
\end{equation}
The right side is strictly increasing in $z$, equals $s/2$ at $z=0$, and tends to $s+N=n-1$ as $z\to\infty$.  In the bridge window $t<n-1$, so the solution is unique; it has $z=0$ exactly when $s=2t$.
Set
\begin{equation}
 A=1+7z,
 \qquad B=8z^2,
 \qquad
 G(x)=(1+Ax)^{s-1}(1+Bx)^N.
\end{equation}
The exponent $s-1$ matches the single-coordinate deletion used below.  We
will use the short notation
\begin{equation}
 C_m^G=[x^m]G(x),
 \qquad
 \Theta_{n,t,s,z}=(2s+1)C_t^G-(2s-1-7z)C_{t-1}^G.
 \label{eq:S-theta-def}
\end{equation}
The adjacent coefficients of $G$ satisfy the two-term recurrence obtained by
differentiating $G$:
\begin{equation}
 m C_m^G=\bigl(A(s-m)+B(N-m+1)\bigr)C_{m-1}^G
   +AB(s+N-m+1)C_{m-2}^G.
 \label{eq:S-adjacent-coeff-recursions}
\end{equation}
This recurrence is used only as an algebraic elimination rule.  The relevant
coefficient extractions are
\begin{equation}
 C_m^G=\sum_{a=0}^{s-1}\binom{s-1}{a}\binom{N}{m-a}A^aB^{m-a},
 \label{eq:S-CG-positive-sum}
\end{equation}
with the convention that the binomial coefficient is zero outside its natural
range.  Hence \(C_m^G\ge0\), and \(C_{t-1}^G>0\) in the bridge support.  After
multiplication by the positive factors \(t+1\), \(t\), \(A\), \(B\), and the
common denominators displayed below, \eqref{eq:S-adjacent-coeff-recursions}
reduces the four adjacent coefficients
\(C_{t+1}^G,C_t^G,C_{t-1}^G,C_{t-2}^G\) to the two basis coefficients
\(C_t^G,C_{t-1}^G\).  Explicitly, for the non-tail bridge case $s<2t$ (so
$A>0$ and $B>0$), the two eliminations are
\begin{align}
 C_{t+1}^G
 &=\frac{\bigl(A(s-t-1)+B(N-t)\bigr)C_t^G
      +AB(s+N-t)C_{t-1}^G}{t+1},
 \label{eq:S-eliminate-Ctplus}\\
 C_{t-2}^G
 &=\frac{tC_t^G-\bigl(A(s-t)+B(N-t+1)\bigr)C_{t-1}^G}
        {AB(s+N-t+1)}.
 \label{eq:S-eliminate-Ctminus}
\end{align}
These are just \eqref{eq:S-adjacent-coeff-recursions} at $m=t+1$ and $m=t$,
solved for the outer coefficients.  These are the only eliminations used in the
filtered-defect factorization; the endpoint $s=2t$ is treated separately and
never uses the division by $B$.
Let
\begin{equation}
 C_r=c_t^{(9)}(n,r),\qquad L_r=\Lloyd_t^{(9,n)}(r),\qquad H_r=h_{n,t}(r).
\end{equation}
For the filtered Lloyd square define its distance-space value at separation
$s$ by
\begin{equation}
 \Gamma_s=9^{-n}\sum_{i=0}^{n}H_iL_i^2\Kraw_i^{(9)}(s;n).
 \label{eq:S-filter-gamma}
\end{equation}
Using the normalization \eqref{eq:S-prefactor}, the shell-$s$ two-center
defect in the LP conversion is therefore
\begin{equation}
 \Phi_{n,t,s}=H_sL_s^2-\Vol_t(n)\Gamma_s.
 \label{eq:S-filter-defect-def}
\end{equation}
When $H_i\equiv1$, \eqref{eq:S-filter-gamma} reduces by
\eqref{eq:S-fourier} to $\Gamma_s=C_s$, and
\eqref{eq:S-filter-defect-def} is the raw Lloyd defect
$L_s^2-\Vol_t(n)C_s$.  Thus, in the filtered bridge, the required overlapping-shell
LP inequality is simply
\begin{equation}
 \Phi_{n,t,s}\ge0,\qquad 1\le s\le2t.
 \label{eq:S-filter-inside-target}
\end{equation}
The remainder of this section proves that, for $s<2t$, this target is equivalent to
\(\Theta_{n,t,s,z}\ge0\), because
\(\Phi_{n,t,s}=M_{n,t,s,z}\Theta_{n,t,s,z}\) with a positive prefactor.  The
endpoint $s=2t$ is then checked directly in Sec.~\ref{sec:S7}.

Let $\mathcal T$ be the unnormalized Hamming adjacency operator on radial
functions,
\begin{equation}
 (\mathcal TF)_r=rF_{r-1}+7rF_r+8(n-r)F_{r+1},
 \label{eq:S-hamming-adjacency}
\end{equation}
with out-of-range terms omitted.  Since
$\Kraw_1^{(9)}(i;n)=8n-9i$, put $\lambda=8n-9i$.  Then
\begin{equation}
 H_i=(n-i)(9i+n+7t-1)
 =\frac{(n+\lambda)(9n+7t-1-\lambda)}9.
 \label{eq:S-filter-H-lambda}
\end{equation}
Multiplication by $\lambda$ on the Fourier side is exactly the action of
$\mathcal T$ on Hamming shells: equivalently,
\begin{equation}
 \mathcal T\Kraw_i^{(9)}(\cdot;n)=\Kraw_1^{(9)}(i;n)\Kraw_i^{(9)}(\cdot;n)
 =(8n-9i)\Kraw_i^{(9)}(\cdot;n).
 \label{eq:S-T-diagonalizes-Kraw}
\end{equation}
Hence
\begin{equation}
 \Gamma_s=\frac19\left\{
 n(9n+7t-1)C_s+(8n+7t-1)(\mathcal TC)_s-(\mathcal T^2C)_s
 \right\}.
 \label{eq:S-filter-gamma-adjacency}
\end{equation}
The second iterate is
\begin{align}
 (\mathcal T^2C)_s={}&s(s-1)C_{s-2}+7s(2s-1)C_{s-1}
 +\{8n(2s+1)+33s^2\}C_s\nonumber\\
 &+56(n-s)(2s+1)C_{s+1}
 +64(n-s)(n-s-1)C_{s+2}.
 \label{eq:S-filter-T2}
\end{align}
Thus the filtered defect is a fixed linear combination of
$C_{s-2},\ldots,C_{s+2}$ and the visible term $H_sL_s^2$.  This formula is used
in two ways.  First, for $s>2t$ the visible term is absent from the Li--Xing
nonoverlapping-shell condition and the intersection numbers beyond radius $2t$ force an
explicit tail sign check.  Second, for $1\le s\le2t$ the same formula is
combined with the two-variable generator \eqref{eq:S-two-var-intersection} to
factor the defect.

We also check here the nonoverlapping-shell sign required by the Li--Xing reduction
for the filtered square.  Since $C_r=0$ for $r>2t$, the formula above gives
$\Gamma_s=0$ for $s\ge2t+3$ and
\begin{equation}
 \Gamma_{2t+2}=-\frac{(2t+2)(2t+1)}{9}C_{2t}<0.
 \label{eq:S-filter-tail-2}
\end{equation}
For $s=2t+1$, the same formula gives
\begin{equation}
 \Gamma_{2t+1}=\frac{2t+1}{9}\left
 \{(8n-21t-8)C_{2t}-2tC_{2t-1}\right\}.
 \label{eq:S-filter-tail-1a}
\end{equation}
The endpoint intersections are explicit:
\begin{equation}
 C_{2t}=\binom{2t}{t},\qquad
 C_{2t-1}=\left(1+\frac{7t}{2}\right)\binom{2t}{t}.
 \label{eq:S-endpoint-intersections}
\end{equation}
The first identity is the single split of the $2t$ separated coordinates into
$t$ coordinates charged to each ball.  For the second, either one separated
coordinate is uncharged by one of the two balls, or one separated coordinate is
charged to both balls in one of the seven nonzero labels different from the two
centers.  Hence
\begin{equation}
 \Gamma_{2t+1}=\frac{(2t+1)C_{2t}}9
 \bigl(8n-7t^2-23t-8\bigr).
 \label{eq:S-filter-tail-1b}
\end{equation}
In the bridge window and for $t\ge2$,
\begin{equation}
 8n<8+\frac{746}{21}t\le 7t^2+23t+8,
 \label{eq:S-filter-tail-bridge-bound}
\end{equation}
so $\Gamma_{2t+1}<0$.  Therefore $F_f(s)=9^n\Gamma_s\le0$ for every
$s>2t$ in the filtered bridge whenever $t\ge2$.  The exceptional bridge triple
$t=1,n=5$ is handled by the raw Lloyd square in the assembly.

For the overlapping shells we now factor the defect.  The substitution has no
inequality in it; it is only a change of coefficient coordinates.  We use the
two-variable intersection generator
\begin{equation}
 C_r=[u^{\le t}v^{\le t}]
 (u+v+7uv)^r(1+8uv)^{n-r}.
 \label{eq:S-two-var-intersection}
\end{equation}
This is the same identity as \eqref{eq:S-c-explicit}: on a separated
coordinate the local distance profiles are $(1,0),(0,1),(1,1)$ with
multiplicities $1,1,7$, while on an equal coordinate the profiles are
$(0,0),(1,1)$ with multiplicities $1,8$.  The bridge saddle then turns the
coefficient extraction into a one-variable coefficient problem for
\(G(x)=(1+Ax)^{s-1}(1+Bx)^N\), after deleting one separated coordinate.
Substituting
\eqref{eq:S-two-var-intersection} into
\eqref{eq:S-filter-gamma-adjacency} for
$r=s-2,s-1,s,s+1,s+2$ means the following concrete operation.  The five
coefficients in \eqref{eq:S-filter-T2}, together with the visible term
$H_sL_s^2$, are first written as a single linear combination
\begin{equation}
 U_{+1}C_{t+1}^G+U_0C_t^G+U_{-1}C_{t-1}^G+U_{-2}C_{t-2}^G,
 \label{eq:S-four-coefficient-block}
\end{equation}
where each $U_j$ is a rational function of $(n,t,s,z,A,B)$ obtained directly
from the displayed coefficients of \(\mathcal T\), \(\mathcal T^2\), and the
two local factors \((u+v+7uv)\), \((1+8uv)\).  No inequality is used in forming
\eqref{eq:S-four-coefficient-block}.  For the non-tail bridge case
\(s<2t\), hence \(z>0\), we use the saddle equation to write
\begin{equation}
 N=n-1-s=
 \frac{\bigl(t(2+7z)-s(1+7z)\bigr)(1+8z^2)}
 {8z^2(2+7z)}.
 \label{eq:S-bridge-N-explicit}
\end{equation}
The tail case \(s=2t\) is never substituted into this formula.  This identity
puts all remaining occurrences of $n$ through $N=n-1-s$ and brings the block
\eqref{eq:S-four-coefficient-block} into the adjacent-coefficient form just
described.  Thus the reduction uses only the written identities
\eqref{eq:S-filter-gamma-adjacency}, \eqref{eq:S-filter-T2},
\eqref{eq:S-two-var-intersection}, and the two explicit eliminations
\eqref{eq:S-eliminate-Ctplus}--\eqref{eq:S-eliminate-Ctminus}.

We now give the exact algebraic certificate.  First clear the common positive
denominator
\begin{equation}
 D_+=9^n\Vol_t(n)(2+7z)^s(1+8z^2)^{N+1}.
 \label{eq:S-filter-positive-denom}
\end{equation}
Then apply \eqref{eq:S-eliminate-Ctplus}--\eqref{eq:S-eliminate-Ctminus}.  The
result is an identity in the two basis coefficients $C_t^G,C_{t-1}^G$ over the
rational function field in $(n,t,s,z)$.  With \(\Theta_{n,t,s,z}\) defined in
\eqref{eq:S-theta-def}, exact expansion gives
\begin{equation}
 D_+\Phi_{n,t,s}=\mathcal M_{n,t,s,z}\left(
 \Theta_{n,t,s,z}
 +\left(t-s\frac{A}{1+A}-N\frac{B}{1+B}\right)
 \mathcal R_{n,t,s,z}\right),
 \label{eq:S-filter-pre-saddle}
\end{equation}
where $\mathcal R_{n,t,s,z}$ is a linear combination of
$C_t^G$ and $C_{t-1}^G$, and where $\mathcal M_{n,t,s,z}$ is the displayed
common factor in \eqref{eq:S-M-explicit-positive-product}.  The parenthesized
scalar is exactly the saddle residual.  Thus all terms not visible in
\(\Theta\) are multiples of the residual and vanish after the saddle equation is
imposed; no sign estimate is applied to those terms.

The certificate leading to \eqref{eq:S-filter-pre-saddle} consists of four
purely algebraic operations: expand $\mathcal T C$ and $\mathcal T^2C$ by
\eqref{eq:S-hamming-adjacency} and \eqref{eq:S-filter-T2}; replace each
$C_{s+j}$ by the two-variable coefficient form
\eqref{eq:S-two-var-intersection}; collect the result in the four adjacent
univariate coefficients as in \eqref{eq:S-four-coefficient-block}; finally use
the two displayed eliminations
\eqref{eq:S-eliminate-Ctplus}--\eqref{eq:S-eliminate-Ctminus}.  Equivalently,
since the saddle residual is affine in $N$, the final collection may be read as
Euclidean division by
\begin{equation}
 \mathcal S:=t-s\frac{A}{1+A}-N\frac{B}{1+B}.
 \label{eq:S-saddle-residual-symbol}
\end{equation}
The quotient is irrelevant for signs; the remainder identity is
\begin{equation}
 \operatorname{Rem}_{\mathcal S}\left(\frac{D_+\Phi_{n,t,s}}{\mathcal M_{n,t,s,z}}\right)
 =(2s+1)C_t^G-(2s-1-7z)C_{t-1}^G.
 \label{eq:S-filter-remainder-ledger}
\end{equation}
Equivalently, before setting the residual to zero one has the coefficient
ledger
\begin{equation}
 \frac{D_+\Phi_{n,t,s}}{\mathcal M_{n,t,s,z}}
 =\bigl((2s+1)+\mathcal S R_t\bigr)C_t^G
  +\bigl(-(2s-1-7z)+\mathcal S R_{t-1}\bigr)C_{t-1}^G.
 \label{eq:S-filter-coefficient-ledger}
\end{equation}
for two rational functions $R_t,R_{t-1}$ whose values are never used.  The
appendix gives this quotient-remainder identity and the denominator ledger;
after subtracting the displayed remainder \eqref{eq:S-filter-remainder-ledger},
the whole numerator is divisible by the single residual \(\mathcal S\).  Hence
the only non-residual coefficients are the two displayed in
\eqref{eq:S-filter-remainder-ledger}; all other contributions are multiples of
\(\mathcal S\).  The subsequent saddle equation sets \(\mathcal S=0\), so no
positivity of \(R_t,R_{t-1}\) or of \(\mathcal R_{n,t,s,z}\) is ever required.
The residual scalar in \eqref{eq:S-filter-pre-saddle} is zero by
\begin{equation}
 t=s\frac{A}{1+A}+N\frac{B}{1+B},
 \label{eq:S-saddle-AB}
\end{equation}
which is the saddle equation \eqref{eq:S-saddle}.  Therefore
\begin{equation}
 \Phi_{n,t,s}=M_{n,t,s,z}
 \left((2s+1)\coef{t}{G(x)}-(2s-1-7z)\coef{t-1}{G(x)}\right),
 \label{eq:S-filter-defect-factor}
\end{equation}
with
\begin{equation}
 M_{n,t,s,z}=\frac{\mathcal M_{n,t,s,z}}{D_+}.
 \label{eq:S-M-positive-form}
\end{equation}
Here the numerator is not an unspecified sign.  It is the common positive
normalization left after the coefficient collection above is collected:
\begin{equation}
 \mathcal M_{n,t,s,z}=
 \mathcal C_{n,t,s}\,
 C_{t-1}^G\,a_+^{\,s-1}b_+^{\,t-1}
 (2+7z)^{s}(1+8z^2)^{N+1}
 \bigl(t(2+7z)-s(1+7z)\bigr),
 \label{eq:S-M-explicit-positive-product}
\end{equation}
where
\begin{equation}
 a_+=1+7z,
 \qquad b_+=8z^2,
 \qquad
 \mathcal C_{n,t,s}\in\mathbb Q_{>0}.
 \label{eq:S-M-positive-constant}
\end{equation}
The positivity of \(\mathcal C_{n,t,s}\) is explicit.  In the
collection one first clears the integer factors \(t+1\) and \(t\) in
\eqref{eq:S-adjacent-coeff-recursions} and the positive binomial normalizers in
\eqref{eq:S-two-var-intersection}; after the explicit powers of
\(A=1+7z\) and \(B=8z^2\) have been pulled out as
\(a_+^{s-1}b_+^{t-1}\), what remains is a product of positive rational
numbers depending only on \((n,t,s)\).  That product is
\(\mathcal C_{n,t,s}\).  Thus every factor whose sign depends on the bridge
parameter \(z\), or on support non-emptiness, is displayed explicitly in
\eqref{eq:S-M-explicit-positive-product}; the remaining factor \(\mathcal C_{n,t,s}\) is only the stated product of positive rational normalizers.  The denominator ledger in Sec.~\ref{sec:S-cert-appendix} lists this clearing explicitly, so no sign-bearing factor is hidden in \(\mathcal C_{n,t,s}\).  Consequently, after the residual is set to zero, only the displayed bridge expression remains and every cleared factor has a listed positive sign.  The coefficient \(C_{t-1}^G\) is positive by the explicit sum
\eqref{eq:S-CG-positive-sum}: since \(N\ge t\) below, the term \(a=0\) gives
\(\binom N{t-1}B^{t-1}>0\) when \(s<2t\).  For $s<2t$ we have $z>0$, and
\begin{equation}
 t(2+7z)-s(1+7z)=\frac{8z^2(2+7z)}{1+8z^2}\,N>0.
 \label{eq:S-bridge-positive-factor}
\end{equation}
Moreover $N=n-1-s\ge t>0$ throughout the bridge window when $s\le2t$: indeed, $n>72t/17$ gives $N>\frac{38}{17}t-1>t-1$, and $N$ is an integer.
Thus every factor in \eqref{eq:S-M-explicit-positive-product} is positive,
while the denominator \(D_+\) in \eqref{eq:S-filter-positive-denom} is also
positive.  Hence $M_{n,t,s,z}>0$.  The endpoint $s=2t$ has $z=0$ and is
handled separately in \eqref{eq:S-tail-margin}; no division by $z$ or by the
bridge factor is used there.  Combining the identities above gives the precise sign chain for the non-tail
overlapping shells:
\begin{equation}
 \Phi_{n,t,s}\ge0\quad\Longleftrightarrow\quad
 \Theta_{n,t,s,z}\ge0,\qquad 1\le s<2t,
 \label{eq:S-bridge-sign-chain}
\end{equation}
because all cleared factors are positive.  Thus no sign is lost in the
reduction, and the filtered distance-space condition is equivalent to
\begin{equation}
 \frac{\coef{t}{G(x)}}{\coef{t-1}{G(x)}}
 \ge1-\frac{2+7z}{2s+1}.
 \label{eq:S-direct-target}
\end{equation}
Equivalently,
\begin{equation}
 (2s+1)\coef{t}{G(x)}-(2s-1-7z)\coef{t-1}{G(x)}\ge0.
 \label{eq:S-direct-cleared}
\end{equation}

Let
\begin{equation}
 p=\frac{1+7z}{2+7z},
 \qquad
 \rho=\frac{8z^2}{1+8z^2}.
 \label{eq:S-prho}
\end{equation}
Let $X\sim{\rm Bin}(s,p)$ and $Y\sim{\rm Bin}(N,\rho)$ be independent, and let $X_-\sim{\rm Bin}(s-1,p)$.  Equation \eqref{eq:S-saddle} is $sp+N\rho=t$.  Since $A=p/(1-p)$ and $B=\rho/(1-\rho)$, the common normalization cancels and, with
\begin{equation}
 R_G:=\frac{\Prob(X_-+Y=t)}{\Prob(X_-+Y=t-1)},
 \label{eq:S-RG-def}
\end{equation}
one has
\begin{equation}
 R_G=\frac{\coef{t}{G(x)}}{\coef{t-1}{G(x)}}.
 \label{eq:S-prob-ratio}
\end{equation}
Deleting one of the $s$ high-probability Bernoulli coordinates gives
\begin{align}
 \E[X\,\mathbf 1_{\{X+Y=t\}}]&=sp\,\Prob(X_-+Y=t-1),
 \label{eq:S-delete1}\\
 \Prob(X+Y=t)&=p\,\Prob(X_-+Y=t-1)+(1-p)\Prob(X_-+Y=t).
 \label{eq:S-delete2}
\end{align}
Thus
\begin{equation}
 \E[X\mid X+Y=t]=\frac{sp}{p+(1-p)R_G}.
 \label{eq:S-conditional-mean-ratio}
\end{equation}
Consequently
\begin{align}
 \E[X\mid X+Y=t]\le p\left(s+\frac12\right)
 &\Longleftrightarrow
 R_G\ge\frac{2s-1-7z}{2s+1} \nonumber\\
 &\Longleftrightarrow
 R_G\ge1-\frac{2+7z}{2s+1},
 \label{eq:S-mean-ratio-equivalence}
\end{align}
where the middle expression uses $p=(1+7z)/(2+7z)$.  Hence
\eqref{eq:S-direct-target} is equivalent to
\begin{equation}
 \E[X\mid X+Y=t]\le p\left(s+\frac12\right).
 \label{eq:S-mean-target}
\end{equation}
This is the bridge target used in the Stein-tangent argument.

\smsection{Stein--tangent positivity}{sec:S7}

This section proves the positivity of the bridge expression
\eqref{eq:S-theta-def} left by Sec.~\ref{sec:S6}.  The endpoint $s=2t$ is
exact.  If $s=2t$, then the saddle solution is $z=0$, so
\begin{equation}
 G(x)=(1+x)^{2t-1},\qquad
 \frac{\coef{t}{G}}{\coef{t-1}{G}}=1,
\end{equation}
and the margin in \eqref{eq:S-direct-target} is
\begin{equation}
 1-\left(1-\frac2{4t+1}\right)=\frac2{4t+1}>0.
 \label{eq:S-tail-margin}
\end{equation}
Assume henceforth $s<2t$.  In the bridge window,
\begin{equation}
 0<z<\frac15.
 \label{eq:S-z-bound}
\end{equation}
Indeed, at $z=0$ the right side of \eqref{eq:S-saddle} is $s/2<t$.  At $z=1/5$ it exceeds $t$ by
\begin{equation}
 s\frac{12}{17}+(n-1-s)\frac{8}{33}-t>\frac{15t+124}{561}>0.
\end{equation}
For the displayed lower bound, substitute $n>72t/17$ and use
\begin{equation}
 \frac{12}{17}-\frac{8}{33}=\frac{260}{561}>0,
 \qquad s\ge1.
\end{equation}
The saddle side is strictly increasing in $z$, since
\begin{equation}
 \frac{d}{dz}\frac{1+7z}{2+7z}=\frac7{(2+7z)^2}>0,
 \qquad
 \frac{d}{dz}\frac{8z^2}{1+8z^2}=\frac{16z}{(1+8z^2)^2}>0
\end{equation}
for $z>0$.

Put $S=s$, $T=t$, $U=N-t$, $R=A/B$, and
\begin{equation}
 X_*=p\left(s+\frac12\right).
\end{equation}
The conditional law of $X$ given $X+Y=t$ has unnormalized weights
\begin{equation}
 w_k=\binom S k\binom N{T-k}A^kB^{T-k}.
\end{equation}
The adjacent ratio is
\begin{equation}
 \frac{w_k}{w_{k-1}}
 =R\frac{(S-k+1)(T-k+1)}{k(U+k)}.
\end{equation}
Thus the weights satisfy the detailed balance identity
\begin{equation}
 w_{k-1}a(k-1)=w_k b(k),
 \qquad
 a(x)=R(S-x)(T-x),
 \qquad
 b(x)=x(U+x).
 \label{eq:S-balance}
\end{equation}
Therefore, for every test function $F$,
\begin{equation}
 \sum_k\{a(k)F(k+1)-b(k)F(k)\}w_k=0.
 \label{eq:S-stein}
\end{equation}

\begin{lemma}[Affine Stein tangent]
\label{lem:S-affine}
Let $F(x)=\alpha+\beta x$ and set
\begin{equation}
 \mathcal S F(x)=a(x)F(x+1)-b(x)F(x).
\end{equation}
Choose $\alpha,\beta$ so that
\begin{equation}
 \mathcal S F(X_*)=0,
 \qquad
 (\mathcal S F)'(X_*)=1.
 \label{eq:S-tangent-system}
\end{equation}
If
\begin{equation}
 \mathcal S F(x)-(x-X_*)\ge0
 \label{eq:S-Stein-majorant}
\end{equation}
on the support of $w_k$, then \eqref{eq:S-mean-target} holds.
\end{lemma}

\begin{proof}
Taking expectation in \eqref{eq:S-stein} gives $\E\mathcal S F(X)=0$.  Therefore
\begin{equation}
 0=\E\mathcal S F(X)\ge\E(X-X_*),
\end{equation}
which is precisely \eqref{eq:S-mean-target}.
\end{proof}

We now make the tangent construction and its sign orientation explicit.  All
quantities in the following display are evaluated at $X_*$.  Write
\begin{align}
 A_0&=a-b,
 &B_0&=a(X_*+1)-bX_*,\nonumber\\
 A_1&=a'-b',
 &B_1&=a'(X_*+1)+a-b'X_*-b,
 \label{eq:S-denom-def}
\end{align}
and
\begin{equation}
 \Delta=A_0B_1-B_0A_1.
 \label{eq:S-Delta-def}
\end{equation}
The tangent equations \eqref{eq:S-tangent-system} are the linear system
\begin{equation}
 \alpha A_0+\beta B_0=0,
 \qquad
 \alpha A_1+\beta B_1=1,
 \label{eq:S-tangent-linear-system}
\end{equation}
so
\begin{equation}
 \alpha=-\frac{B_0}{\Delta},
 \qquad
 \beta=\frac{A_0}{\Delta}.
 \label{eq:S-alpha-beta}
\end{equation}

The Bernstein convention used here is: if $f(y)$ has degree at most $d$, write
\begin{equation}
 f(y)=\sum_{j=0}^{d}B_j(f)\binom dj y^j(1-y)^{d-j}.
 \label{eq:S-bern-def}
\end{equation}
Nonnegative entries $B_j(f)$ imply $f(y)\ge0$ on $0\le y\le1$.  For a polynomial $F(T,y)$, the notation $\mathcal B_{m,d}(F)$ in the branch endpoint tables means: after the substitution $t=T+4$, $z=y/5$, expand in the Bernstein basis of degree $d$ in the bounded variable $y$, and list the resulting coefficient polynomials in the unbounded parameter $T$.  The index $m$ indicates the maximal ordinary degree in $T$ of these displayed polynomials.  Thus positivity is read by checking that every displayed $T$-polynomial has nonnegative ordinary coefficients.  The superscripts I and II refer to the branches $s\ge t$ and $s<t$, respectively.  To justify the affine tangent normalization and its sign orientation, the same substitution $t=T+4$, $z=y/5$ gives the denominator signs used in \eqref{eq:S-denom-signs-use}.  For the tangent-denominator tables, the Bernstein expansion is iterated over the branch parameter $v\in[0,1]$ and $y\in[0,1]$; the single index $j$ flattens the resulting coefficient grid.  Namely, for the quantities defined in \eqref{eq:S-denom-def}--\eqref{eq:S-Delta-def}, the Bernstein coefficient vectors for $-A_0$ and $\Delta$ are displayed below.  All entries have nonnegative ordinary coefficients in $T$, hence $A_0<0$ and $\Delta>0$.

For $t\ge4$ the Bernstein coefficient tables displayed below give
\begin{equation}
 -A_0>0,
 \qquad
 \Delta>0.
 \label{eq:S-denom-signs-use}
\end{equation}
Hence $\beta<0$.  Since $0<z<1/5$, we have
$R=A/B=(1+7z)/(8z^2)>1$.  The cubic leading coefficient of
$\mathcal S F(x)-(x-X_*)$ is $\beta(R-1)$.  Also
\eqref{eq:S-tangent-system} gives
\begin{equation}
 \mathcal S F(X_*)-(X_*-X_*)=0,
 \qquad
 \frac{d}{dx}\bigl(\mathcal S F(x)-(x-X_*)\bigr)\Big|_{x=X_*}=0.
\end{equation}
Thus
\begin{equation}
 \mathcal S F(x)-(x-X_*)=(x-X_*)^2L(x)
 \label{eq:S-L-factor}
\end{equation}
with $L$ affine, and the preceding leading-coefficient sign says that $L$ has negative slope.

\begin{lemma}[Endpoint reduction for the affine tangent]
\label{lem:S-endpoint-reduction}
Assume $t\ge4$ and $s<2t$ in the bridge window.  If the upper-endpoint value
of $L$ is nonnegative on each support branch $s\ge t$ and $s<t$, then
\eqref{eq:S-Stein-majorant} holds on the entire conditional support.
\end{lemma}

\begin{proof}
The conditional support is an interval of integers.  By \eqref{eq:S-L-factor},
the quadratic factor $(x-X_*)^2$ is nonnegative on the support.  The remaining
factor $L$ is affine with negative slope, hence its minimum on the support is
attained at the upper endpoint.  The upper endpoint is $M=t$ when $s\ge t$ and
$M=s$ when $s<t$.  Checking these two endpoint values is therefore sufficient.
\end{proof}

In general the support is the integer interval
\begin{equation}
 \max(0,t-N)\le k\le M:=\min(s,t).
\end{equation}
In the present $t\ge4$ bridge range its lower endpoint is $0$, because
$n>72t/17$ and $s\le2t$ imply
\begin{equation}
 N=n-1-s>\frac{72t}{17}-1-2t=\frac{38t}{17}-1>t.
\end{equation}
The cases $t\le3$ are handled separately below.  This gives two upper-endpoint branches.

If $s\ge t$, write $r=2t-s$.  Since the tail case $s=2t$ has already been removed, this branch has $1\le r\le t$.  The endpoint condition at $M=t$ is equivalent to
\begin{equation}
 \frac{P_I(t,r,z)}{D_I(t,r,z)}\le0,
 \qquad D_I(t,r,z)>0,
 \label{eq:S-PI-denom}
\end{equation}
where \(D_I\) is the product of the positive monomial factors in
\(z,1+7z,8z^2,2+7z\), the positive support factors, and the tangent
denominators \(-A_0\) and \(\Delta\).  Its positivity follows from
\eqref{eq:S-denom-signs-use} and the Bernstein table below.  Therefore the
same endpoint condition is the polynomial sign
\begin{equation}
 P_I(t,r,z)\le0,
 \label{eq:S-PI}
\end{equation}
where
\begin{align}
P_I={}&3136r^2z^4-1400r^2z^3-1440r^2z^2-280r^2z-16r^2\notag\\
&+12544rtz^6-5600rtz^5-13600rtz^4+2828rtz^3+3272rtz^2+532rtz+24rt\notag\\
&+6272rz^6-9184rz^5-1342rz^4+2772rz^3+1276rz^2+196rz+10r\notag\\
&-25088t^2z^6+224t^2z^5+5248t^2z^4-4116t^2z^3-2216t^2z^2-280t^2z-16t^2\notag\\
&-18816tz^6+26656tz^5+13502tz^4+1750tz^3+158tz^2+70tz+8t\notag\\
&-3136z^6+4592z^5-113z^4-1036z^3-278z^2-28z-1.
\end{align}
As a quadratic in $r$, its leading coefficient is
\begin{equation}
 8(z-1)(7z+1)(7z+2)(8z+1)<0.
\end{equation}
Its discriminant is $4(z-1)(8z+1)H(t,z)$.  Since $0<z<1/5$, we have $z-1<0$ and $8z+1>0$; hence the discriminant is nonpositive once $H(t,z)\geq 0$.  Together with the negative leading coefficient, this forces $P_I\le0$ for all real $r$, and hence on the branch range $1\le r\le t$.  This last sign follows from Bernstein positivity.  Put $t=T+4$ and $z=y/5$; then $T\ge0$ and $0\le y\le1$.  The Bernstein coefficients of $H(T+4,y/5)$ are displayed in the following table.
\begin{center}
\scriptsize
\setlength{\tabcolsep}{4pt}
\renewcommand{\arraystretch}{1.16}
\begin{tabular}{@{}rl@{}}
\multicolumn{2}{@{}l}{\normalsize \textit{Branch-I discriminant coefficients.}}\\[1mm]
$j$ & $B_j(H(T+4,y/5))$\\
\hline
0 & \cform{(4T+7)(28T+113)}\\
1 & \cform{\left(7392T^2+40100T+41489\right)/\left(50\right)}\\
2 & \cform{\left(221868T^2+1124336T+927821\right)/\left(1125\right)}\\
3 & \cform{\left(4017308T^2+19092656T+11751147\right)/\left(15000\right)}\\
4 & \cform{\left(2(2443206T^2+11041810T+4888745)\right)/\left(13125\right)}\\
5 & \cform{\left(104525738T^2+459346365T+158295399\right)/\left(196875\right)}\\
6 & \cform{\left(2(636059831T^2+2787108348T+940015387)\right)/\left(1640625\right)}\\
7 & \cform{\left(2704681907T^2+12071433766T+4914126799\right)/\left(2343750\right)}\\
8 & \cform{\left(16(1910194265T^2+8804282929T+4607519821)\right)/\left(17578125\right)}\\
9 & \cform{\left(8(3215690437T^2+15402854032T+10109647956)\right)/\left(9765625\right)}\\
10 & \cform{\left(64(608944097T^2+3034086628T+2387265068)\right)/\left(9765625\right)}
\end{tabular}
\end{center}
Every entry is nonnegative for $T\ge0$, so the branch-I endpoint condition holds.

If $s<t$, write $h=t-s$.  Then $h\ge1$.  The endpoint condition at $M=s$ is equivalently
\begin{equation}
 \frac{P_{II}(t,h,z)}{D_{II}(t,h,z)}\ge0,
 \qquad D_{II}(t,h,z)>0,
 \label{eq:S-PII-denom}
\end{equation}
with the same type of positive denominator: positive monomials and support
factors times the tangent denominators \(-A_0\) and \(\Delta\).  Thus its
sign is the polynomial sign
\begin{equation}
 P_{II}(t,h,z)\ge0,
 \label{eq:S-PII}
\end{equation}
where $P_{II}=a_2(z)h^2+a_1(t,z)h+a_0(t,z)$ and
\begin{align}
a_2={}&12544z^6-16576z^5-5564z^4+6020z^3+3076z^2+476z+24,\\
a_1={}&-25088tz^6+11200tz^5+9952tz^4+2268tz^3+1244tz^2+392tz+32t\notag\\
&-12544z^6+17472z^5+2556z^4-5082z^3-2094z^2-294z-14,\\
a_0={}&12544t^2z^6+5376t^2z^5+5216t^2z^4+2688t^2z^3+384t^2z^2+28t^2z+8t^2\notag\\
&+12544tz^6-17472tz^5-12160tz^4-4522tz^3-1434tz^2-266tz-18t\notag\\
&+3136z^6-4592z^5+113z^4+1036z^3+278z^2+28z+1.
\end{align}
Again put $t=T+4$ and $z=y/5$, so $T\ge0$ and $0\le y\le1$.  The Bernstein coefficients of the three branch-II terms are as follows.
\begin{center}
\scriptsize
\setlength{\tabcolsep}{4pt}
\renewcommand{\arraystretch}{1.16}
\begin{tabular}{@{}rl@{}}
\multicolumn{2}{@{}l}{\normalsize \textit{Branch-II endpoint coefficients for }$a_2$.}\\[1mm]
$j$ & $B_j(a_2)$\\
\hline
0 & \cform{24}\\
1 & \cform{\left(598\right)/\left(15\right)}\\
2 & \cform{\left(7992\right)/\left(125\right)}\\
3 & \cform{\left(12327\right)/\left(125\right)}\\
4 & \cform{\left(1366136\right)/\left(9375\right)}\\
5 & \cform{\left(642464\right)/\left(3125\right)}\\
6 & \cform{\left(4328064\right)/\left(15625\right)}
\end{tabular}
\end{center}
\begin{center}
\scriptsize
\setlength{\tabcolsep}{4pt}
\renewcommand{\arraystretch}{1.16}
\begin{tabular}{@{}rl@{}}
\multicolumn{2}{@{}l}{\normalsize \textit{Branch-II endpoint coefficients for }$a_1$.}\\[1mm]
$j$ & $B_j(a_1)$\\
\hline
0 & \cform{2(16T+57)}\\
1 & \cform{\left(676T+2347\right)/\left(15\right)}\\
2 & \cform{\left(2(11522T+38741)\right)/\left(375\right)}\\
3 & \cform{\left(102574T+332565\right)/\left(1250\right)}\\
4 & \cform{\left(4(255143T+798941)\right)/\left(9375\right)}\\
5 & \cform{\left(2(681955T+2086228)\right)/\left(9375\right)}\\
6 & \cform{\left(624(4913T+14936)\right)/\left(15625\right)}
\end{tabular}
\end{center}
\begin{center}
\scriptsize
\setlength{\tabcolsep}{4pt}
\renewcommand{\arraystretch}{1.16}
\begin{tabular}{@{}rl@{}}
\multicolumn{2}{@{}l}{\normalsize \textit{Branch-II endpoint coefficients for }$a_0$.}\\[1mm]
$j$ & $B_j(a_0)$\\
\hline
0 & \cform{8T^2+46T+57}\\
1 & \cform{\left(134T^2+669T+561\right)/\left(15\right)}\\
2 & \cform{\left(4084T^2+17838T+7361\right)/\left(375\right)}\\
3 & \cform{\left(18684T^2+77121T+17588\right)/\left(1250\right)}\\
4 & \cform{\left(4(53284T^2+227187T+81636)\right)/\left(9375\right)}\\
5 & \cform{\left(26(13243T^2+60483T+36188)\right)/\left(9375\right)}\\
6 & \cform{\left(4(239581T^2+1178444T+977824)\right)/\left(15625\right)}
\end{tabular}
\end{center}
Since $h=t-s\ge1$ in this branch, these signs give $P_{II}\ge0$ for $t\ge4$.

% Compact Bernstein coefficient tables for the Stein tangent denominators.

% Each entry has nonnegative coefficients for T >= 0.

\begin{center}
\scriptsize
\setlength{\tabcolsep}{4pt}
\renewcommand{\arraystretch}{1.16}
\begin{tabular}{@{}rl@{}}
\multicolumn{2}{@{}l}{\normalsize \textit{Denominator coefficients for }$\mathcal B_{1,4}(-A_0^{I})$.}\\[1mm]
$j$ & $B_j$\\
\hline
0 & \cform{625 \left(4 T + 15\right)}\\
1 & \cform{\left(125 \left(122 T + 447\right)\right)/\left(4\right)}\\
2 & \cform{\left(50 \left(340 T + 1209\right)\right)/\left(3\right)}\\
3 & \cform{\left(15 \left(1131 T + 3908\right)\right)/\left(2\right)}\\
4 & \cform{72 \left(187 T + 644\right)}\\
5 & \cform{625 \left(6 T + 23\right)}\\
6 & \cform{\left(125 \left(190 T + 719\right)\right)/\left(4\right)}\\
7 & \cform{\left(25 \left(1081 T + 4022\right)\right)/\left(3\right)}\\
8 & \cform{\left(5 \left(5297 T + 19340\right)\right)/\left(2\right)}
\end{tabular}
\end{center}

\begin{center}
\scriptsize
\setlength{\tabcolsep}{4pt}
\renewcommand{\arraystretch}{1.16}
\begin{tabular}{@{}rl@{}}
\multicolumn{2}{@{}l}{\normalsize \textit{Denominator coefficients for }$\mathcal B_{1,4}(-A_0^{I})$. (continued)}\\[1mm]
$j$ & $B_j$\\
\hline
9 & \cform{24 \left(821 T + 2972\right)}
\end{tabular}
\end{center}

\begin{center}
\scriptsize
\setlength{\tabcolsep}{4pt}
\renewcommand{\arraystretch}{1.16}
\begin{tabular}{@{}rl@{}}
\multicolumn{2}{@{}l}{\normalsize \textit{Denominator coefficients for }$\mathcal B_{3,8}(\Delta^{I})$.}\\[1mm]
$j$ & $B_j$\\
\hline
0 & \cform{390625 \left(4 T + 15\right)^{2}}\\
1 & \cform{\left(78125 \left(4 T + 15\right) \left(122 T + 447\right)\right)/\left(4\right)}\\
2 & \cform{\left(15625 \left(25764 T^{2} + 188300 T + 343865\right)\right)/\left(28\right)}\\
3 & \cform{\left(3125 \left(96532 T^{2} + 693259 T + 1242754\right)\right)/\left(14\right)}\\
4 & \cform{\left(250 \left(903274 T^{2} + 6351099 T + 11122728\right)\right)/\left(7\right)}\\
5 & \cform{\left(500 \left(679473 T^{2} + 4659040 T + 7923304\right)\right)/\left(7\right)}\\
6 & \cform{\left(25 \left(20667969 T^{2} + 137668192 T + 225661744\right)\right)/\left(7\right)}\\
7 & \cform{60 \left(1903473 T^{2} + 12283936 T + 19256752\right)}\\
8 & \cform{576 \left(314721 T^{2} + 1971184 T + 2946544\right)}
\end{tabular}
\end{center}

\begin{center}
\scriptsize
\setlength{\tabcolsep}{4pt}
\renewcommand{\arraystretch}{1.16}
\begin{tabular}{@{}rl@{}}
\multicolumn{2}{@{}l}{\normalsize \textit{Denominator coefficients for }$\mathcal B_{3,8}(\Delta^{I})$. (continued)}\\[1mm]
$j$ & $B_j$\\
\hline
9 & \cform{\left(390625 \left(128 T^{3} + 1536 T^{2} + 6108 T + 8051\right)\right)/\left(3\right)}\\
10 & \cform{\left(78125 \left(3232 T^{3} + 38812 T^{2} + 154094 T + 202355\right)\right)/\left(12\right)}\\
11 & \cform{\left(15625 \left(142368 T^{3} + 1712636 T^{2} + 6790232 T + 8878971\right)\right)/\left(84\right)}\\
12 & \cform{\left(3125 \left(223710 T^{3} + 2700380 T^{2} + 10698221 T + 13925589\right)\right)/\left(21\right)}\\
13 & \cform{\left(250 \left(1172636 T^{3} + 14239590 T^{2} + 56436933 T + 73133712\right)\right)/\left(7\right)}\\
14 & \cform{\left(125 \left(17744136 T^{3} + 217551722 T^{2} + 864181727 T + 1115333148\right)\right)/\left(42\right)}\\
15 & \cform{\left(25 \left(56125840 T^{3} + 698189335 T^{2} + 2786570788 T + 3584336992\right)\right)/\left(21\right)}\\
16 & \cform{\left(10 \left(25453675 T^{3} + 323331358 T^{2} + 1300619732 T + 1668590768\right)\right)/\left(3\right)}\\
17 & \cform{16 \left(6755375 T^{3} + 88381096 T^{2} + 359840864 T + 461114304\right)}
\end{tabular}
\end{center}

\begin{center}
\scriptsize
\setlength{\tabcolsep}{4pt}
\renewcommand{\arraystretch}{1.16}
\begin{tabular}{@{}rl@{}}
\multicolumn{2}{@{}l}{\normalsize \textit{Denominator coefficients for }$\mathcal B_{3,8}(\Delta^{I})$. (continued)}\\[1mm]
$j$ & $B_j$\\
\hline
18 & \cform{\left(390625 \left(256 T^{3} + 3060 T^{2} + 12144 T + 16003\right)\right)/\left(3\right)}\\
19 & \cform{\left(78125 \left(6688 T^{3} + 79904 T^{2} + 316534 T + 415827\right)\right)/\left(12\right)}\\
20 & \cform{\left(15625 \left(302528 T^{3} + 3614196 T^{2} + 14291276 T + 18708427\right)\right)/\left(84\right)}\\
21 & \cform{\left(15625 \left(193812 T^{3} + 2317088 T^{2} + 9147735 T + 11930038\right)\right)/\left(42\right)}\\
22 & \cform{\left(250 \left(7710180 T^{3} + 92365031 T^{2} + 364297333 T + 473312504\right)\right)/\left(21\right)}\\
23 & \cform{\left(125 \left(19545276 T^{3} + 235084380 T^{2} + 927309199 T + 1200688924\right)\right)/\left(21\right)}\\
24 & \cform{\left(25 \left(123556280 T^{3} + 1496234719 T^{2} + 5912395848 T + 7634459248\right)\right)/\left(21\right)}\\
25 & \cform{\left(10 \left(55724725 T^{3} + 681982942 T^{2} + 2705556536 T + 3487259840\right)\right)/\left(3\right)}\\
26 & \cform{\left(16 \left(43964125 T^{3} + 546542808 T^{2} + 2183396112 T + 2813116672\right)\right)/\left(3\right)}
\end{tabular}
\end{center}

\begin{center}
\scriptsize
\setlength{\tabcolsep}{4pt}
\renewcommand{\arraystretch}{1.16}
\begin{tabular}{@{}rl@{}}
\multicolumn{2}{@{}l}{\normalsize \textit{Denominator coefficients for }$\mathcal B_{3,8}(\Delta^{I})$. (continued)}\\[1mm]
$j$ & $B_j$\\
\hline
27 & \cform{390625 \left(2 T + 9\right) \left(48 T^{2} + 362 T + 681\right)}\\
28 & \cform{\left(78125 \left(2648 T^{3} + 31884 T^{2} + 127274 T + 168465\right)\right)/\left(4\right)}\\
29 & \cform{\left(15625 \left(125472 T^{3} + 1511068 T^{2} + 6024320 T + 7953289\right)\right)/\left(28\right)}\\
30 & \cform{\left(3125 \left(208902 T^{3} + 2517590 T^{2} + 10025682 T + 13198131\right)\right)/\left(7\right)}\\
31 & \cform{\left(250 \left(3430872 T^{3} + 41412735 T^{2} + 164790433 T + 216304496\right)\right)/\left(7\right)}\\
32 & \cform{\left(125 \left(17834916 T^{3} + 215914822 T^{2} + 859156991 T + 1124695132\right)\right)/\left(14\right)}\\
33 & \cform{\left(75 \left(19153480 T^{3} + 233024451 T^{2} + 928311084 T + 1212568000\right)\right)/\left(7\right)}\\
34 & \cform{10 \left(26280425 T^{3} + 322184922 T^{2} + 1287090420 T + 1678809584\right)}\\
35 & \cform{192 \left(1744625 T^{3} + 21631623 T^{2} + 86853012 T + 113254112\right)}
\end{tabular}
\end{center}

\begin{center}
\scriptsize
\setlength{\tabcolsep}{4pt}
\renewcommand{\arraystretch}{1.16}
\begin{tabular}{@{}rl@{}}
\multicolumn{2}{@{}l}{\normalsize \textit{Denominator coefficients for }$\mathcal B_{1,4}(-A_0^{II})$.}\\[1mm]
$j$ & $B_j$\\
\hline
0 & \cform{625 \left(6 T + 23\right)}\\
1 & \cform{\left(125 \left(190 T + 719\right)\right)/\left(4\right)}\\
2 & \cform{\left(25 \left(1081 T + 4022\right)\right)/\left(3\right)}\\
3 & \cform{\left(5 \left(5297 T + 19340\right)\right)/\left(2\right)}\\
4 & \cform{24 \left(821 T + 2972\right)}\\
5 & \cform{625 \left(8 T + 31\right)}\\
6 & \cform{\left(125 \left(272 T + 1047\right)\right)/\left(4\right)}\\
7 & \cform{\left(25 \left(1685 T + 6438\right)\right)/\left(3\right)}\\
8 & \cform{\left(5 \left(8993 T + 34124\right)\right)/\left(2\right)}
\end{tabular}
\end{center}

\begin{center}
\scriptsize
\setlength{\tabcolsep}{4pt}
\renewcommand{\arraystretch}{1.16}
\begin{tabular}{@{}rl@{}}
\multicolumn{2}{@{}l}{\normalsize \textit{Denominator coefficients for }$\mathcal B_{1,4}(-A_0^{II})$. (continued)}\\[1mm]
$j$ & $B_j$\\
\hline
9 & \cform{24 \left(1445 T + 5468\right)}
\end{tabular}
\end{center}

\begin{center}
\scriptsize
\setlength{\tabcolsep}{4pt}
\renewcommand{\arraystretch}{1.16}
\begin{tabular}{@{}rl@{}}
\multicolumn{2}{@{}l}{\normalsize \textit{Denominator coefficients for }$\mathcal B_{3,8}(\Delta^{II})$.}\\[1mm]
$j$ & $B_j$\\
\hline
0 & \cform{390625 \left(2 T + 9\right) \left(48 T^{2} + 362 T + 681\right)}\\
1 & \cform{\left(78125 \left(2648 T^{3} + 31884 T^{2} + 127274 T + 168465\right)\right)/\left(4\right)}\\
2 & \cform{\left(15625 \left(125472 T^{3} + 1511068 T^{2} + 6024320 T + 7953289\right)\right)/\left(28\right)}\\
3 & \cform{\left(3125 \left(208902 T^{3} + 2517590 T^{2} + 10025682 T + 13198131\right)\right)/\left(7\right)}\\
4 & \cform{\left(250 \left(3430872 T^{3} + 41412735 T^{2} + 164790433 T + 216304496\right)\right)/\left(7\right)}\\
5 & \cform{\left(125 \left(17834916 T^{3} + 215914822 T^{2} + 859156991 T + 1124695132\right)\right)/\left(14\right)}\\
6 & \cform{\left(75 \left(19153480 T^{3} + 233024451 T^{2} + 928311084 T + 1212568000\right)\right)/\left(7\right)}\\
7 & \cform{10 \left(26280425 T^{3} + 322184922 T^{2} + 1287090420 T + 1678809584\right)}\\
8 & \cform{192 \left(1744625 T^{3} + 21631623 T^{2} + 86853012 T + 113254112\right)}
\end{tabular}
\end{center}

\begin{center}
\scriptsize
\setlength{\tabcolsep}{4pt}
\renewcommand{\arraystretch}{1.16}
\begin{tabular}{@{}rl@{}}
\multicolumn{2}{@{}l}{\normalsize \textit{Denominator coefficients for }$\mathcal B_{3,8}(\Delta^{II})$. (continued)}\\[1mm]
$j$ & $B_j$\\
\hline
9 & \cform{\left(390625 \left(320 T^{3} + 3876 T^{2} + 15576 T + 20771\right)\right)/\left(3\right)}\\
10 & \cform{\left(78125 \left(9312 T^{3} + 112828 T^{2} + 453116 T + 603307\right)\right)/\left(12\right)}\\
11 & \cform{\left(15625 \left(466768 T^{3} + 5658404 T^{2} + 22708616 T + 30181819\right)\right)/\left(84\right)}\\
12 & \cform{\left(3125 \left(1646488 T^{3} + 19976164 T^{2} + 80119991 T + 106279262\right)\right)/\left(42\right)}\\
13 & \cform{\left(250 \left(14321896 T^{3} + 173999459 T^{2} + 697600774 T + 923525244\right)\right)/\left(21\right)}\\
14 & \cform{\left(125 \left(78761776 T^{3} + 958991990 T^{2} + 3845063765 T + 5080945972\right)\right)/\left(42\right)}\\
15 & \cform{\left(25 \left(267891572 T^{3} + 3272876251 T^{2} + 13133470604 T + 17329952448\right)\right)/\left(21\right)}\\
16 & \cform{\left(20 \left(64522565 T^{3} + 792256185 T^{2} + 3185429574 T + 4200252680\right)\right)/\left(3\right)}\\
17 & \cform{64 \left(9002350 T^{3} + 111333993 T^{2} + 449221500 T + 592568608\right)}
\end{tabular}
\end{center}

\begin{center}
\scriptsize
\setlength{\tabcolsep}{4pt}
\renewcommand{\arraystretch}{1.16}
\begin{tabular}{@{}rl@{}}
\multicolumn{2}{@{}l}{\normalsize \textit{Denominator coefficients for }$\mathcal B_{3,8}(\Delta^{II})$. (continued)}\\[1mm]
$j$ & $B_j$\\
\hline
18 & \cform{\left(390625 \left(256 T^{3} + 3168 T^{2} + 12972 T + 17587\right)\right)/\left(3\right)}\\
19 & \cform{\left(78125 \left(7808 T^{3} + 96848 T^{2} + 397018 T + 538339\right)\right)/\left(12\right)}\\
20 & \cform{\left(15625 \left(411264 T^{3} + 5114856 T^{2} + 20995376 T + 28473371\right)\right)/\left(84\right)}\\
21 & \cform{\left(3125 \left(763392 T^{3} + 9524224 T^{2} + 39156305 T + 53116069\right)\right)/\left(21\right)}\\
22 & \cform{\left(250 \left(13980036 T^{3} + 175078909 T^{2} + 721190537 T + 978734056\right)\right)/\left(21\right)}\\
23 & \cform{\left(125 \left(80811948 T^{3} + 1016721114 T^{2} + 4198438445 T + 5701989716\right)\right)/\left(42\right)}\\
24 & \cform{\left(25 \left(287953820 T^{3} + 3643385003 T^{2} + 15092466124 T + 20521778368\right)\right)/\left(21\right)}\\
25 & \cform{\left(10 \left(144565025 T^{3} + 1841900598 T^{2} + 7660722108 T + 10435018832\right)\right)/\left(3\right)}\\
26 & \cform{64 \left(10440125 T^{3} + 134155245 T^{2} + 560814588 T + 765818528\right)}
\end{tabular}
\end{center}

\begin{center}
\scriptsize
\setlength{\tabcolsep}{4pt}
\renewcommand{\arraystretch}{1.16}
\begin{tabular}{@{}rl@{}}
\multicolumn{2}{@{}l}{\normalsize \textit{Denominator coefficients for }$\mathcal B_{3,8}(\Delta^{II})$. (continued)}\\[1mm]
$j$ & $B_j$\\
\hline
27 & \cform{390625 \left(64 T^{2} + 480 T + 897\right)}\\
28 & \cform{\left(78125 \left(2176 T^{2} + 16264 T + 30281\right)\right)/\left(4\right)}\\
29 & \cform{\left(15625 \left(127904 T^{2} + 952616 T + 1766889\right)\right)/\left(28\right)}\\
30 & \cform{\left(3125 \left(530264 T^{2} + 3935183 T + 7270738\right)\right)/\left(14\right)}\\
31 & \cform{250 \left(774863 T^{2} + 5729660 T + 10545220\right)}\\
32 & \cform{\left(125 \left(35022890 T^{2} + 258047447 T + 473093244\right)\right)/\left(14\right)}\\
33 & \cform{\left(25 \left(139309849 T^{2} + 1022839748 T + 1868077888\right)\right)/\left(7\right)}\\
34 & \cform{60 \left(12994885 T^{2} + 95089670 T + 173017096\right)}\\
35 & \cform{576 \left(2088025 T^{2} + 15230300 T + 27610144\right)}
\end{tabular}
\end{center}

For the finitely many bridge triples with $t\le3$, the following exact rational
Sturm data close the same direct inequality.  Let $F_{t,n,s}(z)$ be the
saddle polynomial in \eqref{eq:S-saddle} after clearing denominators, and let
$P_{t,n,s}(z)$ be the cleared direct polynomial in
\eqref{eq:S-direct-cleared}.  In each non-tail row below, Sturm's theorem gives
exactly one zero of $F_{t,n,s}$ in the displayed interval $I$, no zero of
$P_{t,n,s}$ in $I$, and $P_{t,n,s}$ is positive at the midpoint of
$I$.  The corresponding cleared polynomials and midpoint values are displayed in
Sec.~\ref{sec:S-cert-appendix}.  Hence $P_{t,n,s}$ is positive at the saddle root.  In the tail rows
$s=2t$, the saddle root is $z=0$ and the explicit margin
\eqref{eq:S-tail-margin} applies.  Here $N_F(I)$ and $N_P(I)$ denote the
numbers of real zeros of $F_{t,n,s}$ and $P_{t,n,s}$ in the rational interval
$I$, counted by Sturm's theorem.
\begin{center}
\scriptsize
\setlength{\tabcolsep}{3.5pt}
\renewcommand{\arraystretch}{1.08}
\begin{tabular}{@{}ccccl@{} }
\hline
$t$&$n$&$s$& interval $I$& sign check\\
\hline
1&5&1&$[1/10,1/5]$&$N_F(I)=1,\ N_P(I)=0,\ P(m_I)>0$\\
1&5&2&$[0,0]$&tail case\\
2&9&1&$[1/10,1/5]$&$N_F(I)=1,\ N_P(I)=0,\ P(m_I)>0$\\
2&9&2&$[1/8,3/20]$&$N_F(I)=1,\ N_P(I)=0,\ P(m_I)>0$\\
2&9&3&$[1/20,1/10]$&$N_F(I)=1,\ N_P(I)=0,\ P(m_I)>0$\\
2&9&4&$[0,0]$&tail case\\
3&13&1&$[1/10,1/5]$&$N_F(I)=1,\ N_P(I)=0,\ P(m_I)>0$\\
3&13&2&$[3/20,1/5]$&$N_F(I)=1,\ N_P(I)=0,\ P(m_I)>0$\\
3&13&3&$[1/8,3/20]$&$N_F(I)=1,\ N_P(I)=0,\ P(m_I)>0$\\
3&13&4&$[3/40,1/10]$&$N_F(I)=1,\ N_P(I)=0,\ P(m_I)>0$\\
3&13&5&$[1/40,1/20]$&$N_F(I)=1,\ N_P(I)=0,\ P(m_I)>0$\\
3&13&6&$[0,0]$&tail case\\
3&14&1&$[1/10,1/5]$&$N_F(I)=1,\ N_P(I)=0,\ P(m_I)>0$\\
3&14&2&$[1/8,3/20]$&$N_F(I)=1,\ N_P(I)=0,\ P(m_I)>0$\\
3&14&3&$[9/80,1/8]$&$N_F(I)=1,\ N_P(I)=0,\ P(m_I)>0$\\
3&14&4&$[3/40,1/10]$&$N_F(I)=1,\ N_P(I)=0,\ P(m_I)>0$\\
3&14&5&$[1/40,1/20]$&$N_F(I)=1,\ N_P(I)=0,\ P(m_I)>0$\\
3&14&6&$[0,0]$&tail case\\
\hline
\end{tabular}
\end{center}

\begin{theorem}[Qutrit bridge-ratio estimate]
\label{thm:S-qutrit-bridge}
For every integer triple $(t,n,s)$ in the bridge window \eqref{eq:S-bridge}, with $1\le s\le2t$ and $z$ defined by \eqref{eq:S-saddle}, the direct bridge inequality \eqref{eq:S-direct-target} holds.
\end{theorem}

\begin{proof}
The case $s=2t$ is \eqref{eq:S-tail-margin}.  If $s<2t$ and $t\ge4$, then $0<z<1/5$ and Lemma~\ref{lem:S-affine}, together with the two branch endpoint inequalities, proves \eqref{eq:S-mean-target} and hence \eqref{eq:S-direct-target}.  The remaining bridge triples with $t\le3$ reduce to $(t,n)=(1,5),(2,9),(3,13),(3,14)$ with $1\le s\le2t$.  Substitution into \eqref{eq:S-direct-cleared} and \eqref{eq:S-saddle} gives univariate polynomial checks of degree at most six.  In each case the saddle equation has a unique root in $0\le z\le1/5$; exact Sturm isolation gives a rational interval for that root, and the direct polynomial is positive on the same isolating interval.
\end{proof}

\smsection{Assembly}{sec:S8}

We now assemble the proof of the nonbinary theorem stated in the Letter.  At
this point every required sign condition has been proved in the relevant length
range; the only remaining step is to insert those signs into the Li--Xing
normalization of Sec.~\ref{sec:S1}.  The case $t=0$ is immediate because
$\Vol_0^{(q^2)}(n)=1$ and every subspace has $K\le q^n$.  Hence assume
$t\ge1$.

First let $q\ge4$, so that $Q=q^2\ge16$.  For a nontrivial exact code
($K>1$), the quantum Singleton bound gives $n\ge4t+1$.  Theorem~\ref{thm:S-halfgap}
therefore applies, after the length reduction of Sec.~\ref{sec:S2} and the
critical high-alphabet comparison of Secs.~\ref{sec:Sjacobi}--\ref{sec:S3}.  It
gives
\begin{equation}
 \Lloyd_t^{(Q,n)}(s)>0,
 \qquad
 R_{Q;n,t}(s)\le1,
 \qquad 1\le s\le2t.
\end{equation}
The Li--Xing tail-pruning step in Sec.~\ref{sec:S1} removes all shells
$s>2t$; for the raw Lloyd square this is also reflected by
$c_t^{(Q)}(n,s)=0$.  Thus the checked defects are nonnegative on all required shells.  The
raw-Lloyd normalization \eqref{eq:S-lloyd-normalization} and the Li--Xing comparison
of Sec.~\ref{sec:S1} give
\begin{equation}
 K\Vol_t^{(Q)}(n)\le q^n.
\end{equation}

It remains to assemble the qutrit case $q=3$ ($Q=9$).  The three alternatives
\begin{equation}
 17n\le72t,\qquad 84(n-1)\ge373t,\qquad
 \frac{72}{17}t<n<1+\frac{373}{84}t
\end{equation}
cover every integer length.  In the short range, the quantum Singleton bound
and \eqref{eq:S-qutrit-vol} give
\begin{equation}
 K\Vol_t^{(9)}(n)\le 3^{n-4t}\,3^{4t}=3^n.
\end{equation}
In the long range, \eqref{eq:S-qutrit-natural-zero} proves positivity of the
qutrit Lloyd response and \eqref{eq:S-qutrit-chain}--\eqref{eq:S-qutrit-R2}
prove $R_{9;n,t}(s)\le1$ for every $1\le s\le2t$.  Hence the checked defects are nonnegative for the raw Lloyd square, and Sec.~\ref{sec:S1} gives
$K\Vol_t^{(9)}(n)\le3^n$.

Finally consider the bridge window
\begin{equation}
 \frac{72}{17}t<n<1+\frac{373}{84}t.
\end{equation}
If $t=1$, the bridge window contains only $n=5$.  The raw Lloyd square already
gives
\begin{equation}
 R_{9;5,1}(1)=\frac{41\cdot9}{32^2}=\frac{369}{1024}<1,
 \qquad
 R_{9;5,1}(2)=\frac{41\cdot2}{23^2}=\frac{82}{529}<1,
\end{equation}
and $L_1^{(9,5)}(1)=32$, $L_1^{(9,5)}(2)=23$ are positive.  Hence Sec.~\ref{sec:S1}
gives $K\Vol_1^{(9)}(5)\le3^5$.  We may therefore assume $t\ge2$ in the
filtered bridge.

Use the filtered Lloyd square
\begin{equation}
 f_i=h_{n,t}(i)\Lloyd_t^{(9,n)}(i)^2
\end{equation}
from \eqref{eq:S-filter}.  The bridge verification has four pieces, all already
proved above.  First, the filter is nonnegative on Fourier shells, and
Sec.~\ref{sec:S5} gives the exact Hamming prefactor
\begin{equation}
 \frac{f(0)}{f_0}=\frac{9^n}{\Vol_t^{(9)}(n)}.
\end{equation}
Second, \eqref{eq:S-filter-tail-2}--\eqref{eq:S-filter-tail-bridge-bound} give
the nonoverlapping-shell Li--Xing sign for $s>2t$.  Third, for $1\le s<2t$,
Sec.~\ref{sec:S6} gives the sign-preserving exact certificate
\eqref{eq:S-bridge-sign-chain}: the filtered shell defect is a positive prefactor
times the bridge quantity \eqref{eq:S-theta-def}, with the quotient-remainder and denominator ledgers given in Sec.~\ref{sec:S-cert-appendix}.  Fourth, Sec.~\ref{sec:S7}
proves this bridge quantity nonnegative; the endpoint $s=2t$ is the direct
calculation \eqref{eq:S-tail-margin}, and the remaining finitely many small
bridge triples are covered by the small-bridge table in Sec.~\ref{sec:S7}.
Hence all overlapping-shell defects and nonoverlapping-shell signs required by
the division-free Li--Xing comparison of Sec.~\ref{sec:S1} hold.  With the exact prefactor above, this gives
\begin{equation}
 K\Vol_t^{(9)}(n)\le3^n.
\end{equation}

These high-alphabet, qutrit short-range, qutrit long-range, and qutrit bridge
arguments cover all nonbinary local dimensions $q\ge3$ and prove the nonbinary
quantum Hamming bound for nontrivial exact subspace codes.  The binary
$q=2$ endpoint is not used in the nonbinary proof; it is the separate $Q=4$
finite-length result cited in the Letter.

\smsection{Exact coefficient and Sturm data}{sec:S-cert-appendix}

This final appendix contains the finite exact-algebra data invoked in four
places: the high-alphabet endpoint and scalar checks of Sec.~\ref{sec:S3}, the
filtered-defect factorization of Sec.~\ref{sec:S6}, the qutrit long-range scalar
comparison of Sec.~\ref{sec:S4}, and the small-radius bridge Sturm checks of
Sec.~\ref{sec:S7}.  The symbols in each block are the quantities already defined
in the corresponding section; the block header repeats the substitutions used
there.  The displayed data are exact algebraic outputs after those
substitutions, and each displayed entry is read by integer arithmetic,
coefficientwise positivity, Bernstein coefficient nonnegativity, or Sturm
isolation on explicit rational intervals.  No numerical approximation is used in
reading the signs.  Thus the entry point is contained in the printed
certificate: start from the named formulae in the indicated section, make the
substitutions in the block header, clear only the denominators listed in the
ledger, and read the printed coefficients by the stated sign rule.

\noindent\textbf{Index of printed data.}
The high-alphabet entries correspond to the endpoint formulae and scalar
Jacobi inequality in Sec.~\ref{sec:S3}; their signs are read from rational
factorization and coefficient positivity.  The filtered bridge factorization
corresponds to \eqref{eq:S-filter-defect-def},
\eqref{eq:S-two-var-intersection}, and
\eqref{eq:S-eliminate-Ctplus}--\eqref{eq:S-eliminate-Ctminus}; its sign
information is the quotient-remainder identity modulo the saddle residual,
together with the denominator ledger.  The qutrit long-range entries correspond
to the scalar comparisons after \eqref{eq:S-qutrit-chain}--
\eqref{eq:S-qutrit-R2}; their signs are read coefficientwise in
\(\mathbb Q(\sqrt2)\) after the displayed substitutions.  The small bridge
entries correspond to \eqref{eq:S-saddle} and \eqref{eq:S-direct-cleared};
their signs are read by Sturm isolation on the printed rational intervals and
midpoint signs.

\noindent\textbf{Sign conventions.}
In the algebraic coefficient blocks, `r2' denotes \(\sqrt2\).  A coefficient of
the form \(c(a-b\sqrt2)\) is positive because the exact integer comparison
\(a^2>2b^2\) holds for that entry; coefficients of the form \(a+b\sqrt2\) with
\(a,b>0\) are positive.  In the bridge-factorization block, \(\Phi\) is the
filtered shell defect of Sec.~\ref{sec:S6} and \(Sres\) is the saddle residual
\(\mathcal S\).  The displayed quotient-remainder identity is obtained by the
four algebraic operations listed in Sec.~\ref{sec:S6}: expand the adjacency
formula, substitute the two-variable intersection generator, collect the four
adjacent coefficients of \(G\), and eliminate the outer two coefficients.  It
states that, after setting \(Sres=0\), the only remaining sign-bearing factor is
the two-coefficient bridge expression used in Sec.~\ref{sec:S6}.  The
denominator ledger lists every factor cleared in obtaining this identity, so
the positive prefactor in Sec.~\ref{sec:S6} contains no hidden sign-dependent
term.

\noindent\textbf{Bridge-factorization ledger.}
For the bridge factorization, the adjacent-coefficient eliminations
\eqref{eq:S-eliminate-Ctplus}--\eqref{eq:S-eliminate-Ctminus}, the saddle
substitution \eqref{eq:S-bridge-N-explicit}, and the remainder ledger
\eqref{eq:S-filter-remainder-ledger}--\eqref{eq:S-filter-coefficient-ledger}
are identities in the displayed variables.  The small-radius rows at the end of
this appendix give the corresponding exact Sturm output for the finite
exceptional bridge triples.

{\scriptsize
\begin{verbatim}
HIGH-ALPHABET ALGEBRAIC DATA
endpoint s=1 gap = (Q^2 - 16*Q + 16)/(2*(3*Q - 4)^2)
endpoint s=2 gap = (7*Q - 8)*(7*Q^3 - 72*Q^2 + 128*Q - 64)/(2*(3*Q - 4)^4)
Jacobi scalar numerator = 15201000*z^4 + 1147275*z^3 + 22440*z^2 - 575*z + 4
quadratic discriminant = -28415
terminal r=1 gap numerator = 28*t^2 + 220*t + 495

FILTERED DEFECT FACTORIZATION DATA
Variables: A=1+7z, B=8z^2, N=n-1-s, Sres=t-s*A/(1+A)-N*B/(1+B).
This block is only for the non-tail bridge case s<2t, z>0.  The endpoint
s=2t is checked separately in the text and never divides by B.

Denominator and sign ledger.
(1) Two-variable intersection terms are first written with binomial factors
    binom(s,a) binom(N,m-a), with 0<=a<=s and 0<=m-a<=N.  All such factors are
    nonnegative integers; in the support terms used for C_{t-1}^G at least one
    term is strictly positive.
(2) The adjacent-coefficient eliminations clear only t+1, t, A, B, and
    s+N-t+1.  In the bridge range these are positive: t>=1, A=1+7z>0,
    B=8z^2>0, and s+N-t+1=n-t>0.
(3) The saddle substitution clears the positive factors (2+7z), (1+8z^2), and
    their powers.  The residual factor
       t(2+7z)-s(1+7z)=8z^2(2+7z)N/(1+8z^2)
    is positive for z>0 and N>0.
(4) The global denominator D_+ is the product of the cleared factors in (1)--(3)
    and the positive powers displayed in the proof.  No factor whose sign depends
    on z,s,t,n is hidden in C_{n,t,s}.

After the T/T^2 expansion, two-variable intersection substitution, and adjacent-
coefficient eliminations, the exact quotient-remainder identity is
D_+ Phi / M = ((2s+1)+Sres*R_t) C_t^G
              + (-(2s-1-7z)+Sres*R_{t-1}) C_{t-1}^G.
Remainder modulo Sres:
Rem_{Sres}(D_+ Phi / M) = (2s+1) C_t^G - (2s-1-7z) C_{t-1}^G.
The same exact simplification gives the divisibility identity:
D_+ Phi - M*((2s+1) C_t^G - (2s-1-7z) C_{t-1}^G)
is divisible by Sres.
The positive factor used in the proof is
M = C^+_{n,t,s} C_{t-1}^G (1+7z)^(s-1) (8z^2)^(t-1) (2+7z)^s
    *(1+8z^2)^(N+1)*(t(2+7z)-s(1+7z)) / D_+,
where C^+_{n,t,s}>0 is precisely the product of the positive integer and rational
normalizers listed in (1)--(4).

QUTRIT LONG-RANGE SCALAR COEFFICIENT DATA
Variables A,B are nonnegative integers after s=2(A+1) or 2(A+1)+1
and t=A+B+2; r2 denotes sqrt(2).

[even rational residual numerator]
N_even_1: terms=28, total_degree=6
A^6 B^0: -336200*(-39979 + 22554*r2)
A^5 B^1: -2460*(-35817651 + 9160864*r2)
A^5 B^0: -2460*(-81240359 + 31894582*r2)
A^4 B^2: 12*(9037614379*r2 + 25404327941)
A^4 B^1: 36*(4173705749*r2 + 34857014947)
A^4 B^0: -12*(-111539524531 + 10400588668*r2)
A^3 B^3: 2*(403732016693 + 327434456532*r2)
A^3 B^2: 6*(492547791278*r2 + 729479094677)
A^3 B^1: 6*(668604292760*r2 + 1368660116403)
A^3 B^0: 2*(727470411546*r2 + 2680812514471)
A^2 B^4: 6*(252157071747 + 214884571564*r2)
A^2 B^3: 6*(1702501076659 + 1439641092442*r2)
A^2 B^2: 9*(2907233063149 + 2333583033198*r2)
A^2 B^1: 24*(1268758979973 + 903011151704*r2)
A^2 B^0: 3*(2601525082306*r2 + 4577159115505)
A^1 B^5: 6*(266102691775 + 188920298384*r2)
A^1 B^4: 18*(738736078971 + 550264007570*r2)
A^1 B^3: 6*(7352504130023 + 5672406040843*r2)
A^1 B^2: 6*(12205571476838 + 9542180314933*r2)
A^1 B^1: 18*(3403263341668 + 2603273237787*r2)
A^1 B^0: 6*(3474485005243 + 2462927925701*r2)
A^0 B^6: 62613138466*(6*r2 + 11)
A^0 B^5: 6*(671754869144*r2 + 1154900668361)
A^0 B^4: 12*(1485310075195*r2 + 2399856769221)
A^0 B^3: 2*(20755134825759*r2 + 31684675862593)
A^0 B^2: 3*(17855352994772*r2 + 26017348611749)
A^0 B^1: 6*(6031328799979*r2 + 8535990786165)
A^0 B^0: 14067440825945 + 9947822141892*r2

[even squared residual numerator]
N_even_2: terms=91, total_degree=12
A^12 B^0: -113030440000*(-2615686273 + 1803372732*r2)
A^11 B^1: -413526000*(-6635926244061 + 4386086622028*r2)
A^11 B^0: -413526000*(-18001634222765 + 12119426894644*r2)
A^10 B^2: -4034400*(-2505926412997411 + 1416700464096403*r2)
A^10 B^1: -6051600*(-9946899043778597 + 5999220013133906*r2)
A^10 B^0: -2017200*(-41801507425264453 + 26500854913328248*r2)
A^9 B^3: -45920*(-429078489051679775 + 63316504165065198*r2)
A^9 B^2: -19680*(-10215357731190363068 + 3312612465235573945*r2)
A^9 B^1: -9840*(-61898580762905094285 + 27785886655172288432*r2)
A^9 B^0: -3280*(-176504974133128700249 + 94392327861986516706*r2)
A^8 B^4: 144*(283184129973136863372 + 268070506187576311277*r2)
A^8 B^3: 144*(1804386923022846108101*r2 + 3637564946158481643308)
A^8 B^2: 432*(816738941537943395583*r2 + 5209623230823612514447)
A^8 B^1: -144*(-28910689600452987654009 + 3190182780265620553721*r2)
A^8 B^0: -144*(-19767817888234617014077 + 6077591643050223960638*r2)
A^7 B^5: 36*(5318687380888712693759 + 5269220670172499203252*r2)
A^7 B^4: 108*(20995636080754563346333 + 19087526252588566101144*r2)
A^7 B^3: 144*(69308384539839235112485 + 54278783874546921769061*r2)
A^7 B^2: 288*(44745599998766725524595*r2 + 76073066184264006193541)
A^7 B^1: 108*(77687747520173289978208*r2 + 230393822415429443454247)
A^7 B^0: 36*(24153003049201748040712*r2 + 328756510176193657172585)
A^6 B^6: 168*(4730851408106400198571 + 3602655985530256539726*r2)
A^6 B^5: 252*(40220340975645197222191 + 31455791355289870896676*r2)
A^6 B^4: 252*(198486173956659547228659 + 157468200602359284009190*r2)
A^6 B^3: 2184*(58143152444248956746734 + 45529229845093554007659*r2)
A^6 B^2: 504*(357087888862194175114294 + 261540258328853939851417*r2)
A^6 B^1: 252*(342026663040070671624866*r2 + 550294982181359537853561)
A^6 B^0: 420*(49045900529624544349980*r2 + 110696700949524197995789)
A^5 B^7: 36*(41304067773912214936700*r2 + 59915845612400941823493)
A^5 B^6: 252*(86288453816870842477256*r2 + 122680078248399861596897)
A^5 B^5: 5292*(33813535684517847735653 + 24271622652181115203698*r2)
A^5 B^4: 252*(2194778043487717044065367 + 1605871818655582566161780*r2)
A^5 B^3: 252*(3965082426396348066213557 + 2938185527141569188691136*r2)
A^5 B^2: 756*(1412578269456631262317081 + 1042154254853162670291228*r2)
A^5 B^1: 252*(2515149185994377936851959 + 1782511777299054569842106*r2)
A^5 B^0: 36*(2898482771366577834339320*r2 + 4552750831971815773753091)
A^4 B^8: 144*(18738129765611062855711*r2 + 27210291317276812110110)
A^4 B^7: 108*(399978747411358034340500*r2 + 578862358383910834764147)
A^4 B^6: 1008*(287776444303737345137213*r2 + 414273945424575496749709)
A^4 B^5: 252*(4286773297636158988027828*r2 + 6123040755957939910892771)
A^4 B^4: 189*(18385980204927718523016109 + 13002017704932415673263108*r2)
A^4 B^3: 504*(9744192878565242682461924 + 6964185235913188544595451*r2)
A^4 B^2: 126*(33934856477421201148319089 + 24428099932625234845578872*r2)
A^4 B^1: 216*(9767921750343846553408480 + 7003857234144878033623041*r2)
A^4 B^0: 9*(35271865225359810908404508*r2 + 50625080430393222336197065)
A^3 B^9: 4*(850077717065833117059036*r2 + 1203465918545112742854793)
A^3 B^8: 36*(1647310844531930025954256*r2 + 2341930959816771927076105)
A^3 B^7: 180*(2476860307327956422725724*r2 + 3532165091857233082707447)
A^3 B^6: 84*(22742081329621384439367330*r2 + 32483554926118463127603317)
A^3 B^5: 102564*(50373187994659744757267*r2 + 71928372834323288322740)
A^3 B^4: 252*(36413231530254015350682343*r2 + 51867921508779812592600477)
A^3 B^3: 84*(127692376944846481721056062*r2 + 181100821242491878210101061)
A^3 B^2: 36*(312243865134231350811104569 + 221273370182405148522290620*r2)
A^3 B^1: 36*(133284446064609192960923595 + 94725528303978580897529911*r2)
A^3 B^0: 4*(226245785222524119216677606 + 159999008135360002203591657*r2)
A^2 B^10: 168*(23057736451867509447717 + 16551450378593099321806*r2)
A^2 B^9: 12*(6138113952830822346166829 + 4388967812841374397875372*r2)
A^2 B^8: 216*(2852968378524820019141300 + 2032323028637545968301917*r2)
A^2 B^7: 36*(83327921911385242755257661 + 59146690859202955056728284*r2)
A^2 B^6: 504*(18721350759914030380125575 + 13246441917375759387545141*r2)
A^2 B^5: 756*(18744463280405535801081897*r2 + 26555841657908638629948418)
A^2 B^4: 126*(163948199667905842988277202*r2 + 232571707724360103168472815)
A^2 B^3: 252*(81142995511402776611475272*r2 + 115100151019495950553076723)
A^2 B^2: 108*(121899385697637265658665206*r2 + 172687964709661790445222373)
A^2 B^1: 12*(415002448173944870935273993*r2 + 586903150520444881939845771)
A^2 B^0: 6*(198012696826851508708180955 + 140019027247199972445704138*r2)
A^1 B^11: 4476*(414043701102967682993 + 294634297320734032156*r2)
A^1 B^10: 36*(1054462964505273052260557 + 751075425175256004605800*r2)
A^1 B^9: 24*(14494359680007010702412123 + 10328178005163747073440835*r2)
A^1 B^8: 72*(26210174848227573757351841 + 18671171111134810950746857*r2)
A^1 B^7: 1944*(3469938000017400086364963 + 2469551293213029260261429*r2)
A^1 B^6: 1008*(16569937927130274499943621 + 11775960130165638262412056*r2)
A^1 B^5: 252*(116104456726140623339522084 + 82375361562520439099380999*r2)
A^1 B^4: 108*(335949230116914806337481993 + 237972381092352635313841007*r2)
A^1 B^3: 36*(867470941568891892107761903 + 613739842150216284989259740*r2)
A^1 B^2: 12*(1047400401244924811446208762*r2 + 1481273662248857626323478567)
A^1 B^1: 36*(118329259667066012560245335*r2 + 167344437957716894171174182)
A^1 B^0: 12*(54308276342232245748490153*r2 + 76803589750908621736852907)
A^0 B^12: 2076877093820241107152*(132*r2 + 193)
A^0 B^11: 4476*(1354825608341835295096*r2 + 1965311355840683788453)
A^0 B^10: 12*(5061069074492189858136640*r2 + 7290841102118956281894627)
A^0 B^9: 8*(45573952609780065736057551*r2 + 65271709159639542035300386)
A^0 B^8: 72*(20314173734750236349045488*r2 + 28959810119672418310521595)
A^0 B^7: 72*(57417045071484985839257155*r2 + 81571616845119431753252298)
A^0 B^6: 336*(25140188502235560623747247*r2 + 35632642394215478396335784)
A^0 B^5: 36*(349431516265006389666180529*r2 + 494580376820935863227305678)
A^0 B^4: 45*(301283937015307473542869184*r2 + 426153076047830183051428677)
A^0 B^3: 8*(1823952030243027936580670245 + 1289747781988958198692311711*r2)
A^0 B^2: 6*(1241065219960218225993676735 + 877569490820033260377941212*r2)
A^0 B^1: 12*(190720982185184785396659333 + 134860166615347322394061895*r2)
A^0 B^0: 320452477350252257025435409 + 226594128868898674598496840*r2

[odd rational residual numerator]
N_odd_1: terms=35, total_degree=7
A^7 B^0: -5379200*(-39979 + 22554*r2)
A^6 B^1: -39360*(-35817651 + 9160864*r2)
A^6 B^0: -6560*(-519681941 + 250777020*r2)
A^5 B^2: 192*(9037614379*r2 + 25404327941)
A^5 B^1: -96*(-211307994455 + 12525212624*r2)
A^5 B^0: -48*(-491895442388 + 178524097707*r2)
A^4 B^3: 32*(403732016693 + 327434456532*r2)
A^4 B^2: 48*(738307424936*r2 + 1359151693981)
A^4 B^1: 24*(795845840236*r2 + 5270992372577)
A^4 B^0: -4*(-23301134988977 + 4843292117328*r2)
A^3 B^4: 96*(252157071747 + 214884571564*r2)
A^3 B^3: 16*(9245211296417 + 7723594531896*r2)
A^3 B^2: 72*(3362630580436*r2 + 5009919089375)
A^3 B^1: 12*(12659536451848*r2 + 36493747227745)
A^3 B^0: -6640*(-34296848539 + 976500438*r2)
A^2 B^5: 96*(266102691775 + 188920298384*r2)
A^2 B^4: 48*(4216468808089 + 3334489934180*r2)
A^2 B^3: 24*(26401349809135 + 21644617706808*r2)
A^2 B^2: 12*(84815014631593 + 62784667911020*r2)
A^2 B^1: 24*(18589371776624*r2 + 36816663102991)
A^2 B^0: 48*(1126009301997*r2 + 7197836045785)
A^1 B^6: 1001810215456*(6*r2 + 11)
A^1 B^5: 48*(1691167789508*r2 + 2618991918007)
A^1 B^4: 24*(22639375152467 + 16534575310318*r2)
A^1 B^3: 4*(297225577081805 + 232826352553812*r2)
A^1 B^2: 12*(120570170385899 + 91991696765848*r2)
A^1 B^1: 24*(24993670500146*r2 + 40705379835703)
A^1 B^0: 4*(24521570609040*r2 + 75314777715833)
A^0 B^6: 1518192430016*(6*r2 + 11)
A^0 B^5: 2016*(41659231488*r2 + 67836380219)
A^0 B^4: 48*(6545418635982*r2 + 9564582702265)
A^0 B^3: 8*(101807028998177 + 75539499390132*r2)
A^0 B^2: 216*(3792735551353 + 2867374806432*r2)
A^0 B^1: 48*(6446381663490*r2 + 9533017937939)
A^0 B^0: 8*(6702713012472*r2 + 14500604267753)

[odd squared residual numerator]
N_odd_2: terms=117, total_degree=14
A^14 B^0: -28935792640000*(-2615686273 + 1803372732*r2)
A^13 B^1: -105862656000*(-6635926244061 + 4386086622028*r2)
A^13 B^0: -17643776000*(-126119249810087 + 86056261995540*r2)
A^12 B^2: -1032806400*(-2505926412997411 + 1416700464096403*r2)
A^12 B^1: -258201600*(-71936142838463453 + 45800486956495284*r2)
A^12 B^0: -43033600*(-702187862215596541 + 471116048100314106*r2)
A^11 B^3: -11755520*(-429078489051679775 + 63316504165065198*r2)
A^11 B^2: -17633280*(-3520618489334445563 + 1636416997455429602*r2)
A^11 B^1: -1889280*(-120003957673216082327 + 71329721839997843120*r2)
A^11 B^0: -104960*(-2397371751216848747203 + 1563106155143226931152*r2)
A^10 B^4: 36864*(283184129973136863372 + 268070506187576311277*r2)
A^10 B^3: 4096*(6057712801233149916273*r2 + 31650533554986978039481)
A^10 B^2: -6144*(-115743405609284040143152 + 34443903338711688220417*r2)
A^10 B^1: -1536*(-1111565739474662148268557 + 580337540809741069767226*r2)
A^10 B^0: -256*(-5625672708746275543885385 + 3489952591986712064206491*r2)
A^9 B^5: 9216*(5318687380888712693759 + 5269220670172499203252*r2)
A^9 B^4: 4608*(87523302912015751353203 + 82366940814920126855628*r2)
A^9 B^3: 512*(1725611525591474026572204*r2 + 3486130281591525935991023)
A^9 B^2: -2304*(-2311136821414819417854663 + 141610547631809884223308*r2)
A^9 B^1: -192*(-46801104862637357390039153 + 18972064627410441694291908*r2)
A^9 B^0: -32*(-188376899087719384528351903 + 107029417933531807905025524*r2)
A^8 B^6: 43008*(4730851408106400198571 + 3602655985530256539726*r2)
A^8 B^5: 4608*(387420893104201542019327 + 327365560843862794312700*r2)
A^8 B^4: 6912*(999829850693008472608227 + 874652817216210809706200*r2)
A^8 B^3: 768*(14657284616287077435038916*r2 + 21771486349978884647389085)
A^8 B^2: 2304*(2635886859033713070626027*r2 + 12956041042213558107531994)
A^8 B^1: -864*(-41252245309948053208021817 + 9702534643533620795528252*r2)
A^8 B^0: -48*(-400161674462061024333110123 + 194226036112752253289955072*r2)
A^7 B^7: 9216*(41304067773912214936700*r2 + 59915845612400941823493)
A^7 B^6: 10752*(536561930982924026250331 + 386843760152336087760132*r2)
A^7 B^5: 18432*(1419230270115310700305357 + 1096872056060669066636981*r2)
A^7 B^4: 145152*(462083142730117742959241 + 376211932853086724256228*r2)
A^7 B^3: 192*(577609167996352631151905639 + 429135494147341203148211604*r2)
A^7 B^2: 288*(197436515271575927102478676*r2 + 458941201531479003252827099)
A^7 B^1: -288*(-389022158153812069961138271 + 8326887478730142839738512*r2)
A^7 B^0: -384*(-124913213694553264554117841 + 45290437550390254954803738*r2)
A^6 B^8: 36864*(18738129765611062855711*r2 + 27210291317276812110110)
A^6 B^7: 4608*(1837784295768138806349540*r2 + 2666346111366780771184547)
A^6 B^6: 5376*(8777291232880139559633480*r2 + 12463599326633916998030207)
A^6 B^5: 16128*(12976987368690503468799125 + 9544543524913295703859828*r2)
A^6 B^4: 24192*(16859482156961346200262691 + 12992887113296071718020078*r2)
A^6 B^3: 672*(775810771673375880147698995 + 586818715781554148397721812*r2)
A^6 B^2: 1008*(266086073676538909306714768*r2 + 457962068320846738623309449)
A^6 B^1: 576*(100142955206814639977714244*r2 + 496930371156084804027810167)
A^6 B^0: -384*(-249603445521418361990736103 + 49352690680174774877232846*r2)
A^5 B^9: 1024*(850077717065833117059036*r2 + 1203465918545112742854793)
A^5 B^8: 4608*(2637319857151799481919316*r2 + 3781499249266126209735289)
A^5 B^7: 13824*(5621320789127774297405076*r2 + 8106481837443316170770723)
A^5 B^6: 5376*(55130139832313285070290844*r2 + 78893838995583204492872051)
A^5 B^5: 4032*(254460491893466177100027431 + 182311265526451900559985076*r2)
A^5 B^4: 6048*(270061732787986562777809365 + 200436213968294497823999572*r2)
A^5 B^3: 2688*(644073803367948345010836773 + 482362052441396345748404418*r2)
A^5 B^2: 288*(2845130893090348639831799048*r2 + 4294496246822568509320663207)
A^5 B^1: 3456*(67184463534832628837931254*r2 + 171245362372992789041563225)
A^5 B^0: -32*(-4833430828223802709652707033 + 17510301070184511747338040*r2)
A^4 B^10: 43008*(23057736451867509447717 + 16551450378593099321806*r2)
A^4 B^9: 3584*(4517536493035410818270027 + 3215295630968095443242076*r2)
A^4 B^8: 11520*(7430773520793837756760832*r2 + 10551497160311567679191395)
A^4 B^7: 2304*(166050741946986788013197588*r2 + 237674341504218425283675783)
A^4 B^6: 5376*(210183217381463559394626621*r2 + 300827150053047619549482710)
A^4 B^5: 2016*(1602570645721209449260692187 + 1133895450034835949929946812*r2)
A^4 B^4: 3024*(1451754744906827199798399879 + 1052061100889083243444855168*r2)
A^4 B^3: 672*(5990471308974055920688699043 + 4413770753091279169581979752*r2)
A^4 B^2: 8064*(212784158444989452719545862*r2 + 304262566963716193390353229)
A^4 B^1: 96*(5291292660616931104211632280*r2 + 10001040658107021147705487497)
A^4 B^0: 64*(600823682950666371552401532*r2 + 3119626571682931840636739711)
A^3 B^11: 1145856*(414043701102967682993 + 294634297320734032156*r2)
A^3 B^10: 1536*(5989997892519431737311779 + 4284868689515774881841556*r2)
A^3 B^9: 1024*(79647995636367892229408701 + 56824284346777924940301342*r2)
A^3 B^8: 2304*(189536784197091744565575409 + 134285447113226411173482764*r2)
A^3 B^7: 576*(1899071763874229198662998420*r2 + 2700513814159638078896284231)
A^3 B^6: 672*(3991962521108123064483496188*r2 + 5696527738622189070037664761)
A^3 B^5: 2016*(2298741136590209047319434256*r2 + 3264366402016706199956832871)
A^3 B^4: 864*(9099762053649461883349646357 + 6502904794894414806428103748*r2)
A^3 B^3: 768*(8347015086075617016060769519 + 6059875522823455153176919905*r2)
A^3 B^2: 96*(36003572904163194253431856961 + 25661865083616065680741872016*r2)
A^3 B^1: 768*(928585091523801035406490599*r2 + 1511660385270349647676290647)
A^3 B^0: 128*(563467479942100164381996027*r2 + 1554176615884732648328573101)
A^2 B^12: 531680536017981723430912*(132*r2 + 193)
A^2 B^11: 572928*(3285051879005741449196*r2 + 4677599674035926138275)
A^2 B^10: 2304*(12945768591179205538458017 + 9196741373648604931622752*r2)
A^2 B^9: 256*(765356382636574858592379209 + 545184793426701451642902936*r2)
A^2 B^8: 1152*(739654052061166082372950811 + 525360640821253263702962896*r2)
A^2 B^7: 864*(2105277762266194604445765972*r2 + 2980166446088455938081022603)
A^2 B^6: 336*(11543638128722977142073318144*r2 + 16412954643674393832751039625)
A^2 B^5: 1440*(4105231672438225358475946732*r2 + 5833811134277476244774731883)
A^2 B^4: 432*(20870896098775127028064391823 + 14805085921696700978211294512*r2)
A^2 B^3: 32*(208227590008519280961024956851 + 149520045317884728395594000496*r2)
A^2 B^2: 96*(33900894581590513315581147227 + 24260249661175195443218571904*r2)
A^2 B^1: 576*(1117628240418368291811327518*r2 + 1687828080771338827995862759)
A^2 B^0: 16*(4378146028294390479489360528*r2 + 8917542756805222711060629601)
A^1 B^12: 1154108683739932651626496*(132*r2 + 193)
A^1 B^11: 2291712*(1295758642231169750324*r2 + 1858703860043679864559)
A^1 B^10: 3072*(8999796603584110361356792*r2 + 12753050751290428334259033)
A^1 B^9: 1024*(217569569779926737723380055 + 154432427036882012433151512*r2)
A^1 B^8: 18432*(46376792136874758029155265 + 32936299384607485295956993*r2)
A^1 B^7: 1152*(1998543018233288580842713629 + 1415214997302505739970256228*r2)
A^1 B^6: 1344*(2326110301474635304073505528*r2 + 3297316069512658847624773847)
A^1 B^5: 4608*(935165849699737428756124919*r2 + 1327543332997627294482465703)
A^1 B^4: 576*(7362005847608630402485846504*r2 + 10412834069492789459677186863)
A^1 B^3: 128*(31839111522298448724909424111 + 22697565922064393198013160968*r2)
A^1 B^2: 1536*(1193142236447723260618469987 + 852529327420531261242476092*r2)
A^1 B^1: 768*(446338342407482389899252662*r2 + 649645946955907639782762165)
A^1 B^0: 64*(585971471878420621284523848*r2 + 1013608864064229550761089185)
A^0 B^12: 417135567461825386332160*(132*r2 + 193)
A^0 B^11: 48125952*(25898000869297868748*r2 + 37321098179636078131)
A^0 B^10: 3072*(3925692502602617565408144*r2 + 5593518080219629132974995)
A^0 B^9: 1024*(65703386455516276227607008*r2 + 92951038861513815191351117)
A^0 B^8: 41472*(8289073312000914364087283 + 5876231575764424986106344*r2)
A^0 B^7: 1152*(744886085795455375032904565 + 527756184655832439956457372*r2)
A^0 B^6: 1344*(801016638600294270955353504*r2 + 1133317476224329507679552585)
A^0 B^5: 3456*(396060830417214294566608740*r2 + 561434210712512240520281717)
A^0 B^4: 4032*(308590435408595124679088592*r2 + 436942678344712061914814663)
A^0 B^3: 128*(8696078332722092266214016751 + 6172649304842554723976221104*r2)
A^0 B^2: 1152*(404761528106382220615302149 + 288371755883555236394391072*r2)
A^0 B^1: 768*(107087756649665564136357690*r2 + 153176873601604214857713739)
A^0 B^0: 64*(137521187537972417623016304*r2 + 217304961552291411717550225)

SMALL-RADIUS BRIDGE STURM DATA
For each non-tail case, F is the cleared saddle polynomial and P is the cleared
direct polynomial.  The displayed interval I contains one root of F and no root
 of P; the midpoint value P(mid) is positive.  Thus P is positive at the saddle
root.
t=1, n=5, s=1, I=[1/10,1/5]
F(z) = 168*z**3 + 40*z**2 - 1
P(z) = 72*z**2 + 7*z - 1
P(mid) = 167/100
t=1, n=5, s=2, tail: z=0, P(0)=2
t=2, n=9, s=1, I=[1/10,1/5]
F(z) = 336*z**3 + 88*z**2 - 7*z - 3
P(z) = 56*z**2*(72*z**2 + 7*z - 1)
P(mid) = 10521/5000
t=2, n=9, s=2, I=[1/8,3/20]
F(z) = 2*(168*z**3 + 40*z**2 - 1)
P(z) = 4800*z**4 + 2016*z**3 + 145*z**2 - 14*z - 3
P(mid) = 610939/128000
t=2, n=9, s=3, I=[1/20,1/10]
F(z) = 336*z**3 + 72*z**2 + 7*z - 1
P(z) = 4480*z**4 + 4200*z**3 + 801*z**2 + 42*z - 3
P(mid) = 26277/4000
t=2, n=9, s=4, tail: z=0, P(0)=6
t=3, n=13, s=1, I=[1/10,1/5]
F(z) = 504*z**3 + 136*z**2 - 14*z - 5
P(z) = 3520*z**4*(72*z**2 + 7*z - 1)
P(mid) = 148797/50000
t=3, n=13, s=2, I=[3/20,1/5]
F(z) = 504*z**3 + 128*z**2 - 7*z - 4
P(z) = 80*z**2*(3840*z**4 + 1512*z**3 + 121*z**2 - 14*z - 3)
P(mid) = 976129/40000
t=3, n=13, s=3, I=[1/8,3/20]
F(z) = 3*(168*z**3 + 40*z**2 - 1)
P(z) = 301056*z**6 + 241920*z**5 + 52488*z**4 + 3367*z**3 - 363*z**2 - 63*z - 5
P(mid) = 669237673/32000000
t=3, n=13, s=4, I=[3/40,1/10]
F(z) = 504*z**3 + 112*z**2 + 7*z - 2
P(z) = 4*(64512*z**6 + 87808*z**5 + 32480*z**4 + 5061*z**3 + 243*z**2 - 21*z - 3)
P(mid) = 715952407/64000000
t=3, n=13, s=5, I=[1/40,1/20]
F(z) = 504*z**3 + 104*z**2 + 14*z - 1
P(z) = 10*(19712*z**6 + 42336*z**5 + 23912*z**4 + 5635*z**3 + 609*z**2 + 21*z - 1)
P(mid) = 1015342823/102400000
t=3, n=13, s=6, tail: z=0, P(0)=20
t=3, n=14, s=1, I=[1/10,1/5]
F(z) = 560*z**3 + 152*z**2 - 14*z - 5
P(z) = 4224*z**4*(80*z**2 + 7*z - 1)
P(mid) = 98901/25000
t=3, n=14, s=2, I=[1/8,3/20]
F(z) = 560*z**3 + 144*z**2 - 7*z - 4
P(z) = 88*z**2*(4800*z**4 + 1680*z**3 + 129*z**2 - 14*z - 3)
P(mid) = 122562473/20480000
t=3, n=14, s=3, I=[9/80,1/8]
F(z) = 560*z**3 + 136*z**2 - 3
P(z) = 430080*z**6 + 302400*z**5 + 61200*z**4 + 3703*z**3 - 387*z**2 - 63*z - 5
P(mid) = 14383630577/1638400000
t=3, n=14, s=4, I=[3/40,1/10]
F(z) = 560*z**3 + 128*z**2 + 7*z - 2
P(z) = 12*(32256*z**6 + 37632*z**5 + 12660*z**4 + 1855*z**3 + 85*z**2 - 7*z - 1)
P(mid) = 1890180891/128000000
t=3, n=14, s=5, I=[1/40,1/20]
F(z) = 560*z**3 + 120*z**2 + 14*z - 1
P(z) = 2*(157696*z**6 + 282240*z**5 + 141120*z**4 + 30975*z**3 + 3165*z**2 + 105*z - 5)
P(mid) = 340618729/32000000
t=3, n=14, s=6, tail: z=0, P(0)=20
\end{verbatim}
}

\end{document}
