# Supplementary material for: The Quantum Hamming Bound in Arbitrary Local Dimension
Source: arXiv:2606.22538 source file (2026-10-05)
Supplement: Supplementary file 2 [file certificate_appendix.tex]

\smsection{Exact coefficient and Sturm data}{sec:S-cert-appendix}

This final appendix contains the finite exact-algebra data invoked in four
places: the high-alphabet endpoint and scalar checks of Sec.~\ref{sec:S3}, the
filtered-defect factorization of Sec.~\ref{sec:S6}, the qutrit long-range scalar
comparison of Sec.~\ref{sec:S4}, and the small-radius bridge Sturm checks of
Sec.~\ref{sec:S7}.  The symbols in each block are the quantities already defined
in the corresponding section; the block header repeats the substitutions used
there.  The displayed data are exact algebraic outputs after those
substitutions, and each displayed entry is read by integer arithmetic,
coefficientwise positivity, Bernstein coefficient nonnegativity, or Sturm
isolation on explicit rational intervals.  No numerical approximation is used in
reading the signs.  Thus the entry point is contained in the printed
certificate: start from the named formulae in the indicated section, make the
substitutions in the block header, clear only the denominators listed in the
ledger, and read the printed coefficients by the stated sign rule.

\noindent\textbf{Index of printed data.}
The high-alphabet entries correspond to the endpoint formulae and scalar
Jacobi inequality in Sec.~\ref{sec:S3}; their signs are read from rational
factorization and coefficient positivity.  The filtered bridge factorization
corresponds to \eqref{eq:S-filter-defect-def},
\eqref{eq:S-two-var-intersection}, and
\eqref{eq:S-eliminate-Ctplus}--\eqref{eq:S-eliminate-Ctminus}; its sign
information is the quotient-remainder identity modulo the saddle residual,
together with the denominator ledger.  The qutrit long-range entries correspond
to the scalar comparisons after \eqref{eq:S-qutrit-chain}--
\eqref{eq:S-qutrit-R2}; their signs are read coefficientwise in
\(\mathbb Q(\sqrt2)\) after the displayed substitutions.  The small bridge
entries correspond to \eqref{eq:S-saddle} and \eqref{eq:S-direct-cleared};
their signs are read by Sturm isolation on the printed rational intervals and
midpoint signs.

\noindent\textbf{Sign conventions.}
In the algebraic coefficient blocks, `r2' denotes \(\sqrt2\).  A coefficient of
the form \(c(a-b\sqrt2)\) is positive because the exact integer comparison
\(a^2>2b^2\) holds for that entry; coefficients of the form \(a+b\sqrt2\) with
\(a,b>0\) are positive.  In the bridge-factorization block, \(\Phi\) is the
filtered shell defect of Sec.~\ref{sec:S6} and \(Sres\) is the saddle residual
\(\mathcal S\).  The displayed quotient-remainder identity is obtained by the
four algebraic operations listed in Sec.~\ref{sec:S6}: expand the adjacency
formula, substitute the two-variable intersection generator, collect the four
adjacent coefficients of \(G\), and eliminate the outer two coefficients.  It
states that, after setting \(Sres=0\), the only remaining sign-bearing factor is
the two-coefficient bridge expression used in Sec.~\ref{sec:S6}.  The
denominator ledger lists every factor cleared in obtaining this identity, so
the positive prefactor in Sec.~\ref{sec:S6} contains no hidden sign-dependent
term.

\noindent\textbf{Bridge-factorization ledger.}
For the bridge factorization, the adjacent-coefficient eliminations
\eqref{eq:S-eliminate-Ctplus}--\eqref{eq:S-eliminate-Ctminus}, the saddle
substitution \eqref{eq:S-bridge-N-explicit}, and the remainder ledger
\eqref{eq:S-filter-remainder-ledger}--\eqref{eq:S-filter-coefficient-ledger}
are identities in the displayed variables.  The small-radius rows at the end of
this appendix give the corresponding exact Sturm output for the finite
exceptional bridge triples.

{\scriptsize
\begin{verbatim}
HIGH-ALPHABET ALGEBRAIC DATA
endpoint s=1 gap = (Q^2 - 16*Q + 16)/(2*(3*Q - 4)^2)
endpoint s=2 gap = (7*Q - 8)*(7*Q^3 - 72*Q^2 + 128*Q - 64)/(2*(3*Q - 4)^4)
Jacobi scalar numerator = 15201000*z^4 + 1147275*z^3 + 22440*z^2 - 575*z + 4
quadratic discriminant = -28415
terminal r=1 gap numerator = 28*t^2 + 220*t + 495

FILTERED DEFECT FACTORIZATION DATA
Variables: A=1+7z, B=8z^2, N=n-1-s, Sres=t-s*A/(1+A)-N*B/(1+B).
This block is only for the non-tail bridge case s<2t, z>0.  The endpoint
s=2t is checked separately in the text and never divides by B.

Denominator and sign ledger.
(1) Two-variable intersection terms are first written with binomial factors
    binom(s,a) binom(N,m-a), with 0<=a<=s and 0<=m-a<=N.  All such factors are
    nonnegative integers; in the support terms used for C_{t-1}^G at least one
    term is strictly positive.
(2) The adjacent-coefficient eliminations clear only t+1, t, A, B, and
    s+N-t+1.  In the bridge range these are positive: t>=1, A=1+7z>0,
    B=8z^2>0, and s+N-t+1=n-t>0.
(3) The saddle substitution clears the positive factors (2+7z), (1+8z^2), and
    their powers.  The residual factor
       t(2+7z)-s(1+7z)=8z^2(2+7z)N/(1+8z^2)
    is positive for z>0 and N>0.
(4) The global denominator D_+ is the product of the cleared factors in (1)--(3)
    and the positive powers displayed in the proof.  No factor whose sign depends
    on z,s,t,n is hidden in C_{n,t,s}.

After the T/T^2 expansion, two-variable intersection substitution, and adjacent-
coefficient eliminations, the exact quotient-remainder identity is
D_+ Phi / M = ((2s+1)+Sres*R_t) C_t^G
              + (-(2s-1-7z)+Sres*R_{t-1}) C_{t-1}^G.
Remainder modulo Sres:
Rem_{Sres}(D_+ Phi / M) = (2s+1) C_t^G - (2s-1-7z) C_{t-1}^G.
The same exact simplification gives the divisibility identity:
D_+ Phi - M*((2s+1) C_t^G - (2s-1-7z) C_{t-1}^G)
is divisible by Sres.
The positive factor used in the proof is
M = C^+_{n,t,s} C_{t-1}^G (1+7z)^(s-1) (8z^2)^(t-1) (2+7z)^s
    *(1+8z^2)^(N+1)*(t(2+7z)-s(1+7z)) / D_+,
where C^+_{n,t,s}>0 is precisely the product of the positive integer and rational
normalizers listed in (1)--(4).

QUTRIT LONG-RANGE SCALAR COEFFICIENT DATA
Variables A,B are nonnegative integers after s=2(A+1) or 2(A+1)+1
and t=A+B+2; r2 denotes sqrt(2).

[even rational residual numerator]
N_even_1: terms=28, total_degree=6
A^6 B^0: -336200*(-39979 + 22554*r2)
A^5 B^1: -2460*(-35817651 + 9160864*r2)
A^5 B^0: -2460*(-81240359 + 31894582*r2)
A^4 B^2: 12*(9037614379*r2 + 25404327941)
A^4 B^1: 36*(4173705749*r2 + 34857014947)
A^4 B^0: -12*(-111539524531 + 10400588668*r2)
A^3 B^3: 2*(403732016693 + 327434456532*r2)
A^3 B^2: 6*(492547791278*r2 + 729479094677)
A^3 B^1: 6*(668604292760*r2 + 1368660116403)
A^3 B^0: 2*(727470411546*r2 + 2680812514471)
A^2 B^4: 6*(252157071747 + 214884571564*r2)
A^2 B^3: 6*(1702501076659 + 1439641092442*r2)
A^2 B^2: 9*(2907233063149 + 2333583033198*r2)
A^2 B^1: 24*(1268758979973 + 903011151704*r2)
A^2 B^0: 3*(2601525082306*r2 + 4577159115505)
A^1 B^5: 6*(266102691775 + 188920298384*r2)
A^1 B^4: 18*(738736078971 + 550264007570*r2)
A^1 B^3: 6*(7352504130023 + 5672406040843*r2)
A^1 B^2: 6*(12205571476838 + 9542180314933*r2)
A^1 B^1: 18*(3403263341668 + 2603273237787*r2)
A^1 B^0: 6*(3474485005243 + 2462927925701*r2)
A^0 B^6: 62613138466*(6*r2 + 11)
A^0 B^5: 6*(671754869144*r2 + 1154900668361)
A^0 B^4: 12*(1485310075195*r2 + 2399856769221)
A^0 B^3: 2*(20755134825759*r2 + 31684675862593)
A^0 B^2: 3*(17855352994772*r2 + 26017348611749)
A^0 B^1: 6*(6031328799979*r2 + 8535990786165)
A^0 B^0: 14067440825945 + 9947822141892*r2

[even squared residual numerator]
N_even_2: terms=91, total_degree=12
A^12 B^0: -113030440000*(-2615686273 + 1803372732*r2)
A^11 B^1: -413526000*(-6635926244061 + 4386086622028*r2)
A^11 B^0: -413526000*(-18001634222765 + 12119426894644*r2)
A^10 B^2: -4034400*(-2505926412997411 + 1416700464096403*r2)
A^10 B^1: -6051600*(-9946899043778597 + 5999220013133906*r2)
A^10 B^0: -2017200*(-41801507425264453 + 26500854913328248*r2)
A^9 B^3: -45920*(-429078489051679775 + 63316504165065198*r2)
A^9 B^2: -19680*(-10215357731190363068 + 3312612465235573945*r2)
A^9 B^1: -9840*(-61898580762905094285 + 27785886655172288432*r2)
A^9 B^0: -3280*(-176504974133128700249 + 94392327861986516706*r2)
A^8 B^4: 144*(283184129973136863372 + 268070506187576311277*r2)
A^8 B^3: 144*(1804386923022846108101*r2 + 3637564946158481643308)
A^8 B^2: 432*(816738941537943395583*r2 + 5209623230823612514447)
A^8 B^1: -144*(-28910689600452987654009 + 3190182780265620553721*r2)
A^8 B^0: -144*(-19767817888234617014077 + 6077591643050223960638*r2)
A^7 B^5: 36*(5318687380888712693759 + 5269220670172499203252*r2)
A^7 B^4: 108*(20995636080754563346333 + 19087526252588566101144*r2)
A^7 B^3: 144*(69308384539839235112485 + 54278783874546921769061*r2)
A^7 B^2: 288*(44745599998766725524595*r2 + 76073066184264006193541)
A^7 B^1: 108*(77687747520173289978208*r2 + 230393822415429443454247)
A^7 B^0: 36*(24153003049201748040712*r2 + 328756510176193657172585)
A^6 B^6: 168*(4730851408106400198571 + 3602655985530256539726*r2)
A^6 B^5: 252*(40220340975645197222191 + 31455791355289870896676*r2)
A^6 B^4: 252*(198486173956659547228659 + 157468200602359284009190*r2)
A^6 B^3: 2184*(58143152444248956746734 + 45529229845093554007659*r2)
A^6 B^2: 504*(357087888862194175114294 + 261540258328853939851417*r2)
A^6 B^1: 252*(342026663040070671624866*r2 + 550294982181359537853561)
A^6 B^0: 420*(49045900529624544349980*r2 + 110696700949524197995789)
A^5 B^7: 36*(41304067773912214936700*r2 + 59915845612400941823493)
A^5 B^6: 252*(86288453816870842477256*r2 + 122680078248399861596897)
A^5 B^5: 5292*(33813535684517847735653 + 24271622652181115203698*r2)
A^5 B^4: 252*(2194778043487717044065367 + 1605871818655582566161780*r2)
A^5 B^3: 252*(3965082426396348066213557 + 2938185527141569188691136*r2)
A^5 B^2: 756*(1412578269456631262317081 + 1042154254853162670291228*r2)
A^5 B^1: 252*(2515149185994377936851959 + 1782511777299054569842106*r2)
A^5 B^0: 36*(2898482771366577834339320*r2 + 4552750831971815773753091)
A^4 B^8: 144*(18738129765611062855711*r2 + 27210291317276812110110)
A^4 B^7: 108*(399978747411358034340500*r2 + 578862358383910834764147)
A^4 B^6: 1008*(287776444303737345137213*r2 + 414273945424575496749709)
A^4 B^5: 252*(4286773297636158988027828*r2 + 6123040755957939910892771)
A^4 B^4: 189*(18385980204927718523016109 + 13002017704932415673263108*r2)
A^4 B^3: 504*(9744192878565242682461924 + 6964185235913188544595451*r2)
A^4 B^2: 126*(33934856477421201148319089 + 24428099932625234845578872*r2)
A^4 B^1: 216*(9767921750343846553408480 + 7003857234144878033623041*r2)
A^4 B^0: 9*(35271865225359810908404508*r2 + 50625080430393222336197065)
A^3 B^9: 4*(850077717065833117059036*r2 + 1203465918545112742854793)
A^3 B^8: 36*(1647310844531930025954256*r2 + 2341930959816771927076105)
A^3 B^7: 180*(2476860307327956422725724*r2 + 3532165091857233082707447)
A^3 B^6: 84*(22742081329621384439367330*r2 + 32483554926118463127603317)
A^3 B^5: 102564*(50373187994659744757267*r2 + 71928372834323288322740)
A^3 B^4: 252*(36413231530254015350682343*r2 + 51867921508779812592600477)
A^3 B^3: 84*(127692376944846481721056062*r2 + 181100821242491878210101061)
A^3 B^2: 36*(312243865134231350811104569 + 221273370182405148522290620*r2)
A^3 B^1: 36*(133284446064609192960923595 + 94725528303978580897529911*r2)
A^3 B^0: 4*(226245785222524119216677606 + 159999008135360002203591657*r2)
A^2 B^10: 168*(23057736451867509447717 + 16551450378593099321806*r2)
A^2 B^9: 12*(6138113952830822346166829 + 4388967812841374397875372*r2)
A^2 B^8: 216*(2852968378524820019141300 + 2032323028637545968301917*r2)
A^2 B^7: 36*(83327921911385242755257661 + 59146690859202955056728284*r2)
A^2 B^6: 504*(18721350759914030380125575 + 13246441917375759387545141*r2)
A^2 B^5: 756*(18744463280405535801081897*r2 + 26555841657908638629948418)
A^2 B^4: 126*(163948199667905842988277202*r2 + 232571707724360103168472815)
A^2 B^3: 252*(81142995511402776611475272*r2 + 115100151019495950553076723)
A^2 B^2: 108*(121899385697637265658665206*r2 + 172687964709661790445222373)
A^2 B^1: 12*(415002448173944870935273993*r2 + 586903150520444881939845771)
A^2 B^0: 6*(198012696826851508708180955 + 140019027247199972445704138*r2)
A^1 B^11: 4476*(414043701102967682993 + 294634297320734032156*r2)
A^1 B^10: 36*(1054462964505273052260557 + 751075425175256004605800*r2)
A^1 B^9: 24*(14494359680007010702412123 + 10328178005163747073440835*r2)
A^1 B^8: 72*(26210174848227573757351841 + 18671171111134810950746857*r2)
A^1 B^7: 1944*(3469938000017400086364963 + 2469551293213029260261429*r2)
A^1 B^6: 1008*(16569937927130274499943621 + 11775960130165638262412056*r2)
A^1 B^5: 252*(116104456726140623339522084 + 82375361562520439099380999*r2)
A^1 B^4: 108*(335949230116914806337481993 + 237972381092352635313841007*r2)
A^1 B^3: 36*(867470941568891892107761903 + 613739842150216284989259740*r2)
A^1 B^2: 12*(1047400401244924811446208762*r2 + 1481273662248857626323478567)
A^1 B^1: 36*(118329259667066012560245335*r2 + 167344437957716894171174182)
A^1 B^0: 12*(54308276342232245748490153*r2 + 76803589750908621736852907)
A^0 B^12: 2076877093820241107152*(132*r2 + 193)
A^0 B^11: 4476*(1354825608341835295096*r2 + 1965311355840683788453)
A^0 B^10: 12*(5061069074492189858136640*r2 + 7290841102118956281894627)
A^0 B^9: 8*(45573952609780065736057551*r2 + 65271709159639542035300386)
A^0 B^8: 72*(20314173734750236349045488*r2 + 28959810119672418310521595)
A^0 B^7: 72*(57417045071484985839257155*r2 + 81571616845119431753252298)
A^0 B^6: 336*(25140188502235560623747247*r2 + 35632642394215478396335784)
A^0 B^5: 36*(349431516265006389666180529*r2 + 494580376820935863227305678)
A^0 B^4: 45*(301283937015307473542869184*r2 + 426153076047830183051428677)
A^0 B^3: 8*(1823952030243027936580670245 + 1289747781988958198692311711*r2)
A^0 B^2: 6*(1241065219960218225993676735 + 877569490820033260377941212*r2)
A^0 B^1: 12*(190720982185184785396659333 + 134860166615347322394061895*r2)
A^0 B^0: 320452477350252257025435409 + 226594128868898674598496840*r2

[odd rational residual numerator]
N_odd_1: terms=35, total_degree=7
A^7 B^0: -5379200*(-39979 + 22554*r2)
A^6 B^1: -39360*(-35817651 + 9160864*r2)
A^6 B^0: -6560*(-519681941 + 250777020*r2)
A^5 B^2: 192*(9037614379*r2 + 25404327941)
A^5 B^1: -96*(-211307994455 + 12525212624*r2)
A^5 B^0: -48*(-491895442388 + 178524097707*r2)
A^4 B^3: 32*(403732016693 + 327434456532*r2)
A^4 B^2: 48*(738307424936*r2 + 1359151693981)
A^4 B^1: 24*(795845840236*r2 + 5270992372577)
A^4 B^0: -4*(-23301134988977 + 4843292117328*r2)
A^3 B^4: 96*(252157071747 + 214884571564*r2)
A^3 B^3: 16*(9245211296417 + 7723594531896*r2)
A^3 B^2: 72*(3362630580436*r2 + 5009919089375)
A^3 B^1: 12*(12659536451848*r2 + 36493747227745)
A^3 B^0: -6640*(-34296848539 + 976500438*r2)
A^2 B^5: 96*(266102691775 + 188920298384*r2)
A^2 B^4: 48*(4216468808089 + 3334489934180*r2)
A^2 B^3: 24*(26401349809135 + 21644617706808*r2)
A^2 B^2: 12*(84815014631593 + 62784667911020*r2)
A^2 B^1: 24*(18589371776624*r2 + 36816663102991)
A^2 B^0: 48*(1126009301997*r2 + 7197836045785)
A^1 B^6: 1001810215456*(6*r2 + 11)
A^1 B^5: 48*(1691167789508*r2 + 2618991918007)
A^1 B^4: 24*(22639375152467 + 16534575310318*r2)
A^1 B^3: 4*(297225577081805 + 232826352553812*r2)
A^1 B^2: 12*(120570170385899 + 91991696765848*r2)
A^1 B^1: 24*(24993670500146*r2 + 40705379835703)
A^1 B^0: 4*(24521570609040*r2 + 75314777715833)
A^0 B^6: 1518192430016*(6*r2 + 11)
A^0 B^5: 2016*(41659231488*r2 + 67836380219)
A^0 B^4: 48*(6545418635982*r2 + 9564582702265)
A^0 B^3: 8*(101807028998177 + 75539499390132*r2)
A^0 B^2: 216*(3792735551353 + 2867374806432*r2)
A^0 B^1: 48*(6446381663490*r2 + 9533017937939)
A^0 B^0: 8*(6702713012472*r2 + 14500604267753)

[odd squared residual numerator]
N_odd_2: terms=117, total_degree=14
A^14 B^0: -28935792640000*(-2615686273 + 1803372732*r2)
A^13 B^1: -105862656000*(-6635926244061 + 4386086622028*r2)
A^13 B^0: -17643776000*(-126119249810087 + 86056261995540*r2)
A^12 B^2: -1032806400*(-2505926412997411 + 1416700464096403*r2)
A^12 B^1: -258201600*(-71936142838463453 + 45800486956495284*r2)
A^12 B^0: -43033600*(-702187862215596541 + 471116048100314106*r2)
A^11 B^3: -11755520*(-429078489051679775 + 63316504165065198*r2)
A^11 B^2: -17633280*(-3520618489334445563 + 1636416997455429602*r2)
A^11 B^1: -1889280*(-120003957673216082327 + 71329721839997843120*r2)
A^11 B^0: -104960*(-2397371751216848747203 + 1563106155143226931152*r2)
A^10 B^4: 36864*(283184129973136863372 + 268070506187576311277*r2)
A^10 B^3: 4096*(6057712801233149916273*r2 + 31650533554986978039481)
A^10 B^2: -6144*(-115743405609284040143152 + 34443903338711688220417*r2)
A^10 B^1: -1536*(-1111565739474662148268557 + 580337540809741069767226*r2)
A^10 B^0: -256*(-5625672708746275543885385 + 3489952591986712064206491*r2)
A^9 B^5: 9216*(5318687380888712693759 + 5269220670172499203252*r2)
A^9 B^4: 4608*(87523302912015751353203 + 82366940814920126855628*r2)
A^9 B^3: 512*(1725611525591474026572204*r2 + 3486130281591525935991023)
A^9 B^2: -2304*(-2311136821414819417854663 + 141610547631809884223308*r2)
A^9 B^1: -192*(-46801104862637357390039153 + 18972064627410441694291908*r2)
A^9 B^0: -32*(-188376899087719384528351903 + 107029417933531807905025524*r2)
A^8 B^6: 43008*(4730851408106400198571 + 3602655985530256539726*r2)
A^8 B^5: 4608*(387420893104201542019327 + 327365560843862794312700*r2)
A^8 B^4: 6912*(999829850693008472608227 + 874652817216210809706200*r2)
A^8 B^3: 768*(14657284616287077435038916*r2 + 21771486349978884647389085)
A^8 B^2: 2304*(2635886859033713070626027*r2 + 12956041042213558107531994)
A^8 B^1: -864*(-41252245309948053208021817 + 9702534643533620795528252*r2)
A^8 B^0: -48*(-400161674462061024333110123 + 194226036112752253289955072*r2)
A^7 B^7: 9216*(41304067773912214936700*r2 + 59915845612400941823493)
A^7 B^6: 10752*(536561930982924026250331 + 386843760152336087760132*r2)
A^7 B^5: 18432*(1419230270115310700305357 + 1096872056060669066636981*r2)
A^7 B^4: 145152*(462083142730117742959241 + 376211932853086724256228*r2)
A^7 B^3: 192*(577609167996352631151905639 + 429135494147341203148211604*r2)
A^7 B^2: 288*(197436515271575927102478676*r2 + 458941201531479003252827099)
A^7 B^1: -288*(-389022158153812069961138271 + 8326887478730142839738512*r2)
A^7 B^0: -384*(-124913213694553264554117841 + 45290437550390254954803738*r2)
A^6 B^8: 36864*(18738129765611062855711*r2 + 27210291317276812110110)
A^6 B^7: 4608*(1837784295768138806349540*r2 + 2666346111366780771184547)
A^6 B^6: 5376*(8777291232880139559633480*r2 + 12463599326633916998030207)
A^6 B^5: 16128*(12976987368690503468799125 + 9544543524913295703859828*r2)
A^6 B^4: 24192*(16859482156961346200262691 + 12992887113296071718020078*r2)
A^6 B^3: 672*(775810771673375880147698995 + 586818715781554148397721812*r2)
A^6 B^2: 1008*(266086073676538909306714768*r2 + 457962068320846738623309449)
A^6 B^1: 576*(100142955206814639977714244*r2 + 496930371156084804027810167)
A^6 B^0: -384*(-249603445521418361990736103 + 49352690680174774877232846*r2)
A^5 B^9: 1024*(850077717065833117059036*r2 + 1203465918545112742854793)
A^5 B^8: 4608*(2637319857151799481919316*r2 + 3781499249266126209735289)
A^5 B^7: 13824*(5621320789127774297405076*r2 + 8106481837443316170770723)
A^5 B^6: 5376*(55130139832313285070290844*r2 + 78893838995583204492872051)
A^5 B^5: 4032*(254460491893466177100027431 + 182311265526451900559985076*r2)
A^5 B^4: 6048*(270061732787986562777809365 + 200436213968294497823999572*r2)
A^5 B^3: 2688*(644073803367948345010836773 + 482362052441396345748404418*r2)
A^5 B^2: 288*(2845130893090348639831799048*r2 + 4294496246822568509320663207)
A^5 B^1: 3456*(67184463534832628837931254*r2 + 171245362372992789041563225)
A^5 B^0: -32*(-4833430828223802709652707033 + 17510301070184511747338040*r2)
A^4 B^10: 43008*(23057736451867509447717 + 16551450378593099321806*r2)
A^4 B^9: 3584*(4517536493035410818270027 + 3215295630968095443242076*r2)
A^4 B^8: 11520*(7430773520793837756760832*r2 + 10551497160311567679191395)
A^4 B^7: 2304*(166050741946986788013197588*r2 + 237674341504218425283675783)
A^4 B^6: 5376*(210183217381463559394626621*r2 + 300827150053047619549482710)
A^4 B^5: 2016*(1602570645721209449260692187 + 1133895450034835949929946812*r2)
A^4 B^4: 3024*(1451754744906827199798399879 + 1052061100889083243444855168*r2)
A^4 B^3: 672*(5990471308974055920688699043 + 4413770753091279169581979752*r2)
A^4 B^2: 8064*(212784158444989452719545862*r2 + 304262566963716193390353229)
A^4 B^1: 96*(5291292660616931104211632280*r2 + 10001040658107021147705487497)
A^4 B^0: 64*(600823682950666371552401532*r2 + 3119626571682931840636739711)
A^3 B^11: 1145856*(414043701102967682993 + 294634297320734032156*r2)
A^3 B^10: 1536*(5989997892519431737311779 + 4284868689515774881841556*r2)
A^3 B^9: 1024*(79647995636367892229408701 + 56824284346777924940301342*r2)
A^3 B^8: 2304*(189536784197091744565575409 + 134285447113226411173482764*r2)
A^3 B^7: 576*(1899071763874229198662998420*r2 + 2700513814159638078896284231)
A^3 B^6: 672*(3991962521108123064483496188*r2 + 5696527738622189070037664761)
A^3 B^5: 2016*(2298741136590209047319434256*r2 + 3264366402016706199956832871)
A^3 B^4: 864*(9099762053649461883349646357 + 6502904794894414806428103748*r2)
A^3 B^3: 768*(8347015086075617016060769519 + 6059875522823455153176919905*r2)
A^3 B^2: 96*(36003572904163194253431856961 + 25661865083616065680741872016*r2)
A^3 B^1: 768*(928585091523801035406490599*r2 + 1511660385270349647676290647)
A^3 B^0: 128*(563467479942100164381996027*r2 + 1554176615884732648328573101)
A^2 B^12: 531680536017981723430912*(132*r2 + 193)
A^2 B^11: 572928*(3285051879005741449196*r2 + 4677599674035926138275)
A^2 B^10: 2304*(12945768591179205538458017 + 9196741373648604931622752*r2)
A^2 B^9: 256*(765356382636574858592379209 + 545184793426701451642902936*r2)
A^2 B^8: 1152*(739654052061166082372950811 + 525360640821253263702962896*r2)
A^2 B^7: 864*(2105277762266194604445765972*r2 + 2980166446088455938081022603)
A^2 B^6: 336*(11543638128722977142073318144*r2 + 16412954643674393832751039625)
A^2 B^5: 1440*(4105231672438225358475946732*r2 + 5833811134277476244774731883)
A^2 B^4: 432*(20870896098775127028064391823 + 14805085921696700978211294512*r2)
A^2 B^3: 32*(208227590008519280961024956851 + 149520045317884728395594000496*r2)
A^2 B^2: 96*(33900894581590513315581147227 + 24260249661175195443218571904*r2)
A^2 B^1: 576*(1117628240418368291811327518*r2 + 1687828080771338827995862759)
A^2 B^0: 16*(4378146028294390479489360528*r2 + 8917542756805222711060629601)
A^1 B^12: 1154108683739932651626496*(132*r2 + 193)
A^1 B^11: 2291712*(1295758642231169750324*r2 + 1858703860043679864559)
A^1 B^10: 3072*(8999796603584110361356792*r2 + 12753050751290428334259033)
A^1 B^9: 1024*(217569569779926737723380055 + 154432427036882012433151512*r2)
A^1 B^8: 18432*(46376792136874758029155265 + 32936299384607485295956993*r2)
A^1 B^7: 1152*(1998543018233288580842713629 + 1415214997302505739970256228*r2)
A^1 B^6: 1344*(2326110301474635304073505528*r2 + 3297316069512658847624773847)
A^1 B^5: 4608*(935165849699737428756124919*r2 + 1327543332997627294482465703)
A^1 B^4: 576*(7362005847608630402485846504*r2 + 10412834069492789459677186863)
A^1 B^3: 128*(31839111522298448724909424111 + 22697565922064393198013160968*r2)
A^1 B^2: 1536*(1193142236447723260618469987 + 852529327420531261242476092*r2)
A^1 B^1: 768*(446338342407482389899252662*r2 + 649645946955907639782762165)
A^1 B^0: 64*(585971471878420621284523848*r2 + 1013608864064229550761089185)
A^0 B^12: 417135567461825386332160*(132*r2 + 193)
A^0 B^11: 48125952*(25898000869297868748*r2 + 37321098179636078131)
A^0 B^10: 3072*(3925692502602617565408144*r2 + 5593518080219629132974995)
A^0 B^9: 1024*(65703386455516276227607008*r2 + 92951038861513815191351117)
A^0 B^8: 41472*(8289073312000914364087283 + 5876231575764424986106344*r2)
A^0 B^7: 1152*(744886085795455375032904565 + 527756184655832439956457372*r2)
A^0 B^6: 1344*(801016638600294270955353504*r2 + 1133317476224329507679552585)
A^0 B^5: 3456*(396060830417214294566608740*r2 + 561434210712512240520281717)
A^0 B^4: 4032*(308590435408595124679088592*r2 + 436942678344712061914814663)
A^0 B^3: 128*(8696078332722092266214016751 + 6172649304842554723976221104*r2)
A^0 B^2: 1152*(404761528106382220615302149 + 288371755883555236394391072*r2)
A^0 B^1: 768*(107087756649665564136357690*r2 + 153176873601604214857713739)
A^0 B^0: 64*(137521187537972417623016304*r2 + 217304961552291411717550225)

SMALL-RADIUS BRIDGE STURM DATA
For each non-tail case, F is the cleared saddle polynomial and P is the cleared
direct polynomial.  The displayed interval I contains one root of F and no root
 of P; the midpoint value P(mid) is positive.  Thus P is positive at the saddle
root.
t=1, n=5, s=1, I=[1/10,1/5]
F(z) = 168*z**3 + 40*z**2 - 1
P(z) = 72*z**2 + 7*z - 1
P(mid) = 167/100
t=1, n=5, s=2, tail: z=0, P(0)=2
t=2, n=9, s=1, I=[1/10,1/5]
F(z) = 336*z**3 + 88*z**2 - 7*z - 3
P(z) = 56*z**2*(72*z**2 + 7*z - 1)
P(mid) = 10521/5000
t=2, n=9, s=2, I=[1/8,3/20]
F(z) = 2*(168*z**3 + 40*z**2 - 1)
P(z) = 4800*z**4 + 2016*z**3 + 145*z**2 - 14*z - 3
P(mid) = 610939/128000
t=2, n=9, s=3, I=[1/20,1/10]
F(z) = 336*z**3 + 72*z**2 + 7*z - 1
P(z) = 4480*z**4 + 4200*z**3 + 801*z**2 + 42*z - 3
P(mid) = 26277/4000
t=2, n=9, s=4, tail: z=0, P(0)=6
t=3, n=13, s=1, I=[1/10,1/5]
F(z) = 504*z**3 + 136*z**2 - 14*z - 5
P(z) = 3520*z**4*(72*z**2 + 7*z - 1)
P(mid) = 148797/50000
t=3, n=13, s=2, I=[3/20,1/5]
F(z) = 504*z**3 + 128*z**2 - 7*z - 4
P(z) = 80*z**2*(3840*z**4 + 1512*z**3 + 121*z**2 - 14*z - 3)
P(mid) = 976129/40000
t=3, n=13, s=3, I=[1/8,3/20]
F(z) = 3*(168*z**3 + 40*z**2 - 1)
P(z) = 301056*z**6 + 241920*z**5 + 52488*z**4 + 3367*z**3 - 363*z**2 - 63*z - 5
P(mid) = 669237673/32000000
t=3, n=13, s=4, I=[3/40,1/10]
F(z) = 504*z**3 + 112*z**2 + 7*z - 2
P(z) = 4*(64512*z**6 + 87808*z**5 + 32480*z**4 + 5061*z**3 + 243*z**2 - 21*z - 3)
P(mid) = 715952407/64000000
t=3, n=13, s=5, I=[1/40,1/20]
F(z) = 504*z**3 + 104*z**2 + 14*z - 1
P(z) = 10*(19712*z**6 + 42336*z**5 + 23912*z**4 + 5635*z**3 + 609*z**2 + 21*z - 1)
P(mid) = 1015342823/102400000
t=3, n=13, s=6, tail: z=0, P(0)=20
t=3, n=14, s=1, I=[1/10,1/5]
F(z) = 560*z**3 + 152*z**2 - 14*z - 5
P(z) = 4224*z**4*(80*z**2 + 7*z - 1)
P(mid) = 98901/25000
t=3, n=14, s=2, I=[1/8,3/20]
F(z) = 560*z**3 + 144*z**2 - 7*z - 4
P(z) = 88*z**2*(4800*z**4 + 1680*z**3 + 129*z**2 - 14*z - 3)
P(mid) = 122562473/20480000
t=3, n=14, s=3, I=[9/80,1/8]
F(z) = 560*z**3 + 136*z**2 - 3
P(z) = 430080*z**6 + 302400*z**5 + 61200*z**4 + 3703*z**3 - 387*z**2 - 63*z - 5
P(mid) = 14383630577/1638400000
t=3, n=14, s=4, I=[3/40,1/10]
F(z) = 560*z**3 + 128*z**2 + 7*z - 2
P(z) = 12*(32256*z**6 + 37632*z**5 + 12660*z**4 + 1855*z**3 + 85*z**2 - 7*z - 1)
P(mid) = 1890180891/128000000
t=3, n=14, s=5, I=[1/40,1/20]
F(z) = 560*z**3 + 120*z**2 + 14*z - 1
P(z) = 2*(157696*z**6 + 282240*z**5 + 141120*z**4 + 30975*z**3 + 3165*z**2 + 105*z - 5)
P(mid) = 340618729/32000000
t=3, n=14, s=6, tail: z=0, P(0)=20
\end{verbatim}
}
